# Supplementary material for: Panel Data Analysis with Heterogeneous Dynamics
Source: arXiv:1803.09452 ancillary file (2019-01-15)
Supplement: Supplementary file 1 [file supplement.pdf]

# Supplementary Appendix of "Panel Data Analysis with Heterogeneous Dynamics"

Ryo Okui* and Takahide Yanagi†

January, 2019

This supplement contains remarks, extensions, mathematical proofs, simulations, and empirical results omitted from the main text. Appendix B explains the formula of third-order jackknife (TOJ) bias correction. Appendix C develops testing procedures for parametric specifications based on the functional CLT in the main body. Appendix D provides several other extensions. Appendix E includes mathematical proofs. Appendix F presents empirical applications for earnings dynamics and productivity dynamics. Appendix G contains additional Monte Carlo simulations.

## B Appendix: Third-order jackknife

This appendix explains the TOJ bias correction. While the TOJ is originally discussed in Dhaene and Jochmans (2015), we need to modify their formula to provide higher order bias correction in our context.

Suppose that $T$ is a multiple of six (see Dhaene and Jochmans, 2015 for the treatment of the case in which $T$ is not a multiple of six). The panel data are divided into three subpanels: $\{\{y_{it}\}_{i=1}^N\}_{t=1}^{T/3}$, $\{\{y_{it}\}_{i=1}^N\}_{t=T/3+1}^{2T/3}$, and $\{\{y_{it}\}_{i=1}^N\}_{t=2T/3+1}^{T}$. Let $\hat{S}^{(3,1)}$, $\hat{S}^{(3,2)}$, and $\hat{S}^{(3,3)}$ be the estimators of $S$ computed from each of these three subpanels.

*NYU Shanghai, 1555 Century Avenue, Pudong, Shanghai, China, 200122; and Department of Economics, University of Gothenburg, P.O. Box 640, SE-405 30 Gothenburg, Sweden. Tel: +86-21-2059-6157. Email: okui.ryo.3@gmail.com

†Graduate School of Economics, Kyoto University, Yoshida Honmachi, Sakyo, Kyoto, 606-8501, Japan. Email: yanagi@econ.kyoto-u.ac.jp

Following Dhaene and Jochmans (2015), the TOJ bias-corrected estimator has the following form:

$$(1+a_2+a_3)\hat{S} - a_2\left(\frac{\hat{S}^{(1)}+\hat{S}^{(2)}}{2}\right) - a_3\left(\frac{\hat{S}^{(3,1)}+\hat{S}^{(3,2)}+\hat{S}^{(3,3)}}{3}\right),$$

where $a_2$ and $a_3$ are constants, which are set to eliminate the first-order bias and the second-order bias of the estimator $\hat{S}$. To determine the values of $a_2$ and $a_3$, we observe the following expansion of $\hat{S}$ shown in the proof of Theorem 4:

$$\hat{S} = S + \frac{B}{T} + O_p\left(\frac{1}{T^{3/2}}\right) + o_p\left(\frac{1}{T}\right) + O_p\left(\frac{1}{\sqrt{N}}\right).$$

Accordingly, if we assume that the third and fourth terms in the right-hand side can be written as $C/T^{3/2} + o_p(T^{-3/2})$ for a constant $C$, we can eliminate the first- and second-order bias of $\hat{H}$ by setting

$$\left(\frac{1+a_2+a_3}{T} - \frac{a_2}{T/2} - \frac{a_3}{T/3}\right)B = 0, \qquad \left(\frac{1+a_2+a_3}{T^{3/2}} - \frac{a_2}{(T/2)^{3/2}} - \frac{a_3}{(T/3)^{3/2}}\right)C = 0.$$

Solving these equations, we obtain

$$a_2 = 1 - \frac{2(2^{3/2}-2)}{2\cdot 2^{3/2} - 3^{3/2} - 1} \approx 4.072, \qquad a_3 = \frac{2^{3/2}-2}{2\cdot 2^{3/2} - 3^{3/2} - 1} \approx -1.536.$$

Therefore, we have the following TOJ bias-corrected estimator for $S$:

$$\hat{S}^{TOJ} := 3.536\hat{H} - 4.072\left(\frac{\hat{S}^{(1)}+\hat{S}^{(2)}}{2}\right) + 1.536\left(\frac{\hat{S}^{(3,1)}+\hat{S}^{(3,2)}+\hat{S}^{(3,3)}}{3}\right).$$

This TOJ estimator differs from that in Dhaene and Jochmans (2015, page 1018). They consider cases that have no bias of order $T^{-3/2}$ and apply the TOJ to correct the bias of order $T^{-2}$.

## C Appendix: Testing parametric specifications

This appendix develops a testing procedure for hypotheses on parametric specifications of the distribution of $\xi_i = \mu_i$, $\gamma_{k,i}$, or $\rho_{k,i}$. The test is based on one-sample KS statistics computed from

the empirical distribution of $\hat{\xi}_i = \hat{\mu}_i$, $\hat{\gamma}_{k,i}$, or $\hat{\rho}_{k,i}$. We first consider the case for known distributions under the null hypothesis and then consider the case when it belongs to a parametric family under the null hypothesis with unknown parameters.

It is common to impose a parametric specification to model heterogeneous dynamics, and it is important to have a test for such a parametric specification. For example, Browning, Ejrnæs, and Alvarez (2010) develop a parametric model of heterogeneous income dynamics. Hsiao, Pesaran, and Tahmiscioglu (1999) consider random coefficients panel AR(1) models and impose parametric assumptions to implement a Bayesian procedure. Researchers can use our test to examine the validity of these parametric specifications.

We first consider the following hypotheses:

$$H_0 : P_0 = Q \quad \text{v.s.} \quad H_1 : P_0 \neq Q,$$

where $P_0 = P_0^{\xi}$ is the probability measure of $\xi_i$ and $Q$ is a known continuous distribution. Note that $Q$ cannot be a discrete distribution because our asymptotics are based on a continuous $\xi_i$.

Our test is based on one-sample KS statistic (Kolmogorov, 1933; Smirnov, 1944):

$$KS_1 := \sqrt{N} \left\| \mathbb{P}_N - Q \right\|_\infty = \sqrt{N} \sup_{f \in \mathcal{F}} \left| \mathbb{P}_N f - Qf \right|,$$

where $\mathbb{P}_N = \mathbb{P}_N^{\hat{\xi}}$ is the empirical distribution. The test statistic measures the distance between the empirical distribution and the null distribution. Note that $KS_1$ differs from the usual one-sample KS statistic in the sense that they are based on the empirical distributions of the estimator $\hat{\xi}_i$.

We derive the asymptotic distribution of $KS_1$ under $H_0$, utilizing Theorem 2. The following theorem presents the asymptotic null distribution.

**Theorem 9.** *Suppose that the assumptions in Theorem 2 hold. When $N, T \to \infty$ with $N^{3+\epsilon}/T^4 \to 0$ for some $\epsilon \in (0, 1/3)$, $KS_1$ converges in distribution to $\|\mathbb{G}_Q\|_\infty$ under $H_0$.*

*Proof.* The proof is almost identical to the proof of Corollary 19.21 in van der Vaart (1998). We first note that under $H_0$, $\sqrt{N}(\mathbb{P}_N - Q) \rightsquigarrow \mathbb{G}_Q$ in $\ell^\infty(\mathcal{F})$ given $N, T \to \infty$ with $N^{3+\epsilon}/T^4 \to 0$ by Theorem 2. Therefore, because the norm $\|\cdot\|_\infty$ for $D[-\infty, \infty]$, where $D[-\infty, \infty]$ is the class of all càdlàg functions from $[-\infty, \infty]$ into $\mathbb{R}$, is continuous with respect to the uniform norm, we have

$KS_1 \rightsquigarrow \|\mathbb{G}_Q\|_\infty$ under $H_0$ by the continuous mapping theorem. □

The asymptotic null distribution of $KS_1$ is the uniform norm of a Gaussian process. This asymptotic null distribution is identical to those of the usual one-sample KS statistics developed in Kolmogorov (1933) and Smirnov (1944) such that it is equivalent to that of the one-sample KS statistics based on the true $\xi_i = \mu_i$, $\gamma_{k,i}$, or $\rho_{k,i}$. This is because the estimation error in $\hat{\xi}_i = \hat{\mu}_i$, $\hat{\gamma}_{k,i}$, or $\hat{\rho}_{k,i}$ can be ignored asymptotically under the condition $N^{3+\epsilon}/T^4 \to 0$.

The asymptotic null distribution in the theorem is the same as that in Theorem 8 when we set $P_{0,(1)} = Q$. Hence, we can easily evaluate the asymptotic null distribution as in Theorem 8 and the critical value of our test are readily available.

Next, we consider testing a null hypothesis that the distribution belongs to a parametric family:

$$H_0 : P_0 = P_{\beta_0} \text{ for some } \beta_0 \in \mathbb{B} \quad \text{v.s.} \quad H_1 : P_0 \neq P_\beta \text{ for any } \beta \in \mathbb{B},$$

where $P_0 = P_0^\xi$ and $\{P_\beta : \beta \in \mathbb{B} \subset \mathbb{R}^K\}$ is a family of distributions indexed by a finite dimensional parameter $\beta$. Let $\hat{\beta}_{NT}$ be an estimator of $\beta_0$. The testing statistic is the modified KS statistic:

$$MKS := \sqrt{N} \sup_{f \in \mathcal{F}} \left| \mathbb{P}_N f - P_{\hat{\beta}_{NT}} f \right| = \sqrt{N} \sup_{a \in \mathbb{R}} \left| \mathbb{F}_N(a) - P_{\hat{\beta}_{NT}}(a) \right|.$$

For example, the test statistic for $H_0 : P_0^\mu = \mathcal{N}(E(\mu_i), var(\mu_i))$ is

$$\sqrt{N} \sup_{a \in \mathbb{R}} \left| \mathbb{F}_N^{\hat{\mu}}(a) - \Phi\left( \frac{a - \hat{\beta}_{NT}^{(1)}}{\sqrt{\hat{\beta}_{NT}^{(2)} - (\hat{\beta}_{NT}^{(1)})^2}} \right) \right|,$$

where $\hat{\beta}_{NT}^{(1)} = N^{-1} \sum_{i=1}^N \hat{\mu}_i$ and $\hat{\beta}_{NT}^{(2)} = N^{-1} \sum_{i=1}^N \hat{\mu}_i^2$ with $\beta_0^{(1)} = E(\mu_i)$ and $\beta_0^{(2)} = E(\mu_i^2)$.

To examine the asymptotic distribution of the statistic, we show the asymptotic law of $\sqrt{N}(\mathbb{P}_N - P_{\hat{\beta}_{NT}})$ in $\ell^\infty(\mathcal{F})$. The proof is analogous to Theorem 19.23 in van der Vaart (1998) and we thus omit it.

**Theorem 10.** *Suppose that the assumptions in Theorem 2 hold. Suppose that when $N, T \to \infty$ with $N^{3+\epsilon}/T^4 \to 0$ for some $\epsilon \in (0, 1/3)$, $\hat{\beta}_{NT}$ is an estimator depending on asymptotically linear*

*N and T with an influence function* $\psi_{\beta_0} := (\psi_{\beta_0,1}, \ldots, \psi_{\beta_0,K})^\top$*:*

$$\sqrt{N}(\hat{\beta}_{NT} - \beta_0) = \frac{1}{\sqrt{N}} \sum_{i=1}^{N} \psi_{\beta_0}(\zeta_i) + o_{P_{\beta_0}}(1), \tag{S1}$$

*where* $\zeta_i$ *is some i.i.d. sequence. Let the map* $\beta \mapsto P_\beta$ *from* $\mathbb{R}^K$ *to* $\ell^\infty(\mathcal{F})$ *be Fréchet differentiable at* $\beta_0$ *with the derivative* $\dot{P}_{\beta_0}$*. Then, when* $N, T \to \infty$ *with* $N^{3+\epsilon}/T^4 \to 0$*, it holds that* $\sqrt{N}(\mathbb{P}_N - P_{\hat{\beta}_{NT}})$ *weakly converges under* $\beta_0$ *in* $\ell^\infty(\mathcal{F})$ *to the process* $f \mapsto \mathbb{G}_{P_{\beta_0}} f - \mathbb{G}_{P_{\beta_0}} \psi_{\beta_0}^\top \dot{P}_{\beta_0} f$ *under* $H_0 : P = P_{\beta_0}$*. In addition, with the same conditions, it holds that* $MKS$ *weakly converges to the supremum of the process under* $H_0 : P_0 = P_{\beta_0}$*.*

The asymptotic linearity in (S1) can be satisfied in several settings. For example, in the above example, the proof of Theorem 3 shows that

$$\sqrt{N}(\hat{\beta}_{NT}^{(1)} - \beta_0^{(1)}) = \frac{1}{\sqrt{N}} \sum_{i=1}^{N} (\mu_i - \beta_0^{(1)}) + o_{P_{\beta_0}}(1),$$
$$\sqrt{N}(\hat{\beta}_{NT}^{(2)} - \beta_0^{(2)}) = \frac{1}{\sqrt{N}} \sum_{i=1}^{N} (\mu_i^2 - \beta_0^{(2)}) + o_{P_{\beta_0}}(1),$$

when $N, T \to \infty$ with $N/T^2 \to 0$ which is weaker than $N^{3+\epsilon}/T^4 \to 0$ for some $\epsilon \in (0, 1/3)$.

The asymptotic law of $MKS$ is not known in a closed form and it should be approximated by simulations in practice.

# D Appendix: Other extensions

This appendix contains several extensions omitted from the main text.

## D.1 Time effects

We can extend our procedures with only a minor modification to cases that have time-specific effects. Let $y_{it} = \mu_i + \eta_t + w_{it}$, where $\mu_i$ is a unit-specific mean, $\eta_t$ is a time-specific effect, and $w_{it}$ is an idiosyncratic error.[S1] Here, $\eta_t$ may be nonstationary, such that it is a unit root process or a time trend. We can estimate $\mu_i$ with $\hat{\mu}_i = T^{-1} \sum_{t=1}^{T} (y_{it} - \bar{y}_t)$ where $\bar{y}_t := N^{-1} \sum_{i=1}^{N} y_{it}$. We

[S1] How to handle non-additive time effects would be non-trivial. We leave such extension for a future research topic.

estimate the distribution of $\mu_i$ using the empirical distribution of $\hat{\mu}_i$. Note that estimated mean of $\mu_i$ is always zero, and the mean of $\mu_i$ is in fact unidentified because it cannot be distinguished from that of $\eta_t$. When we are also interested in the distribution of $\gamma_{k,i}$ or $\rho_{k,i}$, we transform the variable as follows: $\tilde{y}_{it} \coloneqq y_{it} - \bar{y}_i - \bar{y}_t + \bar{y}$ where $\bar{y} \coloneqq (NT)^{-1} \sum_{i=1}^{N} \sum_{t=1}^{T} y_{it}$. We modify the estimators for $\gamma_{k,i} = E(w_{it} w_{i,t-k}|i)$ and $\rho_{k,i} = \gamma_{k,i}/\gamma_{0,i}$ as $\hat{\gamma}_{k,i} = (T-k)^{-1} \sum_{t=k+1}^{T} \tilde{y}_{it} \tilde{y}_{i,t-k}$ and $\hat{\rho}_{k,i} = \hat{\gamma}_{k,i}/\hat{\gamma}_{0,i}$. We construct the estimators for the distributional properties of $\gamma_{k,i}$ and $\rho_{k,i}$ based on the empirical distributions of $\hat{\gamma}_{k,i}$ and $\hat{\rho}_{k,i}$.

The formal investigation of the asymptotic properties in the presence of time effects is an interesting yet non-trivial task. Here, we conjecture that the asymptotic normality of $\hat{S}$ under $N, T \to \infty$ with $N/T^2 \to 0$ in the main body still holds even in the presence of time effects. Okui (2014) shows that the bias caused by eliminating time effects would be of order $O(1/N)$ in his study on the influence of time-specific effects in a homogeneous dynamic structure. We expect that a similar result would be obtained in heterogeneous dynamics cases. Since the convergence rates of our estimators are of order $O_p(1/\sqrt{N})$, the bias caused by time effects would be asymptotically negligible, regardless of the relative magnitudes of $N$ and $T$. Consequently, the HPJ bias correction and cross-sectional bootstrap inference would remain valid with the presence of time effects. We are currently developing the formal investigation on such extensions as another research project.

### D.2 Covariates

Our procedures could allow for the presence of covariates. We can use covariates in at least two ways: to control for effects of covariates; and to examine the relationships between the heterogeneous quantities and covariates.

The presence of covariates enables controlling for their effects before investigating the distributional properties of the heterogeneous quantities. If there are discrete covariates with small support, we split the data $\{\{y_{it}\}_{t=1}^{T}\}_{i=1}^{N}$ into "cells" according to the discrete covariates. We can then estimate the distributional properties of $\mu_i$, $\gamma_{k,i}$, and $\rho_{k,i}$ in each cell, which controls covariates in a model-free manner. If there are discrete covariates with large support or continuous covariates, there are several approaches to control covariates. For example, we first estimate $\mu_i$, $\gamma_{k,i}$, and $\rho_{k,i}$ for each cross-sectional unit while controlling covariates using some nonparametric technique (e.g., kernel regression), and then estimate the distributional properties of these estimated $\mu_i$, $\gamma_{k,i}$, and

$\rho_{k,i}$ as in the main text. This approach is fully nonparametric, although one should be careful of potential threats of nonparametric estimation problems (e.g., the curse of dimensionality and the difficulty of optimal bandwidth selection). As another example, we obtain the residuals from the linear regression of $y_{it}$ on covariates, and then compute the distributional properties of the heterogeneous quantities of the residuals.

We may also consider investigating the relationships between the heterogeneous quantities and covariates. In this case, we first estimate the sample mean, autocovariances, and autocorrelations for each unit as in the main body. We can then compute quantities that characterize the relationships between these estimated quantities and covariates, such as their correlations, regression functions, and their joint or conditional distributions, based on model-free or model-based approaches. For example, Crucini, Shintani, and Tsuruga (2015) consider such model-based approach to see whether heterogeneity in the LOP deviation dynamics relates to distance measure between cities.

### D.3 Asymptotics under homogeneity

If, in fact, the dynamics of $y_{it}$ are homogeneous across units, the convergence rate of $\hat{S}$ is not on the order of $O_p(1/\sqrt{N})$, but on the order of $O_p(1/\sqrt{NT})$ and the asymptotic variance is different. To see this, consider the following simple example. Let the $k$-th autocovariance be such that $\gamma_{k,i} = \gamma_k$ for any $i$ and constant $\gamma_k$. Suppose that our parameter of interest is $S = E(\gamma_{k,i}) = \gamma_k$. In this case, the estimator is $\hat{S} = N^{-1}\sum_{i=1}^N \hat{\gamma}_{k,i} = (N(T-k))^{-1}\sum_{i=1}^N \sum_{t=k+1}^T (y_{it} - \bar{y}_i)(y_{i,t-k} - \bar{y}_i)$. This estimator is identical to that for the homogeneous autocovariance $\gamma_k$ considered in Okui (2010). Hence, in this case, when $N, T \to \infty$ with $N/T^3 \to 0$, we have $\sqrt{NT}(\hat{S} - S + B/T) \rightsquigarrow \mathcal{N}(0, \Sigma)$ where $B$ is the bias term and $\Sigma$ is the asymptotic variance and their precise expressions are given in Okui (2010). The same argument holds for more general $\hat{S}$. The HPJ bias correction and the bootstrap inference proposed in the main body remain valid in this case.

### D.4 Asymptotics with different parameters of interest

The asymptotic results also change if the parameter of interest is not, for example, $E(g(\mu_i))$, but $N^{-1}\sum_{i=1}^N g(\mu_i)$. In this case, the estimator $N^{-1}\sum_{i=1}^N g(\hat{\mu}_i)$ is still consistent for $N^{-1}\sum_{i=1}^N g(\mu_i)$,

but the convergence rate changes from $O_p(1/\sqrt{N})$ to $O_p(1/\sqrt{NT})$. Specifically, we can show that

$$\begin{aligned}\sqrt{NT}\left(\frac{1}{N}\sum_{i=1}^{N} g(\hat{\mu}_i) - \frac{1}{N}\sum_{i=1}^{N} g(\mu_i)\right) &= \frac{1}{\sqrt{NT}}\sum_{i=1}^{N}\sum_{t=1}^{T} g'(\mu_i) w_{it} + \frac{\sqrt{T}}{2\sqrt{N}}\sum_{i=1}^{N} g''(\tilde{\mu}_i)(\hat{\mu}_i - \mu_i)^2 \\ &\rightsquigarrow \mathcal{N}\Big(0, E\big((g'(\mu_i))^2 V_i\big)\Big) + O_p\left(\frac{\sqrt{N}}{\sqrt{T}}\right),\end{aligned}$$

by Taylor's theorem and the CLT, where $V_i \coloneqq \sum_{j=-\infty}^{\infty} \gamma_{j,i}$. In this case, the convergence rate is of order $O_p(1/\sqrt{NT})$ and asymptotic normality holds as $N, T \to \infty$ with $N/T \to 0$.

### D.5 Half-series jackknife

One may consider applying the half-series jackknife (HSJ) in Quenouille (1949, 1956) to each $\hat{\gamma}_{k,i}$, but we argue that the HSJ is not suitable in the current context. In the HSJ method, we bias-correct each $\hat{\gamma}_{k,i}$ using the jackknife. Suppose $T$ is even. Let $\hat{\gamma}_{k,i}^{(1)}$ be the estimator of $\gamma_{k,i}$ using $\{y_{it}\}_{t=1}^{T/2}$, and $\hat{\gamma}_{k,i}^{(2)}$ be that based on $\{y_{it}\}_{t=T/2+1}^{T}$. Let $\bar{\gamma}_{k,i} \coloneqq (\hat{\gamma}_{k,i}^{(1)} + \hat{\gamma}_{k,i}^{(2)})/2$. The HSJ bias-corrected estimator of $\gamma_{k,i}$ is $\hat{\gamma}_{k,i}^{H} \coloneqq \hat{\gamma}_{k,i} - (\bar{\gamma}_{k,i} - \hat{\gamma}_{k,i}) = 2\hat{\gamma}_{k,i} - \bar{\gamma}_{k,i}$. We then estimate $S$ using $\{\hat{\gamma}_{k,i}^{H}\}_{i=1}^{N}$. The HSJ can reduce the bias of order $O(1/T)$ in $\hat{\gamma}_{k,i}$, and therefore the incidental parameter bias in $\hat{S}$. However, it does not reduce the bias caused by the non-linearity of $g$, nor that of $h$. Thus, we do not pursue a theoretical investigation of the HSJ in this study. We note that when both $h$ and $g$ are linear, the HPJ and HSJ are numerically equivalent.

## E Appendix: Proofs omitted from the main text

This appendix collects the proofs of the theorems and lemmas omitted from the main text. For ease of reference, we restate the assumptions and the theorems and lemmas to be proved here.

### E.1 Assumptions

**Assumption 1.** *The sample space of $\alpha_i$ is some Polish space and $y_{it} \in \mathbb{R}$ is a scalar real random variable. $\{(\{y_{it}\}_{t=1}^{T}, \alpha_i)\}_{i=1}^{N}$ is i.i.d. across $i$.*

**Assumption 2.** *For each $i$, $\{y_{it}\}_{t=1}^{\infty}$ is strictly stationary and $\alpha$-mixing given $\alpha_i$, with mixing coefficients $\{\alpha(m|i)\}_{m=0}^{\infty}$. There exists a natural number $r_m$ and a sequence $\{\alpha(m)\}_{m=0}^{\infty}$ such that*

*for any $i$ and $m$, $\alpha(m|i) \leq \alpha(m)$ and $\sum_{m=0}^{\infty}(m+1)^{r_m/2-1}\alpha(m)^{\delta/(r_m+\delta)} < \infty$ for some $\delta > 0$.*

**Assumption 3.** *There exists a natural number $r_d$ such that $E|w_{it}|^{r_d+\delta} < \infty$ for some $\delta > 0$.*

**Assumption 4.** *a) The random variable $\mu_i$ is continuously distributed. b) The CDF of $\mu_i$ is thrice boundedly differentiable. c) The CDF of $\hat{\mu}_i$ is thrice boundedly differentiable uniformly over $T$. d) There exists some fixed $M < \infty$ such that $E[(\bar{w}_i)^2|\mu_i = \cdot] \leq M/T$.*

**Assumption 5.** *a) The random variable $\gamma_{k,i}$ is continuously distributed. b) The CDF of $\gamma_{k,i}$ is thrice boundedly differentiable. c) The CDF of $\hat{\gamma}_{k,i}$ is thrice boundedly differentiable uniformly over $T$. d) There exists some fixed $M < \infty$ such that $E[(\bar{w}_i)^2|\gamma_{k,i} = \cdot] \leq M/T$ and $E[(\hat{\gamma}_{k,i} - \gamma_{k,i})^2|\gamma_{k,i} = \cdot] \leq M/T$.*

**Assumption 6.** *a) The random variable $\rho_{k,i}$ is continuously distributed. b) The CDF of $\rho_{k,i}$ is thrice boundedly differentiable. c) The CDF of $\hat{\rho}_{k,i}$ is thrice boundedly differentiable uniformly over $T$. d) There exists some fixed $M < \infty$ such that $E[(\bar{w}_i)^2|\rho_{k,i} = \cdot] \leq M/T$, $E[(\hat{\gamma}_{k,i} - \gamma_{k,i})^2|\rho_{k,i} = \cdot] \leq M/T$, and $E[(\hat{\gamma}_{0,i} - \gamma_{0,i})^2|\rho_{k,i} = \cdot] \leq M/T$. e) There exist some fixed $\varepsilon > 0$ and $M < \infty$ such that $\hat{\gamma}_{0,i} > \varepsilon$, $\gamma_{0,i} > \varepsilon$, $|\hat{\gamma}_{k,i}| < M$, and $|\gamma_{k,i}| < M$ almost surely.*

**Assumption 7.** *The function $h : \mathbb{R}^m \to \mathbb{R}^n$ is continuous in a neighborhood of $G$.*

**Assumption 8.** *The function $h : \mathbb{R}^m \to \mathbb{R}^n$ is continuously differentiable in a neighborhood of $G$. The matrix of the first derivatives $\nabla h(G) \coloneqq (\nabla h_1(G)^\top, \nabla h_2(G)^\top, \ldots, \nabla h_n(G)^\top)^\top$ is of full row rank.*

**Assumption 9.** *The function $g = (g_1, g_2, \ldots, g_m) : \mathcal{O} \to \mathbb{R}^m$ is twice-continuously differentiable where $\mathcal{O} \subset \mathbb{R}^l$ is a convex open subset. The covariance matrix $\Gamma \coloneqq E[(g(\theta_i) - E(g(\theta_i)))(g(\theta_i) - E(g(\theta_i)))^\top]$ exists and is non-singular. For any $p = 1, 2, \ldots, m$, the elements of the Hessian matrix of $g_p$ are bounded functions. For any $p = 1, 2, \ldots, m$, the function $g_p$ satisfies $E[((\partial/\partial z_j)g_p(z)|_{z=\theta_i})^4] < \infty$ for any $j = 1, 2, \ldots, m$.*

**Assumption 10.** *The function $g = (g_1, g_2, \ldots, g_m) : \mathcal{O} \to \mathbb{R}^m$ is thrice differentiable. The covariance matrix $\Gamma = E[(g(\theta_i) - E(g(\theta_i)))(g(\theta_i) - E(g(\theta_i)))^\top]$ exists and is nonsingular. For any $p = 1, 2, \ldots, m$, the function $g_p$ satisfies $E[((\partial/\partial z_j)g_p(z)|_{z=\theta_i})^4] < \infty$ for any $j = 1, 2, \ldots, m$, and $E[((\partial^2/\partial z_{j_1}\partial z_{j_2})g_p(z)|_{z=\theta_i})^4] < \infty$ for any $j_1, j_2 = 1, 2, \ldots, m$. All third-order derivatives of $g$ are bounded.*

**Assumption 11.** *The function $g = (g_1, g_2, \dots, g_m) : \mathcal{O} \to \mathbb{R}^m$ is twice-continuously differentiable. The covariance matrix of $g(\theta_i)$, $\Gamma$, exists and is non-singular. The elements of the Hessian matrices of $g_p$ for $p = 1, 2, \dots, m$, $g_{p_1}(\cdot)g_{p_2}(\cdot)$ for $p_1, p_2 = 1, 2, \dots, m$, and $(g(\cdot)^\top g(\cdot))$ are bounded. For any $p = 1, 2, \dots, m$, the function $g_p$ satisfies $E[((\partial/\partial z_j)g_p(z)|_{z=\theta_i})^4] < \infty$ for any $j = 1, 2, \dots, l$. For any $p_1, p_2 = 1, 2, \dots, m$, $E[((\partial/\partial z_j)g_{p_1}(z)|_{z=\theta_i} g_{p_2}(\theta_i))^2] < \infty$. For any $j = 1, 2, \dots, l$, $E[(g(\theta_i)^\top g(\theta_i)(\partial/\partial z_j)g_{p_1}(z)|_{z=\theta_i} g_{p_2}(\theta_i))^2] < \infty$ is satisfied.*

## E.2 Proofs of theorems omitted from the main text

**Theorem 3.** *Let $r^* = 4$ if $\theta_i = \mu_i$ such that $S = h(E(g(\mu_i)))$ for some $h$ and $g$, and $r^* = 8$ if $\theta_i$ contains $\gamma_{k,i}$ for some $k$. Suppose also that Assumptions 1, 2, 3, 7, and 9 hold for $r_m = 4$ and $r_d = r^*$. When $N, T \to \infty$, it holds that $\hat{S} \xrightarrow{p} S$. Moreover, suppose that Assumption 8 also holds. When $N, T \to \infty$ with $N/T^2 \to 0$, it holds that*

$$\sqrt{N}(\hat{S} - S) \rightsquigarrow \mathcal{N}\left(0, \nabla h(G)\Gamma(\nabla h(G))^\top\right).$$

*Proof.* We show only the asymptotic normality of $\sqrt{N}(\hat{S} - S)$, because the consistency of $\hat{S}$ is clear by the following proof and the continuous mapping theorem. Let $\hat{G} = N^{-1}\sum_{i=1}^N g(\hat{\theta}_i)$, $G = E(g(\theta_i))$, $\hat{\theta}_i = (\hat{\theta}_{1,i}, \hat{\theta}_{2,i}, \dots, \hat{\theta}_{l,i})^\top$, and $\theta_i = (\theta_{1,i}, \theta_{2,i}, \dots, \theta_{l,i})^\top$. If we show $\sqrt{N}(\hat{G} - G) \rightsquigarrow \mathcal{N}(0, \Gamma)$, the asymptotic normality of $\sqrt{N}(\hat{S} - S)$ follows by the delta method. We thus focus on the proof for $\sqrt{N}(\hat{G} - G) \rightsquigarrow \mathcal{N}(0, \Gamma)$.

By Taylor's theorem, we have

$$\begin{aligned} \sqrt{N}(\hat{G} - G) = \frac{1}{\sqrt{N}}\sum_{i=1}^N \left(g(\hat{\theta}_i) - G\right) = & \frac{1}{\sqrt{N}}\sum_{i=1}^N (g(\theta_i) - G) && \text{(S2)} \\ & + \frac{1}{\sqrt{N}}\sum_{i=1}^N \nabla g(\theta_i)(\hat{\theta}_i - \theta_i) && \text{(S3)} \\ & + \frac{1}{2\sqrt{N}}\sum_{i=1}^N Q_i, && \text{(S4)} \end{aligned}$$

where $\nabla g(\theta_i) := (\nabla g_1(\theta_i)^\top, \dots, \nabla g_m(\theta_i)^\top)^\top$ is the first derivative (a $m \times l$ matrix) of $g$ evaluated at $\theta_i$, $Q_i$ is the $m \times 1$ matrix whose $p$th element is $(\hat{\theta}_i - \theta_i)^\top \mathcal{H}(g_p)(\tilde{\theta}_i^{(p)})(\hat{\theta}_i - \theta_i)$ for $p = 1, 2, \dots, m$ where $\mathcal{H}(g_p)$ is the Hessian matrix of $g_p$, and $\tilde{\theta}_i^{(p)}$ is between $\theta_i$ and $\hat{\theta}_i$ (see Feng, Wang, Chen, and

Tu, 2014). We examine each term below.

For (S2), under Assumptions 1 and 9, $N^{-1/2}\sum_{i=1}^{N}(g(\theta_i)-G) \rightsquigarrow \mathcal{N}(0,\Gamma)$ by the CLT for i.i.d. random vectors.

For (S3), we show that it is of order $O_p(\sqrt{N}/T)$. By simple algebra, we have

$$\frac{1}{\sqrt{N}}\sum_{i=1}^{N}\nabla g(\theta_i)(\hat{\theta}_i-\theta_i)=\sum_{j=1}^{l}\begin{pmatrix} N^{-1/2}\sum_{i=1}^{N}a_{1,j,i}(\hat{\theta}_{j,i}-\theta_{j,i}) \\ N^{-1/2}\sum_{i=1}^{N}a_{2,j,i}(\hat{\theta}_{j,i}-\theta_{j,i}) \\ \vdots \\ N^{-1/2}\sum_{i=1}^{N}a_{m,j,i}(\hat{\theta}_{j,i}-\theta_{j,i}) \end{pmatrix},$$

where $a_{p,j,i} \coloneqq (\partial/\partial z_j)g_p(z)|_{z=\theta_i}$ for $p=1,2,\ldots,m$. Since $l$ and $m$ are fixed, it is sufficient to show that for $p=1,2,\ldots,m$

$$\frac{1}{\sqrt{N}}\sum_{i=1}^{N}a_{p,j,i}(\hat{\theta}_{j,i}-\theta_{j,i})=O_p\left(\frac{\sqrt{N}}{T}\right), \tag{S5}$$

thanks to Chebyshev's inequality for random vectors and Slutsky's theorem. To this end, we consider the following two cases: (i) $\theta_{j,i}=\mu_i$ and (ii) $\theta_{j,i}=\gamma_{k,i}$ for some $k$.

If $\theta_{j,i}=\mu_i$ in the left-hand side of (S5), we have $N^{-1/2}\sum_{i=1}^{N}a_{p,j,i}(\hat{\mu}_i-\mu_i)=N^{-1/2}\sum_{i=1}^{N}a_{p,j,i}\bar{w}_i$. This term has zero mean and the variance is

$$var\left(\frac{1}{\sqrt{N}}\sum_{i=1}^{N}a_{p,j,i}\bar{w}_i\right)=E\left(a_{p,j,i}^2\,(\bar{w}_i)^2\right)\leq\sqrt{E(a_{p,j,i}^4)}\sqrt{E\left((\bar{w}_i)^4\right)}=O(T^{-1}),$$

where the first equality follows from Assumption 1, the inequality is the Cauchy–Schwarz inequality, and the last equality follows from Assumption 9 and Lemma 3 for $r_m=4$ and $r_d=4$. Thus, we have (S5) in this case.

If $\theta_{j,i}=\gamma_{k,i}$ for some $k$ in the left-hand side of (S5), we have the following expansion:

$$\begin{aligned}&\frac{1}{\sqrt{N}}\sum_{i=1}^{N}a_{p,j,i}(\hat{\gamma}_{k,i}-\gamma_{k,i})\\ =&\frac{1}{\sqrt{N}}\sum_{i=1}^{N}a_{p,j,i}\left(\frac{1}{T-k}\sum_{t=k+1}^{T}w_{it}w_{i,t-k}-\gamma_{k,i}\right)\end{aligned} \tag{S6}$$

$$-\frac{1}{\sqrt{N}}\frac{T+k}{T-k}\sum_{i=1}^{N}a_{p,j,i}(\bar{w}_i)^2 \tag{S7}$$

$$+\frac{1}{\sqrt{N}}\sum_{i=1}^{N}\frac{1}{T-k}a_{p,j,i}\sum_{t=1}^{k}w_{it}\bar{w}_i+\frac{1}{\sqrt{N}}\sum_{i=1}^{N}\frac{1}{T-k}a_{p,j,i}\sum_{t=T-k+1}^{T}w_{it}\bar{w}_i. \tag{S8}$$

The term in (S6) has zero mean and the variance is

$$\begin{aligned}
&var\left(\frac{1}{\sqrt{N}}\sum_{i=1}^{N}a_{p,j,i}\left(\frac{1}{T-k}\sum_{t=k+1}^{T}w_{it}w_{i,t-k}-\gamma_{k,i}\right)\right)\\
=&E\left(a_{p,j,i}^2\left(\frac{1}{T-k}\sum_{t=k+1}^{T}w_{it}w_{i,t-k}-\gamma_{k,i}\right)^2\right)\\
\leq&\sqrt{E(a_{p,j,i}^4)}\sqrt{E\left(\left(\frac{1}{T-k}\sum_{t=k+1}^{T}w_{it}w_{i,t-k}-\gamma_{k,i}\right)^4\right)}=O\left(\frac{1}{T}\right),
\end{aligned}$$

where the first equality follows from Assumption 1, the inequality is the Cauchy–Schwartz inequality, and the last equality follows from Assumption 9 and Lemma 5 for $r_m = 4$ and $r_d = 8$. Thus, the term in (S6) is of order $O_p(1/\sqrt{T})$ by Markov's inequality. For the term in (S7), the absolute mean is

$$\begin{aligned}
E\left|\frac{1}{\sqrt{N}}\frac{T+k}{T-k}\sum_{i=1}^{N}a_{p,j,i}(\bar{w}_i)^2\right| &\leq \frac{T+k}{T-k}\sqrt{N}E|a_{p,j,i}(\bar{w}_i)^2|\\
&\leq \frac{T+k}{T-k}\sqrt{N}\sqrt{E(a_{p,j,i}^2)}\sqrt{E((\bar{w}_i)^4)}=O\left(\frac{\sqrt{N}}{T}\right),
\end{aligned}$$

where the first and second inequalities are the triangle inequality and the Cauchy–Schwarz inequality, respectively. The last result follows from Assumption 9 and Lemma 3 for $r_m = 4$ and $r_d = 4$. Thus, the term in (S7) is of order $O_p(\sqrt{N}/T)$ by Markov's inequality. We can similarly show that the terms in (S8) are of order $o_p(\sqrt{N}/T)$. Therefore, in this case, we have (S5) by Slutsky's theorem.

Accordingly, we have shown (S5) for any $\theta_{j,i}$, which means that the term in (S3) is of order $O_p(\sqrt{N}/T)$.

We show that (S4) is of order $O_p(\sqrt{N}/T)$. We observe that the mean of the Euclidean norm is

$$
\begin{aligned}
E\left\|\frac{1}{2\sqrt{N}}\sum_{i=1}^{N}Q_i\right\| &\leq \frac{\sqrt{N}}{2}E\|Q_i\| \\
&\leq \frac{\sqrt{N}}{2}\sum_{p=1}^{m}E|(\hat{\theta}_i-\theta_i)^\top\mathcal{H}(g_p)(\tilde{\theta}_i^{(p)})(\hat{\theta}_i-\theta_i)| \\
&\leq \sqrt{N}M\sum_{p=1}^{m}\sum_{j_1=1}^{l}\sum_{j_2=1}^{l}E|(\hat{\theta}_{j_1,i}-\theta_{j_1,i})(\hat{\theta}_{j_2,i}-\theta_{j_2,i})| \\
&= O(\sqrt{N}/T),
\end{aligned}
$$

where the first inequality follows from the triangle inequality, the second follows from the triangle inequality, the third follows from the triangle inequality and Assumption 9, and the last follows from the Cauchy–Schwarz inequality, Corollary 3, Lemma 6, and fixed $m$ and $l$. Therefore, (S4) is $O_p(\sqrt{N}/T)$ by Markov's inequality.

Consequently, we obtain the desired result by Slutsky's theorem. □

**Theorem 4.** *Let $r^* = 8$ if $\theta_i = \mu_i$ such that $S = h(E(g(\mu_i)))$ for some $h$ and $g$, and $r^* = 16$ if $\theta_i$ contains $\gamma_{k,i}$ for some $k$. Suppose that Assumptions 1, 2, 3, 8, and 10 are satisfied for $r_m = 8$ and $r_d = r^*$. When $N, T \to \infty$ with $N/T^2 \to \nu$ for some $\nu \in [0,\infty)$, it holds that*

$$
\sqrt{N}(\hat{S}^H - S) \rightsquigarrow \mathcal{N}\left(0, \nabla h(G)\Gamma(\nabla h(G))^\top\right).
$$

*Proof.* We first examine the estimation of $G = E(g(\theta_i))$. We focus on cases in which $m = 1$ such that $g$ is a univariate function. Note that it is easy to extend our result to cases with $m > 1$.

The Taylor expansion gives

$$
\begin{aligned}
&\sqrt{N}(\hat{G}-G) \\
=&\frac{1}{\sqrt{N}}\sum_{i=1}^{N}(g(\theta_i)-G) \\
&+\frac{1}{\sqrt{N}}\sum_{i=1}^{N}\sum_{j=1}^{l}\frac{\partial}{\partial z_j}g(z)\big|_{z=\theta_i}(\hat{\theta}_{j,i}-\theta_{j,i}) \qquad \text{(S9)} \\
&+\frac{1}{2\sqrt{N}}\sum_{i=1}^{N}\sum_{j_1=1}^{l}\sum_{j_2=1}^{l}\frac{\partial^2}{\partial z_{j_1}\partial z_{j_2}}g(z)\big|_{z=\theta_i}(\hat{\theta}_{j_1,i}-\theta_{j_1,i})(\hat{\theta}_{j_2,i}-\theta_{j_2,i}) \qquad \text{(S10)}
\end{aligned}
$$

$$+\frac{1}{6\sqrt{N}}\sum_{i=1}^{N}\sum_{j_1=1}^{l}\sum_{j_2=1}^{l}\sum_{j_3=1}^{l}\frac{\partial^3}{\partial z_{j_1}\partial z_{j_2}\partial z_{j_3}}g(z)\big|_{z=\tilde{\theta}_i}(\hat{\theta}_{j_1,i}-\theta_{j_1,i})(\hat{\theta}_{j_2,i}-\theta_{j_2,i})(\hat{\theta}_{j_3,i}-\theta_{j_3,i}), \tag{S11}$$

where $\tilde{\theta}_i$ is between $\theta_i$ and $\hat{\theta}_i$ (see Feng et al., 2014).

The proof follows Dhaene and Jochmans's (2015) arguments. We shall show that

$$\sqrt{N}(\hat{G}-G)=\frac{1}{\sqrt{N}}\sum_{i=1}^{N}(g(\theta_i)-G)+\frac{\sqrt{N}}{T}B+o_p\left(\frac{\sqrt{N}}{T}\right),$$

for some $B$. This result also implies that

$$\sqrt{N}(\bar{G}-G)=\frac{1}{\sqrt{N}}\sum_{i=1}^{N}(g(\theta_i)-G)+2\frac{\sqrt{N}}{T}B+o_p\left(\frac{\sqrt{N}}{T}\right),$$

where $\bar{G}\coloneqq(\hat{G}^{(1)}+\hat{G}^{(2)})/2$. Consequently, when $N,T\to\infty$ and $N/T^2\to\nu$, we have

$$\sqrt{N}(\hat{G}^H-G)=\frac{1}{\sqrt{N}}\sum_{i=1}^{N}(g(\theta_i)-E(g(\theta_i)))+o_p\left(\frac{\sqrt{N}}{T}\right)\rightsquigarrow\mathcal{N}(0,\Gamma),$$

where $\hat{G}^H\coloneqq 2\hat{G}-\bar{G}$.

We first consider the term in (S9). Let $a_{j,i}\coloneqq\frac{\partial}{\partial z_j}g(z)\big|_{z=\theta_i}$. Suppose that $\theta_{j,i}=\mu_i$. In this case, we have $N^{-1/2}\sum_{i=1}^{N}a_{j,i}(\hat{\mu}_i-\mu_i)=N^{-1/2}\sum_{i=1}^{N}a_{j,i}\bar{w}_i=O_p(T^{-1/2})$ by the same argument in the proof of Theorem 3.

Suppose next that $\theta_{j,i}=\gamma_{k,i}$ for some $k$. In this case, we have

$$\begin{aligned}
&\frac{1}{\sqrt{N}}\sum_{i=1}^{N}a_{j,i}(\hat{\gamma}_{k,i}-\gamma_{k,i})\\
=&\frac{1}{\sqrt{N}}\sum_{i=1}^{N}a_{j,i}\left(\frac{1}{T-k}\sum_{t=k+1}^{T}w_{it}w_{i,t-k}-\gamma_{k,i}\right) && \text{(S12)}\\
&-\frac{1}{\sqrt{N}}\frac{T+k}{T-k}\sum_{i=1}^{N}a_{j,i}(\bar{w}_i)^2 && \text{(S13)}\\
&+\frac{1}{\sqrt{N}}\sum_{i=1}^{N}\frac{1}{T-k}a_{j,i}\sum_{t=1}^{k}w_{it}\bar{w}_i+\frac{1}{\sqrt{N}}\sum_{i=1}^{N}\frac{1}{T-k}a_{j,i}\sum_{t=T-k+1}^{T}w_{it}\bar{w}_i. && \text{(S14)}
\end{aligned}$$

The term (S12) is of order $O_p(T^{-1/2})$ by the same argument in the proof of Theorem 3. For the

term in (S13), we observe that

$$E\left(\frac{1}{\sqrt{N}}\frac{T+k}{T-k}\sum_{i=1}^{N}a_{j,i}(\bar{w}_i)^2\right)=\frac{T+k}{T-k}\frac{\sqrt{N}}{T}E(a_{j,i}V_{T,i})=\frac{\sqrt{N}}{T}E(a_{j,i}V_i)+o\left(\frac{\sqrt{N}}{T}\right),$$

where $V_{T,i}\coloneqq TE((\bar{w}_i)^2|i)=\sum_{j=-T}^{T}\gamma_{j,i}(T-|j|)/T$ and $V_i\coloneqq\sum_{j=-\infty}^{\infty}\gamma_{j,i}$. The variance is

$$\begin{aligned} var\left(\frac{1}{\sqrt{N}}\sum_{i=1}^{N}a_{j,i}(\bar{w}_i)^2\right)&=var(a_{j,i}(\bar{w}_i)^2)\leq E(a_{j,i}^2(\bar{w}_i)^4)\\ &\leq\sqrt{E(a_{j,i}^4)}\sqrt{E((\bar{w}_i)^8)}=O\left(\frac{1}{T^2}\right), \end{aligned}$$

where the second inequality is the Cauchy–Schwarz inequality and the third inequality follows from Assumptions 2, 3, and 10 and Lemma 3. Therefore,

$$\frac{1}{\sqrt{N}}\sum_{i=1}^{N}a_{j,i}\frac{T+k}{T-k}(\bar{w}_i)^2=\frac{\sqrt{N}}{T}E(a_{j,i}V_i)+o_p\left(\frac{\sqrt{N}}{T}\right).$$

Given this result, it is easy to see that the terms in (S14) are of order $o_p(\sqrt{N}/T)$.

Thus, the term in (S9) can be written as

$$\frac{1}{\sqrt{N}}\sum_{i=1}^{N}\sum_{j=1}^{l}\frac{\partial}{\partial z_j}g(z)\big|_{z=\theta_i}(\hat{\theta}_{j,i}-\theta_{j,i})=\frac{\sqrt{N}}{T}\sum_{j=1}^{l}\mathbf{1}_{\{\theta_{j,i}\neq\mu_i\}}E(a_{j,i}V_i)+o_p\left(\frac{\sqrt{N}}{T}\right).$$

Next, we consider the term in (S10). Let $b_{j_1,j_2,i}\coloneqq\frac{\partial^2}{\partial z_{j_1}\partial z_{j_2}}g(z)\big|_{z=\theta_i}$. We consider four patterns for $\theta_{j_1,i}$ and $\theta_{j_2,i}$: $\theta_{j_1,i}=\theta_{j_2,i}=\mu_i$, $\theta_{j_1,i}=\theta_{j_2,i}=\gamma_{k,i}$ for some $k$, $\theta_{j_1,i}=\mu_i$ and $\theta_{j_2,i}=\gamma_{k,i}$ for some $k$, and $\theta_{j_1,i}=\gamma_{k_1,i}$ and $\theta_{j_2,i}=\gamma_{k_2,i}$ for some $k_1,k_2$. We first consider the case in which $j_1=j_2=j$ and $\theta_{j,i}=\mu_i$. In this case, we have

$$\frac{1}{2\sqrt{N}}\sum_{i=1}^{N}b_{j,j,i}(\hat{\mu}_i-\mu_i)^2=\frac{1}{2\sqrt{N}}\sum_{i=1}^{N}b_{j,j,i}(\bar{w}_i)^2.$$

The argument to analyze the term in (S13) gives

$$\frac{1}{2\sqrt{N}}\sum_{i=1}^{N}b_{j,j,i}(\hat{\mu}_i-\mu_i)^2=\frac{\sqrt{N}}{2T}E(b_{j,j,i}V_i)+o_p\left(\frac{\sqrt{N}}{T}\right).$$

Second, we consider the case where $j_1 = j_2 = j$ and $\theta_{j,i} = \gamma_{k,i}$ for some $k$. It is easy to see that the mean is

$$E\left(\frac{1}{2\sqrt{N}}\sum_{i=1}^{N} b_{j,j,i}(\hat{\gamma}_{k,i}-\gamma_{k,i})^2\right) = \frac{\sqrt{N}}{2}E\left(b_{j,j,i}\left(\frac{1}{T-k}\sum_{t=k+1}^{T} w_{it}w_{i,t-k}-\gamma_{k,i}\right)^2\right) + o\left(\frac{\sqrt{N}}{T}\right).$$

The i.i.d. assumption and the Cauchy–Schwarz inequality imply that

$$\begin{aligned}
&\frac{\sqrt{N}}{2}E\left(b_{j,j,i}\left(\frac{1}{T-k}\sum_{t=k+1}^{T} w_{it}w_{i,t-k}-\gamma_{k,i}\right)^2\right)\\
\le&\frac{\sqrt{N}}{2(T-k)^2}\sqrt{E\left(\left(\sum_{t=k+1}^{T}(w_{it}w_{i,t-k}-\gamma_{k,i})\right)^4\right)}\sqrt{E(b_{j,j,i}^2)} = O\left(\frac{\sqrt{N}}{T}\right),
\end{aligned}$$

by Lemma 5. Moreover, $TE\left(b_{j,j,i}\left(\sum_{t=k+1}^{T} w_{it}w_{i,t-k}-\gamma_{k,i}\right)^2\right)/2$ converges by the dominated convergence theorem. We denote this limit by $B_k$. Next, we consider the variance term. We observe that

$$\begin{aligned}
var\left(\frac{1}{2\sqrt{N}}\sum_{i=1}^{N} b_{j,j,i}(\hat{\gamma}_{k,i}-\gamma_{k,i})^2\right) =&\frac{1}{4}var\left(b_{j,j,i}(\hat{\gamma}_{k,i}-\gamma_{k,i})^2\right)\\
\le&\frac{1}{4}E\left(b_{j,j,i}^2(\hat{\gamma}_{k,i}-\gamma_{k,i})^4\right)\\
\le&\frac{1}{4}\sqrt{E(b_{j,j,i}^4)}\sqrt{E\left((\hat{\gamma}_{k,i}-\gamma_{k,i})^8\right)} = O\left(\frac{1}{T^2}\right),
\end{aligned}$$

by Lemma 6. Thus, we have

$$\frac{1}{2\sqrt{N}}\sum_{i=1}^{N} b_{j,j,i}(\hat{\gamma}_{k,i}-\gamma_{k,i})^2 = B_k\frac{\sqrt{N}}{T} + o_p\left(\frac{\sqrt{N}}{T}\right).$$

Third, we consider the case when $\theta_{j_1,i} = \mu_i$ and $\theta_{j_2,i} = \gamma_{k,i}$ for some $k$. The mean of this term is

$$\begin{aligned}
&E\left(\frac{1}{2\sqrt{N}}\sum_{i=1}^{N} b_{j_1,j_2,i}(\hat{\mu}_i-\mu_i)(\hat{\gamma}_{k,i}-\gamma_{k,i})\right)\\
=&\frac{\sqrt{N}}{2}E\left(b_{j_1,j_2,i}\bar{w}_i\left(\frac{1}{T-k}\sum_{t=k+1}^{T} w_{it}w_{i,t-k}\right)\right) + o\left(\frac{\sqrt{N}}{T}\right).
\end{aligned}$$

As in the second case, $TE\left(b_{j_1,j_2,i}\bar{w}_i\left(\sum_{t=k+1}^{T} w_{it}w_{i,t-k}\right)\right)$ converges by the dominated convergence theorem and we denote the limit by $B_{\mu,k}$. The variance is

$$\begin{aligned}
&var\left(\frac{1}{2\sqrt{N}}\sum_{i=1}^{N} b_{j_1,j_2,i}(\hat{\mu}_i-\mu_i)(\hat{\gamma}_{k,i}-\gamma_{k,i})\right)\\
=&\frac{1}{4}var\left(b_{j_1,j_2,i}\bar{w}_i(\hat{\gamma}_{k,i}-\gamma_{k,i})\right)\\
\leq&\frac{1}{4}E\left(b_{j_1,j_2,i}^2\bar{w}_i^2(\hat{\gamma}_{k,i}-\gamma_{k,i})^2\right)\\
\leq&\frac{1}{4}\left(E(b_{j_1,j_2,i}^4)\right)^{1/2}\left(E(\bar{w}_i^8)\right)^{1/4}\left(E\left((\hat{\gamma}_{k,i}-\gamma_{k,i})^8\right)\right)^{1/4}=O\left(\frac{1}{T^2}\right),
\end{aligned}$$

by Lemmas 3 and 6 and Assumption 10. Thus, we have

$$\frac{1}{2\sqrt{N}}\sum_{i=1}^{N} b_{j_1,j_2,i}(\hat{\mu}_i-\mu_i)(\hat{\gamma}_{k,i}-\gamma_{k,i})=B_{\mu,k}\frac{\sqrt{N}}{T}+o_p\left(\frac{\sqrt{N}}{T}\right).$$

A similar argument shows that when $\theta_{j_1,i}=\gamma_{k_1,i}$ and $\theta_{j_2,i}=\gamma_{k_2,i}$ for some $k_1$ and $k_2$, we have

$$\frac{1}{2\sqrt{N}}\sum_{i=1}^{N} b_{j_1,j_2,i}(\hat{\gamma}_{k_1,i}-\gamma_{k_1,i})(\hat{\gamma}_{k_2,i}-\gamma_{k_2,i})=B_{k_1,k_2}\frac{\sqrt{N}}{T}+o_p\left(\frac{\sqrt{N}}{T}\right).$$

for some $B_{k_1,k_2}$.

It therefore holds that

$$\frac{1}{2\sqrt{N}}\sum_{i=1}^{N}\sum_{j_1=1}^{l}\sum_{j_2=1}^{l}\frac{\partial^2}{\partial z_{j_1}\partial z_{j_2}}g(z)\big|_{z=\theta_i}(\hat{\theta}_{j_1,i}-\theta_{j_1,i})(\hat{\theta}_{j_2,i}-\theta_{j_2,i})=B\frac{\sqrt{N}}{T}+o_p\left(\frac{\sqrt{N}}{T}\right),$$

for some $B$.

Finally, we consider the term in (S11). Let $c_{j_1,j_2,j_3,i}:=\frac{\partial^3}{\partial z_{j_1}\partial z_{j_2}\partial z_{j_3}}g(z)\big|_{z=\tilde{\theta}_i}$. For any $j_1,j_2,j_3=1,2,\ldots,l$, we have

$$\begin{aligned}
&E\left|\frac{1}{6\sqrt{N}}\sum_{i=1}^{N} c_{j_1,j_2,j_3,i}(\hat{\theta}_{j_1,i}-\theta_{j_1,i})(\hat{\theta}_{j_2,i}-\theta_{j_2,i})(\hat{\theta}_{j_3,i}-\theta_{j_3,i})\right|\\
\leq&\frac{\sqrt{N}}{6}E\left|c_{j_1,j_2,j_3,i}(\hat{\theta}_{j_1,i}-\theta_{j_1,i})(\hat{\theta}_{j_2,i}-\theta_{j_2,i})(\hat{\theta}_{j_3,i}-\theta_{j_3,i})\right|\\
\leq&M\frac{\sqrt{N}}{6}\left(E((\hat{\theta}_{j_1,i}-\theta_{j_1,i})^4)\right)^{1/4}\left(E((\hat{\theta}_{j_2,i}-\theta_{j_2,i})^4)\right)^{1/4}\left(E((\hat{\theta}_{j_3,i}-\theta_{j_3,i})^2)\right)^{1/2}=O\left(\frac{\sqrt{N}}{T^{3/2}}\right),
\end{aligned}$$

where the second inequality follows from Assumption 10 and the repeated application of the Cauchy–Schwarz inequality, and the last equality follows from Assumptions 2 and 3 and Corollary 2 and/or Lemma 6. Thus, the term in (S11) is of order $O_p(\sqrt{N}/T^{3/2})$.

In summary, we showed the asymptotic normality and unbiasedness for the HPJ estimation of $G$. When $m > 1$, we analyze each element of $G$ and obtain the asymptotic normality and unbiasedness.

Next, we consider the estimation of $S = h(G)$. Taylor's theorem gives $\sqrt{N}(\hat{S}-S) = \sqrt{N}\nabla h(G)(\hat{G}-G) + \sqrt{N}(\hat{G}-G)^\top \mathbb{H}(\tilde{G})(\hat{G}-G)$ where $\mathbb{H}$ is the Hessian matrix of $h$ and $\tilde{G}$ is between $\hat{G}$ and $G$. Note that

$$\sqrt{N}\nabla h(G)(\hat{G}-G) = \frac{1}{N}\sum_{i=1}^{N}\nabla h(G)(g(\theta_i)-G) + \frac{\sqrt{N}}{T}\nabla h(G)B + O_p\left(\frac{\sqrt{N}}{T^{3/2}}\right) + o_p\left(\frac{\sqrt{N}}{T}\right).$$

Given $\hat{G}-G = O_p(N^{-1/2}+T^{-1})$, we have

$$\sqrt{N}(\hat{G}-G)^\top \mathbb{H}(\tilde{G})(\hat{G}-G) = O_p\left(\frac{1}{\sqrt{N}} + \frac{1}{T} + \frac{\sqrt{N}}{T^2}\right) = o_p\left(\frac{\sqrt{N}}{T}\right).$$

Thus, the condition for the HPJ estimation of $S$ also holds and the proof is complete. □

**Theorem 5.** *Let $r^* = 4$ if $\theta_i = \mu_i$ such that $S = h(E(g(\mu_i)))$ for some $h$ and $g$, and $r^* = 8$ if $\theta_i$ contains $\gamma_{k,i}$ for some $k$. Suppose that Assumptions 1, 2, 3, 8, and 11 hold for $r_m = 4$ and $r_d = r^*$. When $N, T \to \infty$, we have*

$$\sup_{x\in\mathbb{R}}\left|P^*\left(\sqrt{N}(\hat{S}^*-\hat{S}) \le x\right) - \Pr\left(\mathcal{N}\left(0, \nabla h(G)\Gamma(\nabla h(G))^\top\right) \le x\right)\right| \xrightarrow{p} 0.$$

*Proof.* We first consider $\hat{G}^* = N^{-1}\sum_{i=1}^{N} g(\hat{\theta}_i^*)$. We initially fix a diagonal path $N \to \infty$, $T(N) \to \infty$ and then prove the statement. The statement holds for any diagonal path, which implies that the result holds under double asymptotics. Let $E^*$ and $var^*$ denote the expectation and variance, respectively, operators under the probability measure $P^*$ while keeping $\{\hat{\theta}_j\}_{j=1}^{N}$ fixed.

For each diagonal path, we first show that the moments of $\hat{G}^*$ under the bootstrap distribution satisfy Lyapunov's conditions. We then prove that $\sqrt{N}(\hat{G}^*-\hat{G})$ converges in distribution to $\mathcal{N}(0,\Gamma)$ almost surely under a subsequence of any subsequence of the original sequence. This implies that

the bootstrap distribution of $\sqrt{N}(\hat{G}^* - \hat{G})$ converges almost surely under a subsequence of any sequence, which then implies that it converges in probability in the original sequence.

We first examine the moments of $\hat{G}^*$. It is thus easy to see, depending on the data, that the mean and variance of $g(\hat{\theta}_i^*)$ are $E^*(g(\hat{\theta}_i^*)) = N^{-1}\sum_{i=1}^N g(\hat{\theta}_i) = \hat{G}$ and $var^*(g(\hat{\theta}_i^*)) = N^{-1}\sum_{i=1}^N g(\hat{\theta}_i)g(\hat{\theta}_i)^\top - \hat{G}\hat{G}^\top$. The conditional variance converges to $E(g(\theta_i)g(\theta_i)^\top) - GG^\top = \Gamma$ in probability by Theorem 3 under Assumptions 1, 2, 3, and 11 and the continuous mapping theorem. We then consider the third-order moment. Note that $E^*(N^{-1/2}\|g(\hat{\theta}_i^*) - \hat{G}\|^3) = N^{-3/2}\sum_{i=1}^N \|g(\hat{\theta}_i) - \hat{G}\|^3$. We have $\|g(\hat{\theta}_i) - \hat{G}\|^3 \leq 4\|g(\hat{\theta}_i)\|^3 + 4\|\hat{G}\|^3$. As $\hat{G}$ converges by Theorem 3, the continuous mapping theorem leads to $N^{-1/2}\|\hat{G}\|^3 \xrightarrow{p} 0$. By Hölder's inequality, it follows that

$$\frac{1}{N^{3/2}}\sum_{i=1}^N \|g(\hat{\theta}_i)\|^3 \leq \frac{1}{\sqrt{N}}\left(\frac{1}{N}\sum_{i=1}^N \|g(\hat{\theta}_i)\|^4\right)^{\frac{3}{4}} = \frac{1}{\sqrt{N}}\left(\frac{1}{N}\sum_{i=1}^N (g(\hat{\theta}_i)^\top g(\hat{\theta}_i))^2\right)^{\frac{3}{4}} \xrightarrow{p} 0,$$

as $N^{-1}\sum_{i=1}^N (g(\hat{\theta}_i)^\top g(\hat{\theta}_i))^2 = O_p(1)$ by Theorem 3 under Assumptions 1, 2, 3, and 11. Thus, $N^{-3/2}\sum_{i=1}^N \|g(\hat{\theta}_i) - \hat{G}\|^3 \xrightarrow{p} 0$.

We argue that for any subsequence of the original sequence, there exists a further subsequence under which $\sqrt{N}(\hat{G}^* - \hat{G})$ converges in distribution conditionally on $\{\{y_{it}\}_{t=1}^T\}_{i=1}^N$ almost surely. We showed that the first, second, and third moments of $g(\hat{\theta}_i^*)$ satisfy Lyapunov's conditions in probability. For any subsequence of the original sequence, there thus exists a further subsequence under which these moment conditions are satisfied almost surely. Thus, under a subsequence of any subsequence, $\sqrt{N}(\hat{G}^* - \hat{G})$ converges in distribution to $X \sim \mathcal{N}(0, \Gamma)$ conditionally almost surely. This implies that for any subsequence, there exists a further subsequence under which $\sup_{x\in\mathbb{R}}\left|P^*\left(\sqrt{N}(\hat{G}^* - \hat{G}) \leq x\right) - \Pr(X \leq x)\right|$ converges to 0 almost surely. It thus holds that, for the original sequence, $\sup_{x\in\mathbb{R}}|P^*(\sqrt{N}(\hat{G}^* - \hat{G}) \leq x) - \Pr(X \leq x)| \xrightarrow{p} 0$. We note that this argument holds for all monotonic diagonal paths $N \to \infty, T(N) \to \infty$. Hence, as stated in REMARKS (a) in Phillips and Moon (1999), it also holds under double asymptotics $N, T \to \infty$.

Next, we consider $\hat{S}^*$. By Taylor's theorem, we have

$$\sqrt{N}(\hat{S}^* - \hat{S}) = (\nabla h_1(\tilde{G}^{(1)*})^\top, \nabla h_2(\tilde{G}^{(2)*})^\top, \dots, \nabla h_n(\tilde{G}^{(n)*})^\top)^\top \sqrt{N}(\hat{G}^* - \hat{G}),$$

where $\tilde{G}^{(p)*}$ is between $\hat{G}^*$ and $\hat{G}$ for $p = 1, 2, \dots, n$. It is easy to see that $\tilde{G}^{(p)*} = G + o_p(1)$

conditionally, which implies that $\tilde{G}^{(p)*} = G + o_p(1)$ unconditionally as well (Cheng and Huang, 2010, Lemma 3). It thus holds that $\sqrt{N}(\hat{S}^* - \hat{S}) = \nabla h(G)\sqrt{N}(\hat{G}^* - \hat{G}) + o_p(1)$. The rest of the proof follows the same argument for $\hat{G}^*$ and we obtain the desired result. □

**Theorem 6.** *Suppose that the assumptions in Theorem 1 hold. When $N, T \to \infty$, it holds that*

$$\sup_{x\in\mathbb{R}} \left| P^* \left( \sqrt{N} \left( \mathbb{F}_N^*(a) - \mathbb{F}_N(a) \right) \leq x \right) - \Pr \left( \mathcal{N}\left(0, F(a)(1 - F(a))\right) \leq x \right) \right| \xrightarrow{p} 0.$$

*Proof.* It is sufficient to show Lyapunov's conditions. Let $F_0 = F_0^\xi$ be the CDF of $\xi_i$. It is clear that $E^*(\mathbf{1}(\hat{\xi}_i^* \leq a)) = N^{-1}\sum_{i=1}^N \mathbf{1}(\hat{\xi}_i \leq a)$ and that $var^*(\mathbf{1}(\hat{\xi}_i^* \leq a)) = N^{-1}\sum_{i=1}^N \mathbf{1}(\hat{\xi}_i \leq a) - (N^{-1}\sum_{i=1}^N \mathbf{1}(\hat{\xi}_i \leq a))^2 \xrightarrow{p} F_0(a)(1 - F_0(a))$ by Theorem 1 and the continuous mapping theorem. For the third moment, we have $N^{-1/2}E^*|\mathbf{1}(\hat{\xi}_i^* \leq a)|^3 = N^{-3/2}\sum_{i=1}^N \mathbf{1}(\hat{\xi}_i \leq a) \xrightarrow{p} 0 \cdot F_0(a) = 0$ by Theorem 1 and Slutsky's theorem. Therefore, we have the statement by the same argument in the proof of Theorem 5. □

## E.3 Proofs of lemmas omitted from the main text

**Lemma 3.** *Let $r$ be an even natural number. Suppose that Assumptions 1, 2, and 3 hold for $r_m = r$ and $r_d = r$. Then, it holds that $E((\bar{w}_i)^r) \leq CT^{-r/2}$.*

*Proof.* We first consider the case with $r = 2$. Given $E(\bar{w}_i|i) = 0$, Lemma 1 states that $E((\bar{w}_i)^2|i) \leq C_i/T$ where $C_i = 12(E(|w_{it}|^{(4+\delta)/2}|i))^{4/(4+\delta)}\sum_{m=0}^\infty \alpha(m|i)^{\delta/(4+\delta)}$. Assumption 2 implies that $C_i \leq 12(E(|w_{it}|^{(4+\delta)/2}|i))^{4/(4+\delta)}\sum_{m=0}^\infty \alpha(m)^{\delta/(4+\delta)}$. Thus, we have

$$\begin{aligned}
E\left((\bar{w}_i)^2\right) &= E\left(E\left((\bar{w}_i)^2|i\right)\right) \\
&\leq 12E\left((E(|w_{it}|^{(4+\delta)/2}|i))^{4/(4+\delta)}\right)\sum_{m=0}^\infty \alpha(m)^{\delta/(4+\delta)}/T \\
&\leq 12\left(E\left(E(|w_{it}|^{(4+\delta)/2}|i)\right)\right)^{4/(4+\delta)}\sum_{m=0}^\infty \alpha(m)^{\delta/(4+\delta)}/T \\
&= 12\left(E\left(|w_{it}|^{(4+\delta)/2}\right)\right)^{4/(4+\delta)}\sum_{m=0}^\infty \alpha(m)^{\delta/(4+\delta)}/T \\
&= O\left(\frac{1}{T}\right),
\end{aligned}$$

where the second inequality is Jensen's inequality and the last equality follows from Assumptions 2 and 3. Hence, the desired result holds for $r = 2$.

Next, we consider the case with $r > 2$. We use Lemma 2. From the proof of Lemma 2 available in Yokoyama (1980), we have

$$E\left(\left|\sum_{t=1}^{T} w_{it}\right|^r |i\right) \le K_{r,i}\left(E\left(|w_{it}|^{r+\delta}|i\right)\right)^{r/(r+\delta)} T^{r/2},$$

for some $\delta > 0$, where $K_{r,i}$ is a polynomial of $A_q(\alpha|i)$ for $q \le r$ and $A_q(\alpha|i) := \sum_{m=0}^{\infty}(m+1)^{q/2-1}\alpha(m|i)^{\delta/(q+\delta)}$. Note that $A_q(\alpha|i) < \infty$ for $q \le r$ if $A_r(\alpha|i) < \infty$. By Assumption 2, there exists a constant $K_r < \infty$ such that $K_{r,i} < K_r$ for all $i$. Thus, we have

$$\begin{aligned}
E\left((\bar{w}_i)^r\right) = E\left(E\left((\bar{w}_i)^r|i\right)\right) &\le K_r E\left(\left(E\left(|w_{it}|^{r+\delta}|i\right)\right)^{r/(r+\delta)}\right) T^{-r/2} \\
&\le K_r\left(E\left(E\left(|w_{it}|^{r+\delta}|i\right)\right)\right)^{r/(r+\delta)} T^{-r/2} \\
&= K_r\left(E\left(|w_{it}|^{r+\delta}\right)\right)^{r/(r+\delta)} T^{-r/2} \\
&= O(T^{-r/2}),
\end{aligned}$$

where the second inequality is Jensen's inequality and the last equality follows from Assumption 3. The proof for $r > 2$ is complete. □

**Lemma 6.** *Let $r$ be an even natural number. Suppose that Assumptions 1, 2, and 3 hold for $r_m = 2r$ and $r_d = 2r$. Then, we have $E((\hat{\gamma}_{k,i} - \gamma_{k,i})^r) = O(T^{-r/2})$.*

*Proof.* We have

$$\begin{aligned}
E((\hat{\gamma}_{k,i} - \gamma_{k,i})^r) =& E\Bigg(\Bigg(\frac{1}{T-k}\sum_{t=k+1}^{T}(w_{it}w_{i,t-k} - \gamma_{k,i}) - \frac{T+k}{T-k}(\bar{w}_i)^2 \\
&+ \frac{1}{T-k}\sum_{t=1}^{k} w_{it}\bar{w}_i + \frac{1}{T-k}\sum_{t=T-k+1}^{T} w_{it}\bar{w}_i\Bigg)^r\Bigg).
\end{aligned} \tag{S15}$$

Thanks to Loéve's $c_r$ inequality, we only need examine the $r$-order moment of each term in paren-

theses on the right-hand side of (S15). For the first term, Lemma 5 leads to

$$E\left(\left(\frac{1}{T-k}\sum_{t=k+1}^{T}(w_{it}w_{i,t-k}-\gamma_{k,i})\right)^r\right)=O\left(T^{-r/2}\right).$$

For the second term in (S15), we first note that $(T+k)/(T-k)=O(1)$. We observe that $E(((\bar{w}_i)^2)^r)=E((\bar{w}_i)^{2r})=O(T^{-r})$ by Lemma 3. We thus have that

$$E\left(\left(\frac{T+k}{T-k}(\bar{w}_i)^2\right)^r\right)=O\left(T^{-r}\right).$$

For the third term, we first observe that by the Cauchy–Schwarz inequality,

$$\begin{aligned}E\left(\left(\frac{1}{T-k}\sum_{t=1}^{k}w_{it}\bar{w}_i\right)^r\right)&=E\left((\bar{w}_i)^r\left(\frac{1}{T-k}\sum_{t=1}^{k}w_{it}\right)^r\right)\\&\leq\left(E\left((\bar{w}_i)^{2r}\right)\right)^{1/2}\left(E\left(\left(\frac{1}{T-k}\sum_{t=1}^{k}w_{it}\right)^{2r}\right)\right)^{1/2}.\end{aligned}$$

It is shown in the discussion on the second term that $E\left((\bar{w}_i)^{2r}\right)$ is of order $T^{-r}$. Moreover, because $k$ is fixed, it is easy to see that $E(((T-k)^{-1}\sum_{t=1}^{k}w_{it})^{2r}=O(T^{-2r})$. Therefore, it holds that $E(((T-k)^{-1}\sum_{t=1}^{k}w_{it}\bar{w}_i)^r)=O(T^{-3r/2})$. We can use the same argument to show that $E(((T-k)^{-1}\sum_{t=T-k+1}^{T}w_{it}\bar{w}_i)^r)=O(T^{-3r/2})$. Thus, we have shown the desired result. □

**Lemma 9.** *Suppose that Assumptions 1, 2, 3, and 5 hold for* $r_m=8$ *and* $r_d=8$*. Let* $P_T=P_T^{\hat{\gamma}_k}$ *and* $P_0=P_0^{\gamma_k}$ *be the probability measures of* $\hat{\gamma}_{k,i}$ *and* $\gamma_{k,i}$*, respectively. It holds that* $\sup_{f\in\mathcal{F}}|P_Tf-P_0f|=O(T^{-2/(3+\epsilon)})$ *for any* $\epsilon\in(0,1/3)$*.*

*Proof.* Consider $\hat{\gamma}_{k,j}$, $\tilde{\gamma}_{k,j}:=\hat{\gamma}_{k,j}+z$, and $\check{\gamma}_{k,j}:=\gamma_{k,j}+z$ where $z\sim\mathcal{N}(0,\sigma^2)$ and $z$ is independent of $(\alpha_j,\{w_{jt}\}_{t=1}^T)$. The result follows by the same arguments for the proof of $\mu_j$ in Lemma 8 if we show that $|\tilde{F}_T(a)-\check{F}(a)|=O(T^{-2/(3+\epsilon)})$ where $\tilde{F}_T(a)=\Pr(\tilde{\gamma}_{k,j}\leq a)$ and $\check{F}(a)=\Pr(\check{\gamma}_{k,j}\leq a)$ are the CDFs at $a\in\mathbb{R}$.

We first note that the characteristic functions of $\check{\gamma}_{k,j}$ and $\tilde{\gamma}_{k,j}$ are $\psi_{\check{\gamma}_k}(\zeta)=\exp(-\sigma^2\zeta^2/2)\psi_{\gamma_k}(\zeta)$ and $\psi_{\tilde{\gamma}_k}(\zeta)=\exp(-\sigma^2\zeta^2/2)\psi_{\hat{\gamma}_k}(\zeta)$, respectively. Here, we observe that $\psi_{\hat{\gamma}_k}(\zeta)=E[\exp(i\zeta\hat{\gamma}_{k,j})]=$

$E[\exp(i\zeta\gamma_{k,j})\exp(i\zeta(\hat{\gamma}_{k,j}-\gamma_{k,j}))]$. Taylor's theorem leads to

$$\exp(i\zeta(\hat{\gamma}_{k,j}-\gamma_{k,j})) = 1 + i\zeta(\hat{\gamma}_{k,j}-\gamma_{k,j}) - \frac{1}{2}\zeta^2(\hat{\gamma}_{k,j}-\gamma_{k,j})^2 - \frac{1}{3!}i\zeta^3(\hat{\gamma}_{k,j}-\gamma_{k,j})^3\exp(i\zeta c),$$

where $c$ is between $\hat{\gamma}_{k,j}-\gamma_{k,j}$ and 0. Hence, it holds that

$$\begin{aligned}\psi_{\tilde{\gamma}_k}(\zeta) =& \exp\left(-\frac{1}{2}\sigma^2\zeta^2\right)\Bigg(\psi_{\gamma_k}(\zeta) + i\zeta E[(\hat{\gamma}_{k,j}-\gamma_{k,j})\exp(i\zeta\gamma_{k,j})] \\ &- \frac{1}{2}\zeta^2 E[(\hat{\gamma}_{k,j}-\gamma_{k,j})^2\exp(i\zeta\gamma_{k,j})] - \frac{1}{3!}i\zeta^3 E[(\hat{\gamma}_{k,j}-\gamma_{k,j})^3\exp(i\zeta c)\exp(i\zeta\gamma_{k,j})]\Bigg).\end{aligned}$$

By the inversion theorem and the same procedure for the proof of $\mu_j$, we have

$$\begin{aligned}\check{F}(a) - \tilde{F}_T(a) =& \frac{1}{\pi}\int_{-\infty}^{\infty}\frac{e^{-i\zeta a}}{i\zeta}\exp\left(-\frac{1}{2}\sigma^2\zeta^2\right)\left(i\zeta E\left[(\hat{\gamma}_{k,j}-\gamma_{k,j})\exp\left(i\zeta\gamma_{k,j}\right)\right]\right)d\zeta \\ &+ \frac{1}{\pi}\int_{-\infty}^{\infty}\frac{e^{-i\zeta a}}{i\zeta}\exp\left(-\frac{1}{2}\sigma^2\zeta^2\right)\left(-\frac{1}{2}\zeta^2 E\left[(\hat{\gamma}_{k,j}-\gamma_{k,j})^2\exp\left(i\zeta\gamma_{k,j}\right)\right]\right)d\zeta \\ &+ \frac{1}{\pi}\int_{-\infty}^{\infty}\frac{e^{-i\zeta a}}{i\zeta}\exp\left(-\frac{1}{2}\sigma^2\zeta^2\right)\left(-\frac{1}{3!}i\zeta^3 E\left[(\hat{\gamma}_{k,j}-\gamma_{k,j})^3\exp\left(i\zeta c\right)\right]\right)d\zeta.\end{aligned} \tag{S16}$$

For the first line of (S16), we have

$$\begin{aligned}&\frac{1}{\pi}\int_{-\infty}^{\infty}\frac{e^{-i\zeta a}}{i\zeta}\exp\left(-\frac{1}{2}\sigma^2\zeta^2\right)\left(i\zeta E\left[(\hat{\gamma}_{k,j}-\gamma_{k,j})\exp(i\zeta\gamma_{k,j})\right]\right)d\zeta \\ =&\frac{1}{\pi}E\left[(\hat{\gamma}_{k,j}-\gamma_{k,j})\int_{-\infty}^{\infty}\exp(i\zeta(\gamma_{k,j}-a))\exp\left(-\frac{1}{2}\sigma^2\zeta^2\right)d\zeta\right].\end{aligned}$$

We observe that the integral is

$$\int_{-\infty}^{\infty}\exp(i\zeta(\gamma_{k,j}-a))\exp\left(-\frac{1}{2}\sigma^2\zeta^2\right)d\zeta = \frac{\sqrt{2\pi}}{\sigma}\exp\left(-\frac{(\gamma_{k,j}-a)^2}{2\sigma^2}\right).$$

Hence, we can show that

$$\begin{aligned}\text{The first line of (S16)} &= E\left[(\hat{\gamma}_{k,j}-\gamma_{k,j})\frac{\sqrt{2\pi}}{\sigma}\exp\left(-\frac{(\gamma_{k,j}-a)^2}{2\sigma^2}\right)\right] \\ &= E\left[(\bar{w}_j)^2\frac{\sqrt{2\pi}}{\sigma}\exp\left(-\frac{(\gamma_{k,j}-a)^2}{2\sigma^2}\right)\right] + o\left(\frac{A_\sigma}{\sigma T}\right),\end{aligned}$$

by the expansion of $(\hat{\gamma}_{k,j} - \gamma_{k,j})$, the law of iterated expectations, and the following observation. However, the mean in the above equation is analogous to the equation in the proof of $\mu_j$, so that we can evaluate it by the same arguments. As a result, we obtain that the first line of (S16) is of order $O(A_\sigma/(\sigma T))$ for $A_\sigma = \sigma^{1-\epsilon'}$ for any $0 < \epsilon' < 1$ by Assumption 5.d.

Similarly, we can show that the second and third lines of (S16) are of orders $O(A_\sigma^2/(\sigma^3 T))$ and $O(1/(\sigma^3 T^{3/2}))$, respectively, by the same arguments for the proof of $\mu_j$.

Hence, we have

$$\left|\tilde{F}_T(a) - \check{F}(a)\right| = O\left(\frac{A_\sigma}{\sigma T} + \frac{A_\sigma^2}{\sigma^3 T} + \frac{1}{\sigma^3 T^{3/2}}\right),$$

uniformly over $a \in \mathbb{R}$. As well as the proof of $\mu_j$ for Lemma 8, by setting $A_\sigma = \sigma^{1-\epsilon'}$ and $\sigma = 1/T^{1/(3+2\epsilon')}$ for any $0 < \epsilon' < 1/6$, we obtain that $|\tilde{F}_T(a) - \check{F}(a)| = O(T^{-2/(3+2\epsilon')})$ uniformly over $a \in \mathbb{R}$. Therefore, we obtain that $\sup_{f\in\mathcal{F}} |P_T f - P_0 f| = O(T^{-2/(3+\epsilon)})$ for any $0 < \epsilon = 2\epsilon' < 1/3$. □

**Lemma 10.** *Suppose that Assumptions 1, 2, 3, and 6 hold for $r_m = 8$ and $r_d = 8$. Let $P_T = P_T^{\hat{\rho}_k}$ and $P_0 = P_0^{\rho_k}$ be the probability measures of $\hat{\rho}_{k,i}$ and $\rho_{k,i}$, respectively. It holds that $\sup_{f\in\mathcal{F}} |P_T f - P_0 f| = O(T^{-2/(3+\epsilon)})$ for any $\epsilon \in (0, 1/3)$.*

*Proof.* Consider $\hat{\rho}_{k,j}$, $\tilde{\rho}_{k,j} \coloneqq \hat{\rho}_{k,j} + z$, and $\check{\rho}_{k,j} \coloneqq \rho_{k,j} + z$ where $z \sim \mathcal{N}(0, \sigma^2)$ and $z$ is independent of $(\alpha_j, \{w_{jt}\}_{t=1}^T)$. The result follows by the same arguments for the proofs of $\mu_j$ and $\gamma_{k,j}$ in Lemmas 8 and 9 if we show that $|\tilde{F}_T(a) - \check{F}(a)| = O(T^{-2/(3+\epsilon)})$ where $\tilde{F}_T(a) = \Pr(\tilde{\rho}_{k,j} \le a)$ and $\check{F}(a) = \Pr(\check{\rho}_{k,j} \le a)$ are the CDFs at $a \in \mathbb{R}$.

To this end, we first note that the characteristic functions of $\check{\rho}_{k,j}$ and $\tilde{\rho}_{k,j}$ are $\psi_{\check{\rho}_k}(\zeta) = \exp(-\sigma^2\zeta^2/2)\psi_{\rho_k}(\zeta)$ and $\psi_{\tilde{\rho}_k}(\zeta) = \exp(-\sigma^2\zeta^2/2)E[\exp(i\zeta\hat{\rho}_{k,j})]$, respectively. Here, we observe that $E[\exp(i\zeta\hat{\rho}_{k,j})] = E[\exp(i\zeta\rho_{k,j})\exp(i\zeta(\hat{\rho}_{k,j} - \rho_{k,j}))]$. Taylor's theorem leads to

$$\exp(i\zeta(\hat{\rho}_{k,j} - \rho_{k,j})) = 1 + i\zeta(\hat{\rho}_{k,j} - \rho_{k,j}) - \frac{1}{2}\zeta^2(\hat{\rho}_{k,j} - \rho_{k,j})^2 - \frac{1}{6}i\zeta^3(\hat{\rho}_{k,j} - \rho_{k,j})^3\exp(i\zeta c),$$

where $c$ is between $\hat{\rho}_{k,j} - \rho_{k,j}$ and 0. Hence, it holds that

$$\psi_{\tilde{\rho}_k}(\zeta) = \exp\left(-\frac{1}{2}\sigma^2\zeta^2\right)\Bigg(\psi_{\rho_k}(\zeta) + i\zeta E[(\hat{\rho}_{k,j} - \rho_{k,j})\exp(i\zeta\rho_{k,j})]$$

$$- \frac{1}{2}\zeta^2 E[(\hat{\rho}_{k,j} - \rho_{k,j})^2 \exp(i\zeta\rho_{k,j})] - \frac{1}{3!} i\zeta^3 E[(\hat{\rho}_{k,j} - \rho_{k,j})^3 \exp(i\zeta c)\exp(i\zeta\rho_{k,j})] \Bigg).$$

By the inversion theorem and the same procedure for the proof of $\mu_j$, we have

$$\begin{aligned}
\check{F}(a) - \tilde{F}_T(a) =& \frac{1}{\pi}\int_{-\infty}^{\infty} \frac{e^{-i\zeta a}}{i\zeta} \exp\left(-\frac{1}{2}\sigma^2\zeta^2\right)\left(i\zeta E\left[(\hat{\rho}_{k,j} - \rho_{k,j})\exp\left(i\zeta\rho_{k,j}\right)\right]\right) d\zeta \\
&+ \frac{1}{\pi}\int_{-\infty}^{\infty} \frac{e^{-i\zeta a}}{i\zeta} \exp\left(-\frac{1}{2}\sigma^2\zeta^2\right)\left(-\frac{1}{2}\zeta^2 E\left[(\hat{\rho}_{k,j} - \rho_{k,j})^2 \exp\left(i\zeta\rho_{k,j}\right)\right]\right) d\zeta \qquad \text{(S17)} \\
&+ \frac{1}{\pi}\int_{-\infty}^{\infty} \frac{e^{-i\zeta a}}{i\zeta} \exp\left(-\frac{1}{2}\sigma^2\zeta^2\right)\left(-\frac{1}{3!} i\zeta^3 E\left[(\hat{\rho}_{k,j} - \rho_{k,j})^3 \exp\left(i\zeta c\right)\right]\right) d\zeta.
\end{aligned}$$

For the first line of (S17), we have

$$\begin{aligned}
&\frac{1}{\pi}\int_{-\infty}^{\infty} \frac{e^{-i\zeta a}}{i\zeta} \exp\left(-\frac{1}{2}\sigma^2\zeta^2\right)\left(i\zeta E((\hat{\rho}_{k,j} - \rho_{k,j})\exp(i\zeta\rho_{k,j}))\right) d\zeta \\
=& \frac{1}{\pi} E\left((\hat{\rho}_{k,j} - \rho_{k,j})\int_{-\infty}^{\infty} \exp(i\zeta(\rho_{k,j} - a)) \exp\left(-\frac{1}{2}\sigma^2\zeta^2\right) d\zeta\right).
\end{aligned}$$

Here, Taylor's theorem for multivariate functions show that

$$\begin{aligned}
\frac{\hat{\gamma}_{k,j}}{\hat{\gamma}_{0,j}} =& \frac{\gamma_{k,j}}{\gamma_{0,j}} \\
&+ (\hat{\gamma}_{k,j} - \gamma_{k,j})\frac{1}{\gamma_{0,j}} - (\hat{\gamma}_{0,j} - \gamma_{0,j})\frac{\gamma_{k,j}}{\gamma_{0,j}^2} \\
&- (\hat{\gamma}_{k,j} - \gamma_{k,j})(\hat{\gamma}_{0,j} - \gamma_{0,j})\int_0^1 \frac{1}{\hat{\gamma}_{0,j} + t(\hat{\gamma}_{0,j} - \gamma_{0,j})} dt + (\hat{\gamma}_{0,j} - \gamma_{0,j})^2 \int_0^1 \frac{\hat{\gamma}_{k,j} + t(\hat{\gamma}_{k,j} - \gamma_{k,j})}{(\hat{\gamma}_{0,j} + t(\hat{\gamma}_{0,j} - \gamma_{0,j}))^3} dt.
\end{aligned}$$

Note that $E[(\hat{\gamma}_{k,j} - \gamma_{k,j})|j] = O(1/T)$ by the expansion of $\hat{\gamma}_{k,j}$ and $E[(\hat{\gamma}_{k,j} - \gamma_{k,j})^2] = O(1/T)$ by Lemma 6. Hence, because the integrals in the remainder terms are bounded almost surely by Assumption 6.e, the first line of (S17) is of order $O(A_\sigma/(\sigma T))$ for $A_\sigma = \sigma^{1-\epsilon'}$ with any $0 < \epsilon' < 1$ by the same arguments for the proof of $\gamma_{k,j}$. Note that Assumption 6.d is also used here.

For the second and third lines, we can show that they are of order $O(A_\sigma^2/(\sigma^3 T))$ and $O(1/(\sigma^3 T^{3/2}))$ by the same arguments for the proof of $\gamma_{k,j}$.

Hence, we have

$$\left|\tilde{F}_T(a) - \check{F}(a)\right| = O\left(\frac{A_\sigma}{\sigma T} + \frac{A_\sigma^2}{\sigma^3 T} + \frac{1}{\sigma^3 T^{3/2}}\right),$$

uniformly over $a \in \mathbb{R}$. As well as the proofs of $\mu_j$ and $\gamma_{k,j}$ for Lemmas 8 and 9, by setting $A_\sigma = \sigma^{1-\epsilon'}$ and $\sigma = 1/T^{1/(3+2\epsilon')}$ for any $0 < \epsilon' < 1/6$, we obtain that $|\tilde{F}_T(a) - \check{F}(a)| = O(T^{-2/(3+2\epsilon')})$ uniformly over $a \in \mathbb{R}$. Therefore, we obtain that $\sup_{f \in \mathcal{F}} |P_T f - P_0 f| = O(T^{-2/(3+\epsilon)})$ for any $0 < \epsilon = 2\epsilon' < 1/3$. □

# F Appendix: Additional empirical applications

This appendix presents the results of two additional empirical applications: earnings dynamics and productivity dynamics.

In the tables in this section, ED refers to the estimator based on the empirical distribution without the bias correction, HPJ to the half-panel jackknife bias-corrected estimator, and TOJ to the third-order jackknife bias-corrected estimator. The 95% confidence intervals below are computed using the cross-sectional bootstrap.

## F.1 Earnings dynamics

We study the properties of earnings dynamics without relying on any specific models. Earnings (or income) dynamics are an important research theme in economics for applications such as policy implications on earnings (see, e.g., Meghir and Pistaferri, 2011 for a review). We examine the distribution of quantities that describe the earnings dynamics. We find that the earnings dynamics have considerable heterogeneity. Our model-free analysis supports the empirical results in Browning et al. (2010) and Ejrnæs and Browning (2014) which find that the determinants of the income process are significantly heterogeneous.[S2]

We use a panel data set of white male workers' income extracted from the Panel Study of Income Dynamics. The data were originally prepared by Meghir and Pistaferri (2004) and we use a subsample of the version created by Browning et al. (2010). Ejrnæs and Browning (2014) also uses this version of the data. We draw a subsample consisting of individuals without any missing values in earnings between 1967 and 1978, a sample of $N = 393$ individuals. The time series is $T = 12$ long; $t = 1$ refers to the year 1967 and $t = 12$ refers to 1978.

[S2] We also note that heterogeneous volatilities of income process have been investigated by, for example, Meghir and Pistaferri (2004), Hospido (2012) and Botosaru and Sasaki (2018).

Table S1: Distribution of earnings dynamics

(a) Distributions of $\mu$, $\gamma_0$, and $\rho_1$

| | mean | std | Q25 | Q50 | Q75 |
|---|---|---|---|---|---|
| **Distribution of $\mu$** | | | | | |
| ED | 0.022 | 0.364 | -0.200 | 0.049 | 0.281 |
| 95% CI | [-0.012, 0.059] | [0.320, 0.415] | [-0.231, -0.156] | [-0.004, 0.093] | [0.243, 0.314] |
| HPJ | 0.022 | 0.351 | -0.206 | 0.054 | 0.275 |
| 95% CI | [-0.013, 0.060] | [0.304, 0.408] | [-0.237, -0.142] | [-0.024, 0.095] | [0.240, 0.320] |
| TOJ | 0.022 | 0.343 | -0.214 | 0.052 | 0.260 |
| 95% CI | [-0.014, 0.058] | [0.299, 0.400] | [-0.266, -0.101] | [-0.059, 0.112] | [0.209, 0.344] |
| **Distribution of $\gamma_0$** | | | | | |
| ED | 0.043 | 0.131 | 0.009 | 0.018 | 0.037 |
| 95% CI | [0.032, 0.058] | [0.048, 0.211] | [0.007, 0.010] | [0.015, 0.021] | [0.032, 0.043] |
| HPJ | 0.052 | 0.125 | 0.013 | 0.027 | 0.052 |
| 95% CI | [0.040, 0.069] | [0.043, 0.208] | [0.010, 0.015] | [0.021, 0.032] | [0.043, 0.060] |
| TOJ | 0.058 | 0.101 | 0.017 | 0.034 | 0.062 |
| 95% CI | [0.046, 0.075] | [0.032, 0.188] | [0.013, 0.020] | [0.025, 0.042] | [0.047, 0.076] |
| **Distribution of $\rho_1$** | | | | | |
| ED | 0.289 | 0.303 | 0.076 | 0.297 | 0.527 |
| 95% CI | [0.258, 0.318] | [0.283, 0.321] | [0.018, 0.122] | [0.253, 0.339] | [0.492, 0.563] |
| HPJ | 0.542 | 0.246 | 0.361 | 0.521 | 0.753 |
| 95% CI | [0.491, 0.595] | [0.209, 0.278] | [0.254, 0.438] | [0.438, 0.600] | [0.676, 0.823] |
| TOJ | 0.582 | 0.173 | 0.456 | 0.478 | 0.804 |
| 95% CI | [0.488, 0.680] | [0.106, 0.246] | [0.242, 0.621] | [0.333, 0.659] | [0.647, 0.963] |

(b) Correlation structure

| | $\mu$ vs $\gamma_0$ | $\mu$ vs $\rho_1$ | $\gamma_0$ vs $\rho_1$ |
|---|---|---|---|
| ED | -0.253 | 0.079 | -0.040 |
| 95% CI | [-0.351, -0.182] | [-0.043, 0.179] | [-0.094, 0.078] |
| HPJ | -0.217 | 0.120 | -0.074 |
| 95% CI | [-0.351, -0.173] | [-0.079, 0.311] | [-0.168, 0.091] |
| TOJ | -0.162 | 0.112 | -0.124 |
| 95% CI | [-0.396, -0.100] | [-0.220, 0.417] | [-0.289, 0.126] |

We investigate the distribution of individual means, variances, and first-order autocorrelations of residual log earnings. We obtain the residuals by regressing log earnings on year and age dummies. We run the regressions for three educational categories (high school dropouts, high school graduates, and college graduates).

Table S1 summarizes the distributional features of the means, variances, and first-order autocorrelations. We also estimate the correlations between these three quantities.

The results show that the earnings dynamics have considerable heterogeneity. They also show that the HPJ and TOJ estimates can be very different from the ED estimates, and the bias-corrected estimates imply more persistent dynamics than those implied by the ED estimates. Our estimates imply that the variances of income shocks are markedly heterogeneous with a skewed distribution,

which is consistent with Browning et al.'s (2010) findings. The results also indicate that individuals with high permanent earnings face relatively small shocks (in percentage terms). One may have the impression that the persistency of an earnings shock is positively associated with the level of permanent earnings and negatively with the magnitude of income shocks. However, there is no statistical evidence for this conclusion.

We next examine whether the distribution of the means is normal. This is of interest because it is common to model the distribution of earnings using a lognormal distribution. Horowitz and Markatou (1996) find that the permanent component of income process is well approximated by a normal distribution. As an intuitive investigation, Figure S1 provides the QQ plot of the means of earnings against the normal distribution with the same mean and standard deviation. Formally, the Kolmogorov–Smirnov test cannot reject the null of normality (or lognormality of earnings) given a test statistic of 0.04 and a $p$-value of 0.7. These results suggest that the lognormal approximation of earnings might be reasonable.

Finally, we examine whether the distribution of earnings dynamics differs according to distinct educational attainments. In particular, we investigate whether the distribution of the first-order autocorrelations for high school graduates differs from that of college graduates. In our sample, there are 186 high school graduates and 89 college graduates. Table S2 summarizes the distribution of the first-order autocorrelations of high school graduates and that of college graduates and Figure S2 provides the QQ plot.[S3] These indicate that college graduates face more persistent earnings shocks than high school graduates. Moreover, the first-order autocorrelations of earnings for college graduates are relatively more concentrated (i.e., more homogeneous) than those for high school graduates. However, the value of the two-sample Kolmogorov–Smirnov test is 0.1 with a $p$-value of 0.4. There is no statistical evidence that high school and college graduates face different earnings dynamics.

## F.2 Productivity dynamics

Our second application examines the total factor productivity (TFP) dynamics of Chilean firms.

Our analysis is based on plant-level panel data on productivity in the Chilean food industry

[S3] TOJ bias-corrected estimates for the quantiles in Table S2 are non-monotonic as a consequence of bias correction, but this issue can be corrected by using the rearrangement in Chernozhukov, Fernandez-Val, and Galichon (2009).

Table S2: Distributions of $\rho_1$ for earnings dynamics of high school and college graduates

| | mean | std | Q25 | Q50 | Q75 |
|---|---|---|---|---|---|
| **High school graduates** | | | | | |
| ED | 0.296 | 0.300 | 0.064 | 0.317 | 0.527 |
| 95% CI | [0.252, 0.336] | [0.273, 0.325] | [0.001, 0.137] | [0.262, 0.360] | [0.456, 0.581] |
| HPJ | 0.539 | 0.250 | 0.295 | 0.544 | 0.752 |
| 95% CI | [0.468, 0.608] | [0.204, 0.299] | [0.165, 0.426] | [0.444, 0.638] | [0.635, 0.857] |
| TOJ | 0.529 | 0.195 | 0.248 | 0.470 | 0.790 |
| 95% CI | [0.396, 0.665] | [0.085, 0.297] | [0.006, 0.489] | [0.270, 0.709] | [0.541, 1.017] |
| **College graduates** | | | | | |
| ED | 0.341 | 0.281 | 0.158 | 0.366 | 0.551 |
| 95% CI | [0.286, 0.397] | [0.247, 0.311] | [0.078, 0.194] | [0.236, 0.421] | [0.517, 0.630] |
| HPJ | 0.625 | 0.191 | 0.574 | 0.643 | 0.779 |
| 95% CI | [0.530, 0.724] | [0.124, 0.258] | [0.362, 0.675] | [0.435, 0.789] | [0.672, 0.923] |
| TOJ | 0.727 | 0.056 | 1.001 | 0.727 | 0.844 |
| 95% CI | [0.518, 0.958] | [-0.103, 0.198] | [0.500, 1.294] | [0.339, 1.103] | [0.538, 1.126] |

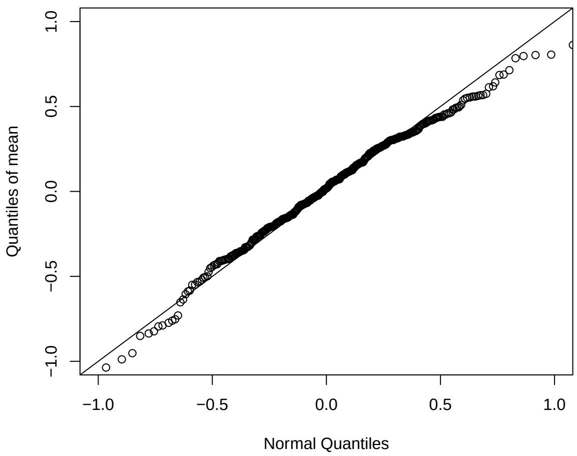


Figure S1: QQ plot of mean earnings against the normal distribution

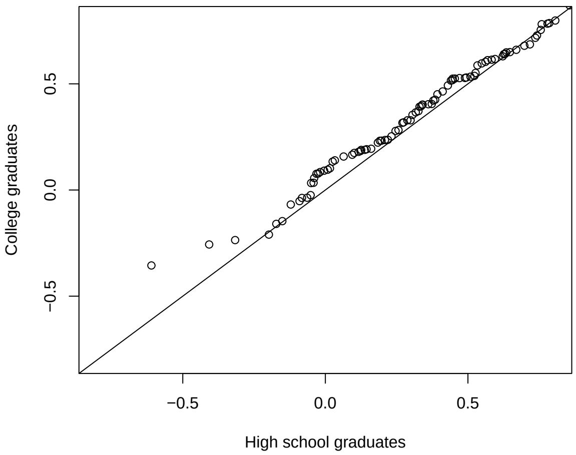


Figure S2: The QQ plot for $\rho_1$

(Industry 311). Levinsohn and Petrin (2003), Balat, Brambilla, and Sasaki (2016), and others also use this data set, and Balat et al. (2016) provides detailed information about the data.[S4] We use the TFP data computed using the method in Levinsohn and Petrin (2003). We employ a subsample consisting of firms with no missing observations in the entire sample period.[S5]

[S4] Yuya Sasaki kindly agreed to share the TFP series extracted from his data set with the authors.

[S5] While Balat et al. (2016) also compute TFPs, they use different time periods and a different method. Note also that Levinsohn and Petrin (2003) use a similar data set but their TFP values are slightly different. Note that there exists a considerable body of literature on the estimation of production functions and productivity; see, for example, Griliches and Mairesse (1998) and Ackerberg, Benkard, Berry, and Pakes (2007) for literature reviews. The main challenge for the structural identification and estimation is the endogeneity problem due to the fact that firms

In this application, $y_{it}$ is the TFP of firm $i$ at time $t$. The cross-sectional sample size is $N = 465$. The length of time series is $T = 18$: $t = 1$ refers to year 1979 and $t = 18$ refers to year 1996. The observations are in 1980 Chilean pesos.

Table S3 summarizes the distributional features of the heterogeneous means, variances, and first-order autocorrelations. We also estimate the correlations between these three quantities. The results show that the productivity dynamics have considerable heterogeneity and firms with high permanent productivity face relatively large shocks. We also obtain a slightly insignificant (at the 5% level) result that firms facing large shocks may not suffer (or benefit) from these shocks for long. In addition, the HPJ and TOJ estimates differ markedly from the ED estimates, in particular for the first-order autocorrelation.

# G Appendix: Additional Monte Carlo simulations

This appendix presents additional Monte Carlo simulation results that complement the simulation results presented in the main body. Here, we base the simulation designs on our empirical applications.

In this section, ED refers to the estimator based on the empirical distribution without the bias correction, HPJ to the half-panel jackknife bias-corrected estimator, and TOJ to the third-order jackknife bias-corrected estimator.

## G.1 Designs

We consider the same DGP as in the Monte Carlo simulation in the main body, except for sample sizes and joint distributions of unit-specific parameters $(\varsigma_i, \phi_i, \sigma_i^2)$. We consider three designs for joint distributions of $(\varsigma_i, \phi_i, \sigma_i^2)$ by imitating the HPJ estimates in our three empirical applications. Specifically, the joint distribution of $(\varsigma_i, \phi_i, \sigma_i^2)$ in design 1 of this simulation imitates the HPJ

select the optimal amount of inputs based on factors that econometricians do not observe. Many studies, including recent papers by Ackerberg, Caves, and Frazer (2015) and Gandhi, Navarro, and Rivers (2016), attempt to solve the problem to infer the structural implications on production functions and productivity. However, we do not discuss the issues regarding the estimation of production functions and productivity in this paper and focus on the heterogeneous dynamics of productivity measure which is obtained by a popular method of Levinsohn and Petrin (2003).

Table S3: Distribution of productivity dynamics

(a) Distributions of $\mu$, $\gamma_0$, and $\rho_1$

| | mean | std | Q25 | Q50 | Q75 |
|---|---|---|---|---|---|
| **Distribution of** $\mu$ | | | | | |
| ED | 2.958 | 0.292 | 2.750 | 2.863 | 3.142 |
| 95% CI | [2.932, 2.984] | [0.271, 0.313] | [2.730, 2.767] | [2.829, 2.877] | [3.047, 3.192] |
| HPJ | 2.958 | 0.284 | 2.755 | 2.864 | 3.159 |
| 95% CI | [2.933, 2.985] | [0.263, 0.304] | [2.734, 2.780] | [2.821, 2.875] | [3.029, 3.217] |
| TOJ | 2.958 | 0.279 | 2.748 | 2.867 | 3.191 |
| 95% CI | [2.931, 2.984] | [0.258, 0.300] | [2.720, 2.792] | [2.797, 2.889] | [3.005, 3.285] |
| **Distribution of** $\gamma_0$ | | | | | |
| ED | 0.035 | 0.039 | 0.014 | 0.024 | 0.037 |
| 95% CI | [0.032, 0.039] | [0.031, 0.047] | [0.013, 0.016] | [0.022, 0.025] | [0.034, 0.042] |
| HPJ | 0.041 | 0.034 | 0.019 | 0.030 | 0.042 |
| 95% CI | [0.036, 0.045] | [0.027, 0.041] | [0.017, 0.021] | [0.027, 0.033] | [0.037, 0.050] |
| TOJ | 0.039 | 0.026 | 0.021 | 0.033 | 0.036 |
| 95% CI | [0.035, 0.045] | [0.019, 0.036] | [0.017, 0.024] | [0.028, 0.038] | [0.027, 0.048] |
| **Distribution of** $\rho_1$ | | | | | |
| ED | 0.408 | 0.266 | 0.227 | 0.450 | 0.611 |
| 95% CI | [0.385, 0.434] | [0.250, 0.282] | [0.175, 0.270] | [0.419, 0.482] | [0.583, 0.635] |
| HPJ | 0.573 | 0.188 | 0.446 | 0.620 | 0.697 |
| 95% CI | [0.538, 0.607] | [0.157, 0.215] | [0.347, 0.519] | [0.572, 0.670] | [0.650, 0.736] |
| TOJ | 0.509 | 0.093 | 0.436 | 0.556 | 0.492 |
| 95% CI | [0.444, 0.573] | [0.029, 0.158] | [0.237, 0.576] | [0.464, 0.689] | [0.390, 0.590] |

(b) Correlation structure

| | $\mu$ vs $\gamma_0$ | $\mu$ vs $\rho_1$ | $\gamma_0$ vs $\rho_1$ |
|---|---|---|---|
| ED | 0.231 | -0.195 | -0.041 |
| 95% CI | [0.132, 0.329] | [-0.276, -0.105] | [-0.121, 0.057] |
| HPJ | 0.258 | -0.235 | -0.126 |
| 95% CI | [0.130, 0.370] | [-0.361, -0.109] | [-0.275, 0.009] |
| TOJ | 0.327 | -0.156 | -0.290 |
| 95% CI | [0.194, 0.480] | [-0.363, 0.045] | [-0.521, -0.076] |

estimates of the LOP application based on the truncated normal distribution:

$$\begin{pmatrix} \varsigma_i \\ \sigma_i^2 \\ \phi_i \end{pmatrix} \sim i.i.d.\,\mathcal{N}\left(\begin{pmatrix} -0.037 \\ 0.024 \\ 0.627 \end{pmatrix}, \begin{pmatrix} 0.120^2 & 0.082 \cdot 0.120 \cdot 0.019 & -0.160 \cdot 0.120 \cdot 0.159 \\ 0.082 \cdot 0.120 \cdot 0.019 & 0.019^2 & 0.106 \cdot 0.019 \cdot 0.159 \\ -0.160 \cdot 0.120 \cdot 0.159 & 0.106 \cdot 0.019 \cdot 0.159 & 0.159^2 \end{pmatrix}\right),$$

conditional on $\sigma_i^2 > 0$ and $|\phi_i| < 1$. Similarly, we imitate the HPJ estimates of the earnings and productivity dynamics for designs 2 and 3, respectively, in this simulation. For design 2, the

parameters are generated by

$$\begin{pmatrix} \varsigma_i \\ \sigma_i^2 \\ \phi_i \end{pmatrix} \sim i.i.d.\, \mathcal{N}\left( \begin{pmatrix} 0.022 \\ 0.052 \\ 0.542 \end{pmatrix}, \begin{pmatrix} 0.351^2 & -0.217 \cdot 0.351 \cdot 0.125 & 0.120 \cdot 0.351 \cdot 0.246 \\ -0.217 \cdot 0.351 \cdot 0.125 & 0.125^2 & -0.074 \cdot 0.125 \cdot 0.246 \\ 0.120 \cdot 0.351 \cdot 0.246 & -0.074 \cdot 0.125 \cdot 0.246 & 0.246^2 \end{pmatrix} \right),$$

conditional on $\sigma_i^2 > 0$ and $|\phi_i| < 1$. For design 3, the data generating process follows:

$$\begin{pmatrix} \varsigma_i \\ \sigma_i^2 \\ \phi_i \end{pmatrix} \sim i.i.d.\, \mathcal{N}\left( \begin{pmatrix} 2.958 \\ 0.041 \\ 0.573 \end{pmatrix}, \begin{pmatrix} 0.284^2 & 0.258 \cdot 0.284 \cdot 0.034 & -0.235 \cdot 0.284 \cdot 0.188 \\ 0.258 \cdot 0.284 \cdot 0.034 & 0.034^2 & -0.126 \cdot 0.034 \cdot 0.188 \\ -0.235 \cdot 0.284 \cdot 0.188 & -0.126 \cdot 0.034 \cdot 0.188 & 0.188^2 \end{pmatrix} \right),$$

conditional on $\sigma_i^2 > 0$ and $|\phi_i| < 1$. In each design, we consider several combinations of $N$ and $T$ (including the same sample size as the corresponding empirical application) as reported in the tables below.

## G.2 Results

Tables S4–S7, S8–S11, and S12–S15 summarize the results of Monte Carlo simulations for designs 1, 2, and 3, respectively. In all simulation designs, we observe similar results to the simulation results in the main body. The split-panel jackknife bias-corrected estimators outperform ED. ED has large biases in many situations, such as the quantities of $\rho_{1,i}$ in designs 2 and 3, especially when $T$ is small. The coverage probabilities of ED for many parameters also differ significantly from 0.95 due to large biases. The HPJ bias correction is successful for many parameters, but the coverage probabilities of HPJ are unsatisfactory in some cases, such as the quantities of $\gamma_{0,i}$ in design 1, especially when $T$ is small. This result is likely because of severity of higher order biases for estimating such highly nonlinear parameters with relatively small $T$. On the contrary, even when $T$ is small, TOJ corrects biases and the coverage probabilities of TOJ are good. Nonetheless, as we discuss in the main body, TOJ eliminates biases at the inevitable cost of inflating standard deviations, and the coverage probabilities for TOJ sometimes exceeds 0.95 for some quantiles.

Consequently, we conclude that one should employ the cross-sectional bootstrap inference based on the split-panel jackknife bias correction.

Table S4: Monte Carlo simulation results for $\mu$ in design 1

| | true | $N$ | $T$ | ED bias | ED rmse | ED cp | HPJ bias | HPJ rmse | HPJ cp | TOJ bias | TOJ rmse | TOJ cp |
|---|---|---|---|---|---|---|---|---|---|---|---|---|
| $\mu$ mean | −0.034 | 1224 | 36 | 0.000 | 0.004 | 0.949 | 0.000 | 0.004 | 0.951 | 0.000 | 0.004 | 0.952 |
| | −0.034 | 1224 | 72 | 0.000 | 0.004 | 0.943 | 0.000 | 0.004 | 0.942 | 0.000 | 0.004 | 0.942 |
| | −0.034 | 1224 | 144 | 0.000 | 0.004 | 0.946 | 0.000 | 0.004 | 0.946 | 0.000 | 0.004 | 0.947 |
| | −0.034 | 2448 | 36 | 0.000 | 0.003 | 0.949 | 0.000 | 0.003 | 0.950 | 0.000 | 0.003 | 0.950 |
| | −0.034 | 2448 | 72 | 0.000 | 0.003 | 0.948 | 0.000 | 0.003 | 0.946 | 0.000 | 0.003 | 0.947 |
| | −0.034 | 2448 | 144 | 0.000 | 0.003 | 0.943 | 0.000 | 0.003 | 0.944 | 0.000 | 0.003 | 0.943 |
| | −0.034 | 4896 | 36 | 0.000 | 0.002 | 0.951 | 0.000 | 0.002 | 0.954 | 0.000 | 0.002 | 0.953 |
| | −0.034 | 4896 | 72 | 0.000 | 0.002 | 0.954 | 0.000 | 0.002 | 0.954 | 0.000 | 0.002 | 0.952 |
| | −0.034 | 4896 | 144 | 0.000 | 0.002 | 0.953 | 0.000 | 0.002 | 0.953 | 0.000 | 0.002 | 0.952 |
| $\mu$ std | 0.120 | 1224 | 36 | 0.016 | 0.016 | 0.000 | 0.006 | 0.006 | 0.578 | 0.001 | 0.004 | 0.937 |
| | 0.120 | 1224 | 72 | 0.009 | 0.010 | 0.063 | 0.002 | 0.004 | 0.888 | 0.000 | 0.003 | 0.946 |
| | 0.120 | 1224 | 144 | 0.005 | 0.006 | 0.489 | 0.001 | 0.003 | 0.932 | 0.000 | 0.003 | 0.945 |
| | 0.120 | 2448 | 36 | 0.016 | 0.016 | 0.000 | 0.006 | 0.006 | 0.259 | 0.001 | 0.003 | 0.914 |
| | 0.120 | 2448 | 72 | 0.009 | 0.009 | 0.001 | 0.002 | 0.003 | 0.807 | 0.000 | 0.002 | 0.943 |
| | 0.120 | 2448 | 144 | 0.005 | 0.005 | 0.195 | 0.001 | 0.002 | 0.920 | 0.000 | 0.002 | 0.945 |
| | 0.120 | 4896 | 36 | 0.016 | 0.016 | 0.000 | 0.006 | 0.006 | 0.041 | 0.001 | 0.002 | 0.887 |
| | 0.120 | 4896 | 72 | 0.009 | 0.009 | 0.000 | 0.002 | 0.003 | 0.646 | 0.000 | 0.002 | 0.940 |
| | 0.120 | 4896 | 144 | 0.005 | 0.005 | 0.016 | 0.001 | 0.002 | 0.903 | 0.000 | 0.001 | 0.957 |
| $\mu$ 25%Q | −0.115 | 1224 | 36 | −0.009 | 0.011 | 0.570 | −0.003 | 0.007 | 0.936 | −0.001 | 0.011 | 0.978 |
| | −0.115 | 1224 | 72 | −0.005 | 0.007 | 0.802 | −0.001 | 0.006 | 0.952 | 0.000 | 0.010 | 0.979 |
| | −0.115 | 1224 | 144 | −0.003 | 0.006 | 0.913 | −0.001 | 0.006 | 0.957 | 0.000 | 0.009 | 0.979 |
| | −0.115 | 2448 | 36 | −0.009 | 0.010 | 0.268 | −0.003 | 0.006 | 0.910 | −0.001 | 0.008 | 0.969 |
| | −0.115 | 2448 | 72 | −0.005 | 0.006 | 0.672 | −0.001 | 0.005 | 0.949 | 0.000 | 0.007 | 0.973 |
| | −0.115 | 2448 | 144 | −0.003 | 0.004 | 0.870 | 0.000 | 0.004 | 0.957 | 0.000 | 0.006 | 0.973 |
| | −0.115 | 4896 | 36 | −0.009 | 0.010 | 0.050 | −0.003 | 0.005 | 0.855 | −0.001 | 0.005 | 0.963 |
| | −0.115 | 4896 | 72 | −0.005 | 0.006 | 0.418 | −0.001 | 0.003 | 0.935 | 0.000 | 0.005 | 0.966 |
| | −0.115 | 4896 | 144 | −0.003 | 0.004 | 0.765 | −0.001 | 0.003 | 0.947 | 0.000 | 0.004 | 0.964 |
| $\mu$ 50%Q | −0.034 | 1224 | 36 | 0.001 | 0.005 | 0.947 | 0.001 | 0.006 | 0.957 | 0.001 | 0.010 | 0.976 |
| | −0.034 | 1224 | 72 | 0.000 | 0.005 | 0.945 | 0.000 | 0.006 | 0.957 | 0.000 | 0.009 | 0.977 |
| | −0.034 | 1224 | 144 | 0.000 | 0.005 | 0.947 | 0.000 | 0.005 | 0.958 | 0.000 | 0.008 | 0.979 |
| | −0.034 | 2448 | 36 | 0.000 | 0.003 | 0.940 | 0.000 | 0.004 | 0.948 | 0.000 | 0.007 | 0.969 |
| | −0.034 | 2448 | 72 | 0.000 | 0.003 | 0.949 | 0.000 | 0.004 | 0.956 | 0.000 | 0.006 | 0.973 |
| | −0.034 | 2448 | 144 | 0.000 | 0.003 | 0.948 | 0.000 | 0.004 | 0.956 | 0.000 | 0.005 | 0.969 |
| | −0.034 | 4896 | 36 | 0.001 | 0.002 | 0.938 | 0.001 | 0.003 | 0.947 | 0.000 | 0.005 | 0.965 |
| | −0.034 | 4896 | 72 | 0.000 | 0.002 | 0.950 | 0.000 | 0.003 | 0.953 | 0.000 | 0.004 | 0.964 |
| | −0.034 | 4896 | 144 | 0.000 | 0.002 | 0.950 | 0.000 | 0.003 | 0.956 | 0.000 | 0.004 | 0.967 |
| $\mu$ 75%Q | 0.046 | 1224 | 36 | 0.010 | 0.011 | 0.520 | 0.004 | 0.007 | 0.930 | 0.001 | 0.011 | 0.976 |
| | 0.046 | 1224 | 72 | 0.006 | 0.008 | 0.791 | 0.001 | 0.006 | 0.950 | 0.000 | 0.010 | 0.978 |
| | 0.046 | 1224 | 144 | 0.003 | 0.006 | 0.897 | 0.001 | 0.006 | 0.954 | 0.000 | 0.009 | 0.977 |
| | 0.046 | 2448 | 36 | 0.010 | 0.011 | 0.227 | 0.004 | 0.006 | 0.887 | 0.001 | 0.008 | 0.965 |
| | 0.046 | 2448 | 72 | 0.006 | 0.007 | 0.620 | 0.002 | 0.005 | 0.937 | 0.000 | 0.007 | 0.972 |
| | 0.046 | 2448 | 144 | 0.003 | 0.005 | 0.834 | 0.001 | 0.004 | 0.953 | 0.000 | 0.006 | 0.975 |
| | 0.046 | 4896 | 36 | 0.010 | 0.010 | 0.026 | 0.004 | 0.005 | 0.799 | 0.001 | 0.005 | 0.964 |
| | 0.046 | 4896 | 72 | 0.006 | 0.006 | 0.341 | 0.002 | 0.003 | 0.927 | 0.000 | 0.005 | 0.965 |
| | 0.046 | 4896 | 144 | 0.003 | 0.004 | 0.736 | 0.001 | 0.003 | 0.944 | 0.000 | 0.004 | 0.964 |

Table S5: Monte Carlo simulation results for $\gamma_0$ in design 1

| | true | $N$ | $T$ | **ED** | | | **HPJ** | | | **TOJ** | | |
|---|---|---|---|---|---|---|---|---|---|---|---|---|
| | | | | bias | rmse | cp | bias | rmse | cp | bias | rmse | cp |
| $\gamma_0$ mean | 0.028 | 1224 | 36 | −0.004 | 0.004 | 0.000 | −0.001 | 0.001 | 0.533 | 0.000 | 0.001 | 0.936 |
| | 0.028 | 1224 | 72 | −0.002 | 0.002 | 0.004 | 0.000 | 0.001 | 0.861 | 0.000 | 0.001 | 0.947 |
| | 0.028 | 1224 | 144 | −0.001 | 0.001 | 0.272 | 0.000 | 0.001 | 0.934 | 0.000 | 0.001 | 0.948 |
| | 0.028 | 2448 | 36 | −0.004 | 0.004 | 0.000 | −0.001 | 0.001 | 0.229 | 0.000 | 0.001 | 0.934 |
| | 0.028 | 2448 | 72 | −0.002 | 0.002 | 0.000 | 0.000 | 0.001 | 0.782 | 0.000 | 0.000 | 0.942 |
| | 0.028 | 2448 | 144 | −0.001 | 0.001 | 0.042 | 0.000 | 0.000 | 0.912 | 0.000 | 0.000 | 0.946 |
| | 0.028 | 4896 | 36 | −0.004 | 0.004 | 0.000 | −0.001 | 0.001 | 0.036 | 0.000 | 0.000 | 0.927 |
| | 0.028 | 4896 | 72 | −0.002 | 0.002 | 0.000 | 0.000 | 0.001 | 0.637 | 0.000 | 0.000 | 0.946 |
| | 0.028 | 4896 | 144 | −0.001 | 0.001 | 0.000 | 0.000 | 0.000 | 0.891 | 0.000 | 0.000 | 0.949 |
| $\gamma_0$ std | 0.016 | 1224 | 36 | 0.001 | 0.001 | 0.365 | 0.001 | 0.002 | 0.564 | 0.001 | 0.002 | 0.920 |
| | 0.016 | 1224 | 72 | 0.001 | 0.001 | 0.511 | 0.001 | 0.001 | 0.861 | 0.000 | 0.001 | 0.944 |
| | 0.016 | 1224 | 144 | 0.001 | 0.001 | 0.713 | 0.000 | 0.001 | 0.927 | 0.000 | 0.001 | 0.938 |
| | 0.016 | 2448 | 36 | 0.001 | 0.001 | 0.095 | 0.001 | 0.001 | 0.276 | 0.001 | 0.001 | 0.898 |
| | 0.016 | 2448 | 72 | 0.001 | 0.001 | 0.197 | 0.001 | 0.001 | 0.710 | 0.000 | 0.001 | 0.943 |
| | 0.016 | 2448 | 144 | 0.001 | 0.001 | 0.490 | 0.000 | 0.000 | 0.902 | 0.000 | 0.000 | 0.940 |
| | 0.016 | 4896 | 36 | 0.001 | 0.001 | 0.005 | 0.001 | 0.001 | 0.042 | 0.001 | 0.001 | 0.833 |
| | 0.016 | 4896 | 72 | 0.001 | 0.001 | 0.015 | 0.001 | 0.001 | 0.461 | 0.000 | 0.000 | 0.940 |
| | 0.016 | 4896 | 144 | 0.001 | 0.001 | 0.181 | 0.000 | 0.000 | 0.832 | 0.000 | 0.000 | 0.940 |
| $\gamma_0$ 25%Q | 0.015 | 1224 | 36 | −0.004 | 0.004 | 0.000 | −0.002 | 0.002 | 0.205 | −0.001 | 0.001 | 0.938 |
| | 0.015 | 1224 | 72 | −0.003 | 0.003 | 0.001 | −0.001 | 0.001 | 0.814 | 0.000 | 0.001 | 0.968 |
| | 0.015 | 1224 | 144 | −0.001 | 0.002 | 0.251 | 0.000 | 0.001 | 0.934 | 0.000 | 0.001 | 0.976 |
| | 0.015 | 2448 | 36 | −0.004 | 0.004 | 0.000 | −0.002 | 0.002 | 0.019 | −0.001 | 0.001 | 0.888 |
| | 0.015 | 2448 | 72 | −0.003 | 0.003 | 0.000 | −0.001 | 0.001 | 0.665 | 0.000 | 0.001 | 0.963 |
| | 0.015 | 2448 | 144 | −0.001 | 0.001 | 0.034 | 0.000 | 0.001 | 0.924 | 0.000 | 0.001 | 0.972 |
| | 0.015 | 4896 | 36 | −0.004 | 0.004 | 0.000 | −0.002 | 0.002 | 0.000 | −0.001 | 0.001 | 0.813 |
| | 0.015 | 4896 | 72 | −0.003 | 0.003 | 0.000 | −0.001 | 0.001 | 0.409 | 0.000 | 0.001 | 0.960 |
| | 0.015 | 4896 | 144 | −0.001 | 0.001 | 0.001 | 0.000 | 0.000 | 0.876 | 0.000 | 0.000 | 0.963 |
| $\gamma_0$ 50%Q | 0.026 | 1224 | 36 | −0.006 | 0.006 | 0.000 | −0.002 | 0.003 | 0.164 | −0.001 | 0.002 | 0.923 |
| | 0.026 | 1224 | 72 | −0.004 | 0.004 | 0.000 | −0.001 | 0.001 | 0.740 | 0.000 | 0.001 | 0.968 |
| | 0.026 | 1224 | 144 | −0.002 | 0.002 | 0.078 | 0.000 | 0.001 | 0.916 | 0.000 | 0.001 | 0.973 |
| | 0.026 | 2448 | 36 | −0.006 | 0.006 | 0.000 | −0.002 | 0.003 | 0.010 | −0.001 | 0.001 | 0.880 |
| | 0.026 | 2448 | 72 | −0.004 | 0.004 | 0.000 | −0.001 | 0.001 | 0.544 | 0.000 | 0.001 | 0.956 |
| | 0.026 | 2448 | 144 | −0.002 | 0.002 | 0.003 | 0.000 | 0.001 | 0.876 | 0.000 | 0.001 | 0.966 |
| | 0.026 | 4896 | 36 | −0.006 | 0.006 | 0.000 | −0.002 | 0.003 | 0.000 | −0.001 | 0.001 | 0.794 |
| | 0.026 | 4896 | 72 | −0.004 | 0.004 | 0.000 | −0.001 | 0.001 | 0.243 | 0.000 | 0.001 | 0.947 |
| | 0.026 | 4896 | 144 | −0.002 | 0.002 | 0.000 | 0.000 | 0.001 | 0.804 | 0.000 | 0.001 | 0.965 |
| $\gamma_0$ 75%Q | 0.038 | 1224 | 36 | −0.006 | 0.006 | 0.000 | −0.002 | 0.002 | 0.669 | 0.000 | 0.002 | 0.965 |
| | 0.038 | 1224 | 72 | −0.003 | 0.004 | 0.007 | −0.001 | 0.001 | 0.885 | 0.000 | 0.002 | 0.969 |
| | 0.038 | 1224 | 144 | −0.002 | 0.002 | 0.278 | 0.000 | 0.001 | 0.938 | 0.000 | 0.002 | 0.977 |
| | 0.038 | 2448 | 36 | −0.006 | 0.006 | 0.000 | −0.002 | 0.002 | 0.409 | 0.000 | 0.002 | 0.943 |
| | 0.038 | 2448 | 72 | −0.003 | 0.004 | 0.000 | −0.001 | 0.001 | 0.811 | 0.000 | 0.001 | 0.962 |
| | 0.038 | 2448 | 144 | −0.002 | 0.002 | 0.051 | 0.000 | 0.001 | 0.914 | 0.000 | 0.001 | 0.966 |
| | 0.038 | 4896 | 36 | −0.006 | 0.006 | 0.000 | −0.002 | 0.002 | 0.124 | 0.000 | 0.001 | 0.934 |
| | 0.038 | 4896 | 72 | −0.003 | 0.003 | 0.000 | −0.001 | 0.001 | 0.664 | 0.000 | 0.001 | 0.957 |
| | 0.038 | 4896 | 144 | −0.002 | 0.002 | 0.001 | 0.000 | 0.001 | 0.880 | 0.000 | 0.001 | 0.960 |

Table S6: Monte Carlo simulation results for $\rho_1$ in design 1

| | true | $N$ | $T$ | **ED** | | | **HPJ** | | | **TOJ** | | |
|---|---|---|---|---|---|---|---|---|---|---|---|---|
| | | | | bias | rmse | cp | bias | rmse | cp | bias | rmse | cp |
| $\rho_1$ mean | 0.626 | 1224 | 36 | −0.088 | 0.088 | 0.000 | 0.006 | 0.009 | 0.868 | 0.006 | 0.013 | 0.920 |
| | 0.626 | 1224 | 72 | −0.042 | 0.043 | 0.000 | 0.003 | 0.006 | 0.915 | 0.001 | 0.007 | 0.945 |
| | 0.626 | 1224 | 144 | −0.021 | 0.021 | 0.007 | 0.001 | 0.005 | 0.947 | 0.000 | 0.005 | 0.953 |
| | 0.626 | 2448 | 36 | −0.088 | 0.088 | 0.000 | 0.006 | 0.008 | 0.787 | 0.006 | 0.010 | 0.892 |
| | 0.626 | 2448 | 72 | −0.042 | 0.042 | 0.000 | 0.003 | 0.005 | 0.883 | 0.001 | 0.005 | 0.948 |
| | 0.626 | 2448 | 144 | −0.021 | 0.021 | 0.000 | 0.001 | 0.004 | 0.943 | 0.000 | 0.004 | 0.946 |
| | 0.626 | 4896 | 36 | −0.088 | 0.088 | 0.000 | 0.006 | 0.007 | 0.619 | 0.006 | 0.008 | 0.818 |
| | 0.626 | 4896 | 72 | −0.042 | 0.042 | 0.000 | 0.003 | 0.004 | 0.819 | 0.001 | 0.004 | 0.945 |
| | 0.626 | 4896 | 144 | −0.021 | 0.021 | 0.000 | 0.001 | 0.003 | 0.928 | 0.000 | 0.003 | 0.948 |
| $\rho_1$ std | 0.154 | 1224 | 36 | 0.044 | 0.045 | 0.000 | −0.002 | 0.007 | 0.924 | −0.011 | 0.016 | 0.841 |
| | 0.154 | 1224 | 72 | 0.021 | 0.021 | 0.000 | −0.002 | 0.005 | 0.908 | −0.001 | 0.008 | 0.940 |
| | 0.154 | 1224 | 144 | 0.010 | 0.011 | 0.108 | −0.001 | 0.004 | 0.937 | 0.000 | 0.005 | 0.946 |
| | 0.154 | 2448 | 36 | 0.044 | 0.044 | 0.000 | −0.002 | 0.005 | 0.910 | −0.011 | 0.014 | 0.732 |
| | 0.154 | 2448 | 72 | 0.021 | 0.021 | 0.000 | −0.002 | 0.004 | 0.885 | −0.001 | 0.005 | 0.938 |
| | 0.154 | 2448 | 144 | 0.010 | 0.010 | 0.004 | −0.001 | 0.003 | 0.934 | 0.000 | 0.003 | 0.945 |
| | 0.154 | 4896 | 36 | 0.044 | 0.044 | 0.000 | −0.002 | 0.004 | 0.869 | −0.011 | 0.013 | 0.519 |
| | 0.154 | 4896 | 72 | 0.021 | 0.021 | 0.000 | −0.002 | 0.003 | 0.825 | −0.002 | 0.004 | 0.930 |
| | 0.154 | 4896 | 144 | 0.010 | 0.010 | 0.000 | −0.001 | 0.002 | 0.923 | 0.000 | 0.002 | 0.947 |
| $\rho_1$ 25%Q | 0.522 | 1224 | 36 | −0.111 | 0.112 | 0.000 | 0.011 | 0.017 | 0.881 | 0.012 | 0.031 | 0.949 |
| | 0.522 | 1224 | 72 | −0.053 | 0.054 | 0.000 | 0.005 | 0.012 | 0.928 | 0.001 | 0.020 | 0.971 |
| | 0.522 | 1224 | 144 | −0.026 | 0.027 | 0.031 | 0.002 | 0.009 | 0.952 | 0.000 | 0.016 | 0.972 |
| | 0.522 | 2448 | 36 | −0.112 | 0.112 | 0.000 | 0.011 | 0.014 | 0.811 | 0.012 | 0.023 | 0.927 |
| | 0.522 | 2448 | 72 | −0.053 | 0.054 | 0.000 | 0.005 | 0.009 | 0.898 | 0.001 | 0.015 | 0.961 |
| | 0.522 | 2448 | 144 | −0.026 | 0.026 | 0.001 | 0.002 | 0.007 | 0.949 | 0.000 | 0.011 | 0.965 |
| | 0.522 | 4896 | 36 | −0.112 | 0.112 | 0.000 | 0.011 | 0.013 | 0.656 | 0.012 | 0.018 | 0.881 |
| | 0.522 | 4896 | 72 | −0.053 | 0.053 | 0.000 | 0.005 | 0.007 | 0.846 | 0.001 | 0.010 | 0.960 |
| | 0.522 | 4896 | 144 | −0.026 | 0.026 | 0.000 | 0.002 | 0.005 | 0.932 | 0.000 | 0.008 | 0.958 |
| $\rho_1$ 50%Q | 0.628 | 1224 | 36 | −0.073 | 0.074 | 0.000 | 0.011 | 0.016 | 0.851 | 0.006 | 0.024 | 0.961 |
| | 0.628 | 1224 | 72 | −0.035 | 0.035 | 0.000 | 0.004 | 0.010 | 0.929 | 0.000 | 0.017 | 0.966 |
| | 0.628 | 1224 | 144 | −0.017 | 0.018 | 0.212 | 0.001 | 0.008 | 0.957 | −0.001 | 0.013 | 0.972 |
| | 0.628 | 2448 | 36 | −0.073 | 0.074 | 0.000 | 0.011 | 0.013 | 0.752 | 0.005 | 0.017 | 0.949 |
| | 0.628 | 2448 | 72 | −0.034 | 0.035 | 0.000 | 0.004 | 0.008 | 0.901 | 0.000 | 0.012 | 0.965 |
| | 0.628 | 2448 | 144 | −0.017 | 0.017 | 0.027 | 0.001 | 0.006 | 0.946 | 0.000 | 0.009 | 0.967 |
| | 0.628 | 4896 | 36 | −0.073 | 0.073 | 0.000 | 0.011 | 0.012 | 0.521 | 0.006 | 0.013 | 0.934 |
| | 0.628 | 4896 | 72 | −0.034 | 0.035 | 0.000 | 0.004 | 0.006 | 0.840 | 0.001 | 0.009 | 0.956 |
| | 0.628 | 4896 | 144 | −0.016 | 0.017 | 0.000 | 0.002 | 0.004 | 0.938 | 0.000 | 0.007 | 0.962 |
| $\rho_1$ 75%Q | 0.734 | 1224 | 36 | −0.049 | 0.050 | 0.000 | 0.006 | 0.013 | 0.924 | 0.001 | 0.023 | 0.963 |
| | 0.734 | 1224 | 72 | −0.023 | 0.024 | 0.048 | 0.003 | 0.010 | 0.943 | 0.001 | 0.017 | 0.963 |
| | 0.734 | 1224 | 144 | −0.011 | 0.013 | 0.560 | 0.001 | 0.008 | 0.960 | 0.000 | 0.013 | 0.979 |
| | 0.734 | 2448 | 36 | −0.049 | 0.049 | 0.000 | 0.007 | 0.010 | 0.874 | 0.001 | 0.016 | 0.962 |
| | 0.734 | 2448 | 72 | −0.023 | 0.024 | 0.001 | 0.003 | 0.007 | 0.935 | 0.001 | 0.012 | 0.965 |
| | 0.734 | 2448 | 144 | −0.011 | 0.012 | 0.269 | 0.001 | 0.006 | 0.950 | 0.000 | 0.010 | 0.967 |
| | 0.734 | 4896 | 36 | −0.049 | 0.049 | 0.000 | 0.007 | 0.009 | 0.787 | 0.001 | 0.011 | 0.958 |
| | 0.734 | 4896 | 72 | −0.023 | 0.023 | 0.000 | 0.003 | 0.005 | 0.915 | 0.001 | 0.008 | 0.962 |
| | 0.734 | 4896 | 144 | −0.011 | 0.011 | 0.058 | 0.001 | 0.004 | 0.943 | 0.000 | 0.007 | 0.964 |

Table S7: Monte Carlo simulation results for correlations in design 1

| | true | $N$ | $T$ | ED bias | ED rmse | ED cp | HPJ bias | HPJ rmse | HPJ cp | TOJ bias | TOJ rmse | TOJ cp |
|---|---|---|---|---|---|---|---|---|---|---|---|---|
| $\mu$ vs $\gamma_0$ | 0.070 | 1224 | 36 | −0.002 | 0.029 | 0.947 | 0.001 | 0.039 | 0.947 | 0.001 | 0.056 | 0.949 |
| | 0.070 | 1224 | 72 | 0.000 | 0.029 | 0.946 | 0.002 | 0.035 | 0.946 | 0.002 | 0.045 | 0.945 |
| | 0.070 | 1224 | 144 | 0.001 | 0.029 | 0.947 | 0.001 | 0.033 | 0.945 | 0.001 | 0.038 | 0.944 |
| | 0.070 | 2448 | 36 | −0.001 | 0.021 | 0.948 | 0.002 | 0.027 | 0.946 | 0.003 | 0.039 | 0.944 |
| | 0.070 | 2448 | 72 | 0.000 | 0.021 | 0.947 | 0.001 | 0.025 | 0.947 | 0.001 | 0.032 | 0.947 |
| | 0.070 | 2448 | 144 | 0.001 | 0.020 | 0.950 | 0.001 | 0.023 | 0.949 | 0.001 | 0.027 | 0.948 |
| | 0.070 | 4896 | 36 | −0.001 | 0.015 | 0.948 | 0.002 | 0.019 | 0.943 | 0.002 | 0.028 | 0.945 |
| | 0.070 | 4896 | 72 | 0.000 | 0.015 | 0.950 | 0.001 | 0.018 | 0.948 | 0.001 | 0.023 | 0.950 |
| | 0.070 | 4896 | 144 | 0.000 | 0.015 | 0.947 | 0.001 | 0.016 | 0.945 | 0.001 | 0.019 | 0.947 |
| $\mu$ vs $\rho_1$ | −0.158 | 1224 | 36 | 0.063 | 0.069 | 0.404 | 0.028 | 0.049 | 0.891 | 0.003 | 0.063 | 0.947 |
| | −0.158 | 1224 | 72 | 0.036 | 0.046 | 0.754 | 0.009 | 0.038 | 0.939 | −0.003 | 0.048 | 0.944 |
| | −0.158 | 1224 | 144 | 0.019 | 0.034 | 0.897 | 0.002 | 0.033 | 0.943 | −0.001 | 0.037 | 0.943 |
| | −0.158 | 2448 | 36 | 0.063 | 0.066 | 0.120 | 0.028 | 0.040 | 0.831 | 0.005 | 0.045 | 0.946 |
| | −0.158 | 2448 | 72 | 0.036 | 0.042 | 0.565 | 0.010 | 0.027 | 0.930 | −0.001 | 0.034 | 0.946 |
| | −0.158 | 2448 | 144 | 0.019 | 0.028 | 0.834 | 0.003 | 0.023 | 0.942 | −0.001 | 0.026 | 0.948 |
| | −0.158 | 4896 | 36 | 0.063 | 0.065 | 0.007 | 0.029 | 0.035 | 0.702 | 0.005 | 0.033 | 0.941 |
| | −0.158 | 4896 | 72 | 0.036 | 0.039 | 0.295 | 0.009 | 0.020 | 0.924 | −0.002 | 0.024 | 0.950 |
| | −0.158 | 4896 | 144 | 0.019 | 0.024 | 0.730 | 0.002 | 0.016 | 0.946 | −0.001 | 0.019 | 0.947 |
| $\gamma_0$ vs $\rho_1$ | 0.086 | 1224 | 36 | 0.104 | 0.108 | 0.036 | 0.049 | 0.063 | 0.762 | −0.007 | 0.061 | 0.942 |
| | 0.086 | 1224 | 72 | 0.052 | 0.059 | 0.548 | 0.000 | 0.037 | 0.945 | −0.026 | 0.057 | 0.916 |
| | 0.086 | 1224 | 144 | 0.022 | 0.036 | 0.882 | −0.009 | 0.035 | 0.943 | −0.013 | 0.043 | 0.934 |
| | 0.086 | 2448 | 36 | 0.104 | 0.106 | 0.001 | 0.049 | 0.056 | 0.580 | −0.008 | 0.044 | 0.946 |
| | 0.086 | 2448 | 72 | 0.053 | 0.056 | 0.261 | 0.002 | 0.026 | 0.951 | −0.024 | 0.044 | 0.888 |
| | 0.086 | 2448 | 144 | 0.022 | 0.030 | 0.809 | −0.009 | 0.026 | 0.936 | −0.013 | 0.033 | 0.924 |
| | 0.086 | 4896 | 36 | 0.104 | 0.105 | 0.000 | 0.049 | 0.052 | 0.310 | −0.009 | 0.031 | 0.938 |
| | 0.086 | 4896 | 72 | 0.053 | 0.055 | 0.041 | 0.001 | 0.019 | 0.946 | −0.025 | 0.036 | 0.824 |
| | 0.086 | 4896 | 144 | 0.022 | 0.026 | 0.667 | −0.009 | 0.019 | 0.914 | −0.013 | 0.025 | 0.890 |

Table S8: Monte Carlo simulation results for $\mu$ in design 2

| | true | $N$ | $T$ | ED | | | HPJ | | | TOJ | | |
|---|---|---|---|---|---|---|---|---|---|---|---|---|
| | | | | bias | rmse | cp | bias | rmse | cp | bias | rmse | cp |
| $\mu$ mean | −0.023 | 196 | 6 | 0.000 | 0.030 | 0.945 | 0.000 | 0.030 | 0.946 | 0.000 | 0.030 | 0.947 |
| | −0.023 | 196 | 12 | 0.000 | 0.029 | 0.942 | 0.000 | 0.029 | 0.942 | 0.000 | 0.029 | 0.943 |
| | −0.023 | 196 | 24 | 0.000 | 0.027 | 0.946 | 0.000 | 0.027 | 0.946 | 0.000 | 0.027 | 0.946 |
| | −0.023 | 393 | 6 | 0.000 | 0.021 | 0.946 | 0.000 | 0.021 | 0.944 | 0.000 | 0.021 | 0.944 |
| | −0.023 | 393 | 12 | 0.000 | 0.019 | 0.952 | 0.000 | 0.019 | 0.953 | 0.000 | 0.019 | 0.951 |
| | −0.023 | 393 | 24 | 0.000 | 0.019 | 0.946 | 0.000 | 0.019 | 0.947 | 0.000 | 0.019 | 0.946 |
| | −0.023 | 786 | 6 | 0.000 | 0.015 | 0.946 | 0.000 | 0.015 | 0.948 | 0.000 | 0.015 | 0.946 |
| | −0.023 | 786 | 12 | 0.000 | 0.014 | 0.950 | 0.000 | 0.014 | 0.948 | 0.000 | 0.014 | 0.948 |
| | −0.023 | 786 | 24 | 0.000 | 0.013 | 0.942 | 0.000 | 0.013 | 0.943 | 0.000 | 0.013 | 0.945 |
| $\mu$ std | 0.346 | 196 | 6 | 0.069 | 0.072 | 0.099 | 0.041 | 0.047 | 0.591 | 0.025 | 0.036 | 0.850 |
| | 0.346 | 196 | 12 | 0.045 | 0.049 | 0.388 | 0.022 | 0.030 | 0.854 | 0.009 | 0.025 | 0.936 |
| | 0.346 | 196 | 24 | 0.027 | 0.034 | 0.732 | 0.009 | 0.023 | 0.928 | 0.002 | 0.022 | 0.939 |
| | 0.346 | 393 | 6 | 0.069 | 0.071 | 0.004 | 0.042 | 0.045 | 0.284 | 0.026 | 0.032 | 0.725 |
| | 0.346 | 393 | 12 | 0.045 | 0.048 | 0.107 | 0.022 | 0.027 | 0.733 | 0.010 | 0.020 | 0.915 |
| | 0.346 | 393 | 24 | 0.028 | 0.031 | 0.472 | 0.010 | 0.017 | 0.904 | 0.003 | 0.015 | 0.947 |
| | 0.346 | 786 | 6 | 0.069 | 0.070 | 0.000 | 0.042 | 0.043 | 0.050 | 0.025 | 0.029 | 0.518 |
| | 0.346 | 786 | 12 | 0.045 | 0.047 | 0.004 | 0.022 | 0.024 | 0.480 | 0.010 | 0.016 | 0.879 |
| | 0.346 | 786 | 24 | 0.028 | 0.029 | 0.162 | 0.010 | 0.014 | 0.839 | 0.003 | 0.011 | 0.946 |
| $\mu$ 25%Q | −0.256 | 196 | 6 | −0.038 | 0.055 | 0.846 | −0.023 | 0.055 | 0.947 | −0.014 | 0.080 | 0.990 |
| | −0.256 | 196 | 12 | −0.025 | 0.046 | 0.899 | −0.012 | 0.049 | 0.959 | −0.004 | 0.074 | 0.991 |
| | −0.256 | 196 | 24 | −0.015 | 0.039 | 0.935 | −0.004 | 0.044 | 0.968 | 0.000 | 0.067 | 0.994 |
| | −0.256 | 393 | 6 | −0.039 | 0.048 | 0.718 | −0.025 | 0.043 | 0.914 | −0.016 | 0.059 | 0.985 |
| | −0.256 | 393 | 12 | −0.026 | 0.038 | 0.839 | −0.013 | 0.036 | 0.948 | −0.006 | 0.054 | 0.989 |
| | −0.256 | 393 | 24 | −0.016 | 0.030 | 0.906 | −0.006 | 0.032 | 0.959 | −0.002 | 0.048 | 0.989 |
| | −0.256 | 786 | 6 | −0.039 | 0.044 | 0.494 | −0.024 | 0.035 | 0.853 | −0.015 | 0.043 | 0.973 |
| | −0.256 | 786 | 12 | −0.026 | 0.032 | 0.723 | −0.013 | 0.027 | 0.933 | −0.006 | 0.037 | 0.983 |
| | −0.256 | 786 | 24 | −0.016 | 0.024 | 0.852 | −0.006 | 0.023 | 0.953 | −0.003 | 0.034 | 0.982 |
| $\mu$ 50%Q | −0.022 | 196 | 6 | 0.003 | 0.037 | 0.942 | 0.001 | 0.045 | 0.960 | 0.000 | 0.069 | 0.988 |
| | −0.022 | 196 | 12 | 0.002 | 0.035 | 0.947 | 0.000 | 0.042 | 0.961 | 0.000 | 0.065 | 0.990 |
| | −0.022 | 196 | 24 | 0.001 | 0.034 | 0.943 | 0.000 | 0.040 | 0.962 | −0.001 | 0.060 | 0.992 |
| | −0.022 | 393 | 6 | 0.002 | 0.026 | 0.946 | 0.001 | 0.032 | 0.962 | 0.000 | 0.049 | 0.988 |
| | −0.022 | 393 | 12 | 0.002 | 0.024 | 0.950 | 0.000 | 0.029 | 0.963 | 0.000 | 0.046 | 0.988 |
| | −0.022 | 393 | 24 | 0.000 | 0.024 | 0.950 | −0.001 | 0.028 | 0.960 | −0.001 | 0.042 | 0.986 |
| | −0.022 | 786 | 6 | 0.003 | 0.019 | 0.944 | 0.001 | 0.023 | 0.958 | 0.000 | 0.035 | 0.980 |
| | −0.022 | 786 | 12 | 0.002 | 0.017 | 0.947 | 0.000 | 0.021 | 0.958 | 0.000 | 0.033 | 0.980 |
| | −0.022 | 786 | 24 | 0.001 | 0.017 | 0.938 | 0.000 | 0.020 | 0.952 | 0.000 | 0.030 | 0.978 |
| $\mu$ 75%Q | 0.211 | 196 | 6 | 0.041 | 0.057 | 0.825 | 0.023 | 0.054 | 0.944 | 0.013 | 0.077 | 0.993 |
| | 0.211 | 196 | 12 | 0.026 | 0.046 | 0.890 | 0.012 | 0.048 | 0.959 | 0.004 | 0.071 | 0.995 |
| | 0.211 | 196 | 24 | 0.015 | 0.040 | 0.922 | 0.004 | 0.044 | 0.960 | 0.000 | 0.065 | 0.993 |
| | 0.211 | 393 | 6 | 0.043 | 0.051 | 0.670 | 0.026 | 0.043 | 0.909 | 0.016 | 0.056 | 0.984 |
| | 0.211 | 393 | 12 | 0.027 | 0.038 | 0.827 | 0.013 | 0.035 | 0.955 | 0.005 | 0.051 | 0.993 |
| | 0.211 | 393 | 24 | 0.016 | 0.030 | 0.905 | 0.005 | 0.032 | 0.959 | 0.001 | 0.048 | 0.988 |
| | 0.211 | 786 | 6 | 0.042 | 0.047 | 0.423 | 0.025 | 0.035 | 0.840 | 0.015 | 0.042 | 0.971 |
| | 0.211 | 786 | 12 | 0.028 | 0.034 | 0.673 | 0.013 | 0.027 | 0.925 | 0.006 | 0.037 | 0.977 |
| | 0.211 | 786 | 24 | 0.017 | 0.025 | 0.845 | 0.006 | 0.023 | 0.952 | 0.001 | 0.033 | 0.984 |

Table S9: Monte Carlo simulation results for $\gamma_0$ in design 2

| | true | $N$ | $T$ | **ED** bias | **ED** rmse | **ED** cp | **HPJ** bias | **HPJ** rmse | **HPJ** cp | **TOJ** bias | **TOJ** rmse | **TOJ** cp |
|---|---|---|---|---|---|---|---|---|---|---|---|---|
| $\gamma_0$ mean | 0.121 | 196 | 6 | −0.053 | 0.053 | 0.000 | −0.029 | 0.030 | 0.147 | −0.016 | 0.021 | 0.695 |
| | 0.121 | 196 | 12 | −0.034 | 0.034 | 0.004 | −0.015 | 0.017 | 0.538 | −0.006 | 0.013 | 0.879 |
| | 0.121 | 196 | 24 | −0.020 | 0.021 | 0.154 | −0.007 | 0.010 | 0.827 | −0.002 | 0.010 | 0.924 |
| | 0.121 | 393 | 6 | −0.053 | 0.053 | 0.000 | −0.029 | 0.030 | 0.013 | −0.017 | 0.019 | 0.539 |
| | 0.121 | 393 | 12 | −0.034 | 0.034 | 0.000 | −0.015 | 0.016 | 0.321 | −0.006 | 0.010 | 0.854 |
| | 0.121 | 393 | 24 | −0.020 | 0.021 | 0.014 | −0.006 | 0.008 | 0.753 | −0.002 | 0.007 | 0.927 |
| | 0.121 | 786 | 6 | −0.053 | 0.053 | 0.000 | −0.029 | 0.029 | 0.000 | −0.016 | 0.018 | 0.313 |
| | 0.121 | 786 | 12 | −0.034 | 0.034 | 0.000 | −0.015 | 0.015 | 0.082 | −0.006 | 0.008 | 0.790 |
| | 0.121 | 786 | 24 | −0.020 | 0.020 | 0.000 | −0.006 | 0.007 | 0.596 | −0.002 | 0.005 | 0.922 |
| $\gamma_0$ std | 0.085 | 196 | 6 | −0.002 | 0.012 | 0.833 | 0.009 | 0.020 | 0.917 | 0.010 | 0.036 | 0.920 |
| | 0.085 | 196 | 12 | 0.002 | 0.010 | 0.916 | 0.007 | 0.015 | 0.918 | 0.007 | 0.025 | 0.919 |
| | 0.085 | 196 | 24 | 0.004 | 0.009 | 0.924 | 0.005 | 0.012 | 0.920 | 0.003 | 0.018 | 0.907 |
| | 0.085 | 393 | 6 | −0.002 | 0.009 | 0.847 | 0.008 | 0.015 | 0.911 | 0.009 | 0.026 | 0.921 |
| | 0.085 | 393 | 12 | 0.003 | 0.008 | 0.929 | 0.008 | 0.013 | 0.893 | 0.007 | 0.019 | 0.928 |
| | 0.085 | 393 | 24 | 0.004 | 0.007 | 0.909 | 0.005 | 0.009 | 0.909 | 0.003 | 0.013 | 0.929 |
| | 0.085 | 786 | 6 | −0.002 | 0.006 | 0.871 | 0.008 | 0.012 | 0.864 | 0.009 | 0.020 | 0.918 |
| | 0.085 | 786 | 12 | 0.003 | 0.006 | 0.922 | 0.008 | 0.011 | 0.809 | 0.007 | 0.015 | 0.909 |
| | 0.085 | 786 | 24 | 0.004 | 0.006 | 0.861 | 0.005 | 0.007 | 0.865 | 0.003 | 0.009 | 0.931 |
| $\gamma_0$ 25%Q | 0.053 | 196 | 6 | −0.038 | 0.038 | 0.000 | −0.028 | 0.028 | 0.001 | −0.019 | 0.020 | 0.326 |
| | 0.053 | 196 | 12 | −0.027 | 0.027 | 0.000 | −0.016 | 0.017 | 0.284 | −0.009 | 0.013 | 0.867 |
| | 0.053 | 196 | 24 | −0.017 | 0.018 | 0.085 | −0.008 | 0.010 | 0.808 | −0.003 | 0.010 | 0.972 |
| | 0.053 | 393 | 6 | −0.038 | 0.038 | 0.000 | −0.028 | 0.028 | 0.000 | −0.019 | 0.019 | 0.066 |
| | 0.053 | 393 | 12 | −0.027 | 0.027 | 0.000 | −0.016 | 0.017 | 0.052 | −0.009 | 0.011 | 0.729 |
| | 0.053 | 393 | 24 | −0.018 | 0.018 | 0.002 | −0.008 | 0.010 | 0.637 | −0.003 | 0.008 | 0.958 |
| | 0.053 | 786 | 6 | −0.038 | 0.038 | 0.000 | −0.028 | 0.028 | 0.000 | −0.019 | 0.019 | 0.001 |
| | 0.053 | 786 | 12 | −0.027 | 0.027 | 0.000 | −0.017 | 0.017 | 0.001 | −0.009 | 0.010 | 0.486 |
| | 0.053 | 786 | 24 | −0.018 | 0.018 | 0.000 | −0.008 | 0.009 | 0.351 | −0.003 | 0.006 | 0.926 |
| $\gamma_0$ 50%Q | 0.107 | 196 | 6 | −0.066 | 0.066 | 0.000 | −0.044 | 0.045 | 0.005 | −0.028 | 0.031 | 0.481 |
| | 0.107 | 196 | 12 | −0.046 | 0.046 | 0.000 | −0.025 | 0.027 | 0.310 | −0.013 | 0.020 | 0.888 |
| | 0.107 | 196 | 24 | −0.029 | 0.030 | 0.036 | −0.012 | 0.016 | 0.777 | −0.004 | 0.016 | 0.969 |
| | 0.107 | 393 | 6 | −0.066 | 0.066 | 0.000 | −0.045 | 0.045 | 0.000 | −0.029 | 0.030 | 0.180 |
| | 0.107 | 393 | 12 | −0.046 | 0.046 | 0.000 | −0.025 | 0.026 | 0.067 | −0.013 | 0.017 | 0.801 |
| | 0.107 | 393 | 24 | −0.029 | 0.029 | 0.000 | −0.012 | 0.014 | 0.626 | −0.004 | 0.012 | 0.957 |
| | 0.107 | 786 | 6 | −0.066 | 0.066 | 0.000 | −0.045 | 0.045 | 0.000 | −0.029 | 0.029 | 0.019 |
| | 0.107 | 786 | 12 | −0.046 | 0.046 | 0.000 | −0.025 | 0.025 | 0.001 | −0.013 | 0.015 | 0.627 |
| | 0.107 | 786 | 24 | −0.029 | 0.029 | 0.000 | −0.012 | 0.013 | 0.362 | −0.004 | 0.009 | 0.939 |
| $\gamma_0$ 75%Q | 0.174 | 196 | 6 | −0.083 | 0.084 | 0.000 | −0.047 | 0.049 | 0.239 | −0.026 | 0.037 | 0.853 |
| | 0.174 | 196 | 12 | −0.054 | 0.055 | 0.009 | −0.024 | 0.029 | 0.693 | −0.010 | 0.029 | 0.962 |
| | 0.174 | 196 | 24 | −0.032 | 0.034 | 0.198 | −0.011 | 0.019 | 0.880 | −0.004 | 0.026 | 0.978 |
| | 0.174 | 393 | 6 | −0.084 | 0.084 | 0.000 | −0.047 | 0.048 | 0.042 | −0.027 | 0.033 | 0.734 |
| | 0.174 | 393 | 12 | −0.054 | 0.054 | 0.000 | −0.024 | 0.026 | 0.492 | −0.010 | 0.021 | 0.943 |
| | 0.174 | 393 | 24 | −0.032 | 0.033 | 0.028 | −0.011 | 0.015 | 0.833 | −0.004 | 0.019 | 0.973 |
| | 0.174 | 786 | 6 | −0.084 | 0.084 | 0.000 | −0.047 | 0.047 | 0.001 | −0.027 | 0.030 | 0.518 |
| | 0.174 | 786 | 12 | −0.054 | 0.054 | 0.000 | −0.024 | 0.025 | 0.192 | −0.010 | 0.017 | 0.911 |
| | 0.174 | 786 | 24 | −0.032 | 0.033 | 0.000 | −0.011 | 0.013 | 0.726 | −0.003 | 0.013 | 0.965 |

Table S10: Monte Carlo simulation results for $\rho_1$ in design 2

| | true | $N$ | $T$ | **ED** bias | **ED** rmse | **ED** cp | **HPJ** bias | **HPJ** rmse | **HPJ** cp | **TOJ** bias | **TOJ** rmse | **TOJ** cp |
|---|---|---|---|---|---|---|---|---|---|---|---|---|
| $\rho_1$ mean | 0.515 | 196 | 6 | −0.477 | 0.477 | 0.000 | −0.011 | 0.051 | 0.940 | −0.176 | 0.200 | 0.540 |
| | 0.515 | 196 | 12 | −0.239 | 0.240 | 0.000 | −0.002 | 0.034 | 0.946 | 0.009 | 0.066 | 0.948 |
| | 0.515 | 196 | 24 | −0.117 | 0.119 | 0.000 | 0.005 | 0.025 | 0.945 | 0.009 | 0.042 | 0.939 |
| | 0.515 | 393 | 6 | −0.476 | 0.477 | 0.000 | −0.012 | 0.037 | 0.933 | −0.179 | 0.191 | 0.244 |
| | 0.515 | 393 | 12 | −0.240 | 0.240 | 0.000 | −0.003 | 0.025 | 0.943 | 0.009 | 0.047 | 0.942 |
| | 0.515 | 393 | 24 | −0.117 | 0.118 | 0.000 | 0.005 | 0.018 | 0.935 | 0.009 | 0.030 | 0.937 |
| | 0.515 | 786 | 6 | −0.476 | 0.477 | 0.000 | −0.011 | 0.027 | 0.928 | −0.177 | 0.184 | 0.039 |
| | 0.515 | 786 | 12 | −0.240 | 0.240 | 0.000 | −0.002 | 0.017 | 0.945 | 0.010 | 0.034 | 0.935 |
| | 0.515 | 786 | 24 | −0.117 | 0.118 | 0.000 | 0.005 | 0.013 | 0.933 | 0.008 | 0.022 | 0.932 |
| $\rho_1$ std | 0.229 | 196 | 6 | 0.142 | 0.143 | 0.000 | 0.162 | 0.165 | 0.000 | −0.345 | 0.349 | 0.000 |
| | 0.229 | 196 | 12 | 0.082 | 0.083 | 0.000 | 0.022 | 0.035 | 0.879 | −0.048 | 0.073 | 0.836 |
| | 0.229 | 196 | 24 | 0.038 | 0.040 | 0.147 | −0.005 | 0.021 | 0.924 | −0.017 | 0.041 | 0.915 |
| | 0.229 | 393 | 6 | 0.142 | 0.143 | 0.000 | 0.163 | 0.164 | 0.000 | −0.343 | 0.346 | 0.000 |
| | 0.229 | 393 | 12 | 0.082 | 0.083 | 0.000 | 0.022 | 0.029 | 0.788 | −0.049 | 0.063 | 0.733 |
| | 0.229 | 393 | 24 | 0.038 | 0.039 | 0.008 | −0.006 | 0.015 | 0.919 | −0.018 | 0.032 | 0.892 |
| | 0.229 | 786 | 6 | 0.142 | 0.142 | 0.000 | 0.163 | 0.164 | 0.000 | −0.343 | 0.344 | 0.000 |
| | 0.229 | 786 | 12 | 0.082 | 0.082 | 0.000 | 0.022 | 0.025 | 0.624 | −0.050 | 0.056 | 0.532 |
| | 0.229 | 786 | 24 | 0.038 | 0.039 | 0.000 | −0.005 | 0.011 | 0.906 | −0.017 | 0.025 | 0.832 |
| $\rho_1$ 25%Q | 0.361 | 196 | 6 | −0.586 | 0.587 | 0.000 | −0.050 | 0.095 | 0.918 | 0.404 | 0.440 | 0.410 |
| | 0.361 | 196 | 12 | −0.293 | 0.295 | 0.000 | −0.002 | 0.060 | 0.966 | 0.103 | 0.164 | 0.920 |
| | 0.361 | 196 | 24 | −0.139 | 0.142 | 0.002 | 0.016 | 0.048 | 0.955 | 0.023 | 0.095 | 0.977 |
| | 0.361 | 393 | 6 | −0.586 | 0.587 | 0.000 | −0.051 | 0.077 | 0.862 | 0.406 | 0.425 | 0.101 |
| | 0.361 | 393 | 12 | −0.294 | 0.295 | 0.000 | −0.001 | 0.043 | 0.960 | 0.110 | 0.143 | 0.822 |
| | 0.361 | 393 | 24 | −0.139 | 0.141 | 0.000 | 0.015 | 0.036 | 0.938 | 0.021 | 0.069 | 0.967 |
| | 0.361 | 786 | 6 | −0.588 | 0.588 | 0.000 | −0.051 | 0.065 | 0.759 | 0.408 | 0.417 | 0.003 |
| | 0.361 | 786 | 12 | −0.295 | 0.295 | 0.000 | −0.001 | 0.031 | 0.949 | 0.110 | 0.128 | 0.637 |
| | 0.361 | 786 | 24 | −0.140 | 0.141 | 0.000 | 0.014 | 0.027 | 0.909 | 0.021 | 0.051 | 0.947 |
| $\rho_1$ 50%Q | 0.523 | 196 | 6 | −0.452 | 0.453 | 0.000 | −0.023 | 0.078 | 0.946 | −0.352 | 0.391 | 0.503 |
| | 0.523 | 196 | 12 | −0.221 | 0.223 | 0.000 | 0.010 | 0.054 | 0.959 | −0.020 | 0.116 | 0.966 |
| | 0.523 | 196 | 24 | −0.104 | 0.107 | 0.011 | 0.014 | 0.042 | 0.949 | 0.013 | 0.081 | 0.975 |
| | 0.523 | 393 | 6 | −0.451 | 0.452 | 0.000 | −0.024 | 0.058 | 0.935 | −0.357 | 0.377 | 0.184 |
| | 0.523 | 393 | 12 | −0.221 | 0.222 | 0.000 | 0.010 | 0.039 | 0.953 | −0.019 | 0.084 | 0.963 |
| | 0.523 | 393 | 24 | −0.103 | 0.105 | 0.000 | 0.014 | 0.031 | 0.930 | 0.012 | 0.058 | 0.967 |
| | 0.523 | 786 | 6 | −0.451 | 0.452 | 0.000 | −0.024 | 0.045 | 0.910 | −0.357 | 0.367 | 0.015 |
| | 0.523 | 786 | 12 | −0.221 | 0.222 | 0.000 | 0.010 | 0.028 | 0.936 | −0.020 | 0.061 | 0.948 |
| | 0.523 | 786 | 24 | −0.104 | 0.104 | 0.000 | 0.013 | 0.024 | 0.910 | 0.011 | 0.041 | 0.960 |
| $\rho_1$ 75%Q | 0.682 | 196 | 6 | −0.357 | 0.358 | 0.000 | 0.057 | 0.087 | 0.867 | −0.707 | 0.718 | 0.000 |
| | 0.682 | 196 | 12 | −0.170 | 0.172 | 0.000 | 0.018 | 0.053 | 0.953 | 0.016 | 0.110 | 0.971 |
| | 0.682 | 196 | 24 | −0.084 | 0.087 | 0.052 | 0.003 | 0.039 | 0.964 | 0.000 | 0.078 | 0.976 |
| | 0.682 | 393 | 6 | −0.356 | 0.357 | 0.000 | 0.056 | 0.073 | 0.773 | −0.713 | 0.718 | 0.000 |
| | 0.682 | 393 | 12 | −0.170 | 0.171 | 0.000 | 0.016 | 0.040 | 0.933 | 0.014 | 0.079 | 0.962 |
| | 0.682 | 393 | 24 | −0.083 | 0.085 | 0.002 | 0.003 | 0.028 | 0.955 | 0.000 | 0.056 | 0.971 |
| | 0.682 | 786 | 6 | −0.355 | 0.356 | 0.000 | 0.057 | 0.066 | 0.577 | −0.712 | 0.715 | 0.000 |
| | 0.682 | 786 | 12 | −0.169 | 0.170 | 0.000 | 0.017 | 0.030 | 0.909 | 0.017 | 0.057 | 0.959 |
| | 0.682 | 786 | 24 | −0.083 | 0.084 | 0.000 | 0.003 | 0.020 | 0.952 | 0.000 | 0.040 | 0.965 |

Table S11: Monte Carlo simulation results for correlations in design 2

| | true | $N$ | $T$ | ED bias | ED rmse | ED cp | HPJ bias | HPJ rmse | HPJ cp | TOJ bias | TOJ rmse | TOJ cp |
|---|---|---|---|---|---|---|---|---|---|---|---|---|
| $\mu$ vs $\gamma_0$ | −0.149 | 196 | 6 | 0.054 | 0.092 | 0.874 | 0.031 | 0.114 | 0.926 | 0.022 | 0.184 | 0.939 |
| | −0.149 | 196 | 12 | 0.038 | 0.083 | 0.910 | 0.020 | 0.102 | 0.937 | 0.012 | 0.151 | 0.942 |
| | −0.149 | 196 | 24 | 0.025 | 0.077 | 0.930 | 0.012 | 0.092 | 0.939 | 0.008 | 0.125 | 0.940 |
| | −0.149 | 393 | 6 | 0.057 | 0.078 | 0.795 | 0.035 | 0.085 | 0.920 | 0.025 | 0.131 | 0.939 |
| | −0.149 | 393 | 12 | 0.038 | 0.065 | 0.875 | 0.021 | 0.074 | 0.931 | 0.015 | 0.107 | 0.939 |
| | −0.149 | 393 | 24 | 0.026 | 0.058 | 0.914 | 0.013 | 0.065 | 0.942 | 0.007 | 0.088 | 0.942 |
| | −0.149 | 786 | 6 | 0.055 | 0.067 | 0.673 | 0.032 | 0.064 | 0.898 | 0.023 | 0.094 | 0.934 |
| | −0.149 | 786 | 12 | 0.038 | 0.053 | 0.817 | 0.020 | 0.054 | 0.926 | 0.013 | 0.077 | 0.941 |
| | −0.149 | 786 | 24 | 0.025 | 0.044 | 0.891 | 0.011 | 0.047 | 0.936 | 0.006 | 0.063 | 0.941 |
| $\mu$ vs $\rho_1$ | 0.106 | 196 | 6 | −0.084 | 0.111 | 0.775 | −0.069 | 0.153 | 0.912 | −0.056 | 0.285 | 0.938 |
| | 0.106 | 196 | 12 | −0.060 | 0.092 | 0.860 | −0.037 | 0.120 | 0.930 | −0.017 | 0.206 | 0.942 |
| | 0.106 | 196 | 24 | −0.036 | 0.080 | 0.916 | −0.011 | 0.102 | 0.945 | 0.004 | 0.158 | 0.940 |
| | 0.106 | 393 | 6 | −0.083 | 0.097 | 0.611 | −0.068 | 0.117 | 0.884 | −0.054 | 0.203 | 0.933 |
| | 0.106 | 393 | 12 | −0.060 | 0.078 | 0.773 | −0.036 | 0.090 | 0.918 | −0.016 | 0.148 | 0.942 |
| | 0.106 | 393 | 24 | −0.037 | 0.062 | 0.882 | −0.014 | 0.072 | 0.945 | 0.000 | 0.110 | 0.948 |
| | 0.106 | 786 | 6 | −0.083 | 0.090 | 0.347 | −0.068 | 0.095 | 0.829 | −0.054 | 0.147 | 0.929 |
| | 0.106 | 786 | 12 | −0.060 | 0.070 | 0.606 | −0.037 | 0.069 | 0.898 | −0.017 | 0.105 | 0.941 |
| | 0.106 | 786 | 24 | −0.035 | 0.050 | 0.832 | −0.010 | 0.051 | 0.942 | 0.005 | 0.079 | 0.949 |
| $\gamma_0$ vs $\rho_1$ | −0.048 | 196 | 6 | 0.168 | 0.182 | 0.341 | 0.208 | 0.246 | 0.617 | 0.156 | 0.299 | 0.891 |
| | −0.048 | 196 | 12 | 0.138 | 0.155 | 0.523 | 0.109 | 0.158 | 0.840 | 0.042 | 0.204 | 0.938 |
| | −0.048 | 196 | 24 | 0.078 | 0.107 | 0.818 | 0.018 | 0.108 | 0.941 | −0.037 | 0.171 | 0.934 |
| | −0.048 | 393 | 6 | 0.167 | 0.174 | 0.105 | 0.206 | 0.225 | 0.369 | 0.157 | 0.237 | 0.843 |
| | −0.048 | 393 | 12 | 0.139 | 0.148 | 0.242 | 0.111 | 0.138 | 0.722 | 0.045 | 0.150 | 0.932 |
| | −0.048 | 393 | 24 | 0.078 | 0.094 | 0.681 | 0.017 | 0.078 | 0.937 | −0.039 | 0.125 | 0.921 |
| | −0.048 | 786 | 6 | 0.168 | 0.171 | 0.006 | 0.209 | 0.219 | 0.108 | 0.164 | 0.206 | 0.731 |
| | −0.048 | 786 | 12 | 0.139 | 0.143 | 0.041 | 0.110 | 0.125 | 0.522 | 0.043 | 0.109 | 0.931 |
| | −0.048 | 786 | 24 | 0.078 | 0.086 | 0.457 | 0.018 | 0.056 | 0.940 | −0.038 | 0.091 | 0.915 |

Table S12: Monte Carlo simulation results for $\mu$ in design 3

| | true | $N$ | $T$ | **ED** bias | **ED** rmse | **ED** cp | **HPJ** bias | **HPJ** rmse | **HPJ** cp | **TOJ** bias | **TOJ** rmse | **TOJ** cp |
|---|---|---|---|---|---|---|---|---|---|---|---|---|
| $\mu$ mean | 2.976 | 232 | 10 | 0.000 | 0.020 | 0.949 | 0.000 | 0.020 | 0.950 | 0.000 | 0.020 | 0.951 |
| | 2.976 | 232 | 18 | 0.000 | 0.019 | 0.947 | 0.000 | 0.019 | 0.946 | 0.000 | 0.019 | 0.949 |
| | 2.976 | 232 | 36 | 0.000 | 0.019 | 0.949 | 0.000 | 0.019 | 0.947 | 0.000 | 0.019 | 0.946 |
| | 2.976 | 465 | 10 | 0.000 | 0.014 | 0.946 | 0.000 | 0.014 | 0.946 | 0.000 | 0.015 | 0.947 |
| | 2.976 | 465 | 18 | 0.000 | 0.014 | 0.950 | 0.000 | 0.014 | 0.948 | 0.000 | 0.014 | 0.947 |
| | 2.976 | 465 | 36 | 0.000 | 0.013 | 0.949 | 0.000 | 0.013 | 0.947 | 0.000 | 0.013 | 0.950 |
| | 2.976 | 930 | 10 | 0.000 | 0.010 | 0.952 | 0.000 | 0.010 | 0.954 | 0.000 | 0.010 | 0.951 |
| | 2.976 | 930 | 18 | 0.000 | 0.010 | 0.954 | 0.000 | 0.010 | 0.955 | 0.000 | 0.010 | 0.953 |
| | 2.976 | 930 | 36 | 0.000 | 0.009 | 0.946 | 0.000 | 0.009 | 0.948 | 0.000 | 0.009 | 0.946 |
| $\mu$ std | 0.281 | 232 | 10 | 0.027 | 0.030 | 0.564 | 0.013 | 0.020 | 0.874 | 0.009 | 0.019 | 0.917 |
| | 0.281 | 232 | 18 | 0.018 | 0.023 | 0.782 | 0.007 | 0.016 | 0.934 | 0.002 | 0.015 | 0.947 |
| | 0.281 | 232 | 36 | 0.010 | 0.017 | 0.895 | 0.002 | 0.014 | 0.943 | 0.000 | 0.014 | 0.939 |
| | 0.281 | 465 | 10 | 0.027 | 0.029 | 0.248 | 0.013 | 0.017 | 0.776 | 0.009 | 0.015 | 0.878 |
| | 0.281 | 465 | 18 | 0.018 | 0.020 | 0.574 | 0.007 | 0.012 | 0.906 | 0.002 | 0.011 | 0.950 |
| | 0.281 | 465 | 36 | 0.010 | 0.014 | 0.826 | 0.003 | 0.010 | 0.948 | 0.000 | 0.010 | 0.943 |
| | 0.281 | 930 | 10 | 0.027 | 0.028 | 0.033 | 0.013 | 0.015 | 0.587 | 0.009 | 0.012 | 0.801 |
| | 0.281 | 930 | 18 | 0.018 | 0.019 | 0.281 | 0.006 | 0.010 | 0.867 | 0.001 | 0.008 | 0.945 |
| | 0.281 | 930 | 36 | 0.010 | 0.012 | 0.688 | 0.002 | 0.007 | 0.941 | 0.000 | 0.007 | 0.950 |
| $\mu$ 25%Q | 2.786 | 232 | 10 | −0.016 | 0.032 | 0.907 | −0.007 | 0.034 | 0.960 | −0.004 | 0.050 | 0.993 |
| | 2.786 | 232 | 18 | −0.011 | 0.029 | 0.933 | −0.003 | 0.032 | 0.961 | 0.000 | 0.047 | 0.992 |
| | 2.786 | 232 | 36 | −0.005 | 0.026 | 0.947 | 0.000 | 0.030 | 0.966 | 0.002 | 0.043 | 0.993 |
| | 2.786 | 465 | 10 | −0.017 | 0.026 | 0.856 | −0.008 | 0.025 | 0.950 | −0.005 | 0.036 | 0.986 |
| | 2.786 | 465 | 18 | −0.011 | 0.022 | 0.910 | −0.003 | 0.023 | 0.957 | −0.001 | 0.034 | 0.989 |
| | 2.786 | 465 | 36 | −0.006 | 0.020 | 0.937 | −0.001 | 0.022 | 0.956 | 0.001 | 0.031 | 0.988 |
| | 2.786 | 930 | 10 | −0.017 | 0.022 | 0.755 | −0.008 | 0.018 | 0.934 | −0.005 | 0.025 | 0.979 |
| | 2.786 | 930 | 18 | −0.011 | 0.017 | 0.869 | −0.003 | 0.016 | 0.954 | 0.000 | 0.024 | 0.984 |
| | 2.786 | 930 | 36 | −0.006 | 0.015 | 0.919 | −0.001 | 0.015 | 0.955 | 0.000 | 0.022 | 0.982 |
| $\mu$ 50%Q | 2.975 | 232 | 10 | −0.001 | 0.025 | 0.949 | 0.001 | 0.030 | 0.965 | 0.001 | 0.045 | 0.992 |
| | 2.975 | 232 | 18 | 0.000 | 0.024 | 0.949 | 0.001 | 0.029 | 0.964 | 0.001 | 0.042 | 0.990 |
| | 2.975 | 232 | 36 | 0.000 | 0.023 | 0.951 | 0.001 | 0.027 | 0.966 | 0.000 | 0.038 | 0.993 |
| | 2.975 | 465 | 10 | 0.000 | 0.018 | 0.947 | 0.001 | 0.022 | 0.960 | 0.001 | 0.033 | 0.986 |
| | 2.975 | 465 | 18 | 0.000 | 0.017 | 0.948 | 0.001 | 0.020 | 0.962 | 0.001 | 0.030 | 0.988 |
| | 2.975 | 465 | 36 | 0.000 | 0.017 | 0.947 | 0.000 | 0.020 | 0.958 | 0.001 | 0.028 | 0.990 |
| | 2.975 | 930 | 10 | −0.001 | 0.013 | 0.947 | 0.001 | 0.015 | 0.957 | 0.001 | 0.023 | 0.979 |
| | 2.975 | 930 | 18 | 0.000 | 0.012 | 0.953 | 0.001 | 0.015 | 0.957 | 0.001 | 0.022 | 0.979 |
| | 2.975 | 930 | 36 | 0.000 | 0.012 | 0.949 | 0.000 | 0.014 | 0.956 | 0.000 | 0.020 | 0.982 |
| $\mu$ 75%Q | 3.165 | 232 | 10 | 0.016 | 0.032 | 0.913 | 0.008 | 0.035 | 0.960 | 0.005 | 0.052 | 0.992 |
| | 3.165 | 232 | 18 | 0.010 | 0.028 | 0.946 | 0.004 | 0.031 | 0.968 | 0.000 | 0.047 | 0.995 |
| | 3.165 | 232 | 36 | 0.005 | 0.026 | 0.943 | 0.000 | 0.031 | 0.960 | −0.001 | 0.044 | 0.993 |
| | 3.165 | 465 | 10 | 0.016 | 0.026 | 0.866 | 0.009 | 0.025 | 0.947 | 0.006 | 0.037 | 0.986 |
| | 3.165 | 465 | 18 | 0.011 | 0.022 | 0.912 | 0.004 | 0.023 | 0.962 | 0.001 | 0.034 | 0.989 |
| | 3.165 | 465 | 36 | 0.006 | 0.019 | 0.943 | 0.001 | 0.021 | 0.965 | 0.000 | 0.032 | 0.990 |
| | 3.165 | 930 | 10 | 0.017 | 0.022 | 0.770 | 0.009 | 0.019 | 0.928 | 0.007 | 0.027 | 0.978 |
| | 3.165 | 930 | 18 | 0.011 | 0.017 | 0.871 | 0.004 | 0.017 | 0.954 | 0.001 | 0.024 | 0.983 |
| | 3.165 | 930 | 36 | 0.006 | 0.014 | 0.928 | 0.002 | 0.015 | 0.959 | 0.000 | 0.022 | 0.985 |

Table S13: Monte Carlo simulation results for $\gamma_0$ in design 3

| | true | $N$ | $T$ | **ED** bias | **ED** rmse | **ED** cp | **HPJ** bias | **HPJ** rmse | **HPJ** cp | **TOJ** bias | **TOJ** rmse | **TOJ** cp |
|---|---|---|---|---|---|---|---|---|---|---|---|---|
| $\gamma_0$ mean | 0.048 | 232 | 10 | −0.016 | 0.016 | 0.000 | −0.007 | 0.008 | 0.300 | −0.005 | 0.006 | 0.705 |
| | 0.048 | 232 | 18 | −0.010 | 0.011 | 0.007 | −0.004 | 0.004 | 0.699 | −0.001 | 0.004 | 0.920 |
| | 0.048 | 232 | 36 | −0.006 | 0.006 | 0.194 | −0.001 | 0.003 | 0.900 | 0.000 | 0.003 | 0.939 |
| | 0.048 | 465 | 10 | −0.016 | 0.016 | 0.000 | −0.007 | 0.008 | 0.068 | −0.005 | 0.006 | 0.544 |
| | 0.048 | 465 | 18 | −0.010 | 0.010 | 0.000 | −0.004 | 0.004 | 0.506 | −0.001 | 0.003 | 0.924 |
| | 0.048 | 465 | 36 | −0.006 | 0.006 | 0.025 | −0.001 | 0.002 | 0.860 | 0.000 | 0.002 | 0.940 |
| | 0.048 | 930 | 10 | −0.016 | 0.016 | 0.000 | −0.007 | 0.007 | 0.001 | −0.005 | 0.006 | 0.294 |
| | 0.048 | 930 | 18 | −0.010 | 0.010 | 0.000 | −0.004 | 0.004 | 0.246 | −0.001 | 0.002 | 0.915 |
| | 0.048 | 930 | 36 | −0.006 | 0.006 | 0.000 | −0.001 | 0.002 | 0.780 | 0.000 | 0.001 | 0.949 |
| $\gamma_0$ std | 0.028 | 232 | 10 | 0.002 | 0.004 | 0.899 | 0.005 | 0.007 | 0.815 | 0.004 | 0.009 | 0.924 |
| | 0.028 | 232 | 18 | 0.003 | 0.004 | 0.813 | 0.004 | 0.005 | 0.842 | 0.003 | 0.007 | 0.923 |
| | 0.028 | 232 | 36 | 0.002 | 0.003 | 0.821 | 0.002 | 0.003 | 0.916 | 0.001 | 0.005 | 0.929 |
| | 0.028 | 465 | 10 | 0.003 | 0.003 | 0.806 | 0.005 | 0.006 | 0.618 | 0.004 | 0.007 | 0.908 |
| | 0.028 | 465 | 18 | 0.003 | 0.004 | 0.621 | 0.004 | 0.005 | 0.685 | 0.003 | 0.005 | 0.921 |
| | 0.028 | 465 | 36 | 0.002 | 0.003 | 0.612 | 0.002 | 0.003 | 0.842 | 0.001 | 0.003 | 0.936 |
| | 0.028 | 930 | 10 | 0.003 | 0.003 | 0.610 | 0.005 | 0.006 | 0.305 | 0.004 | 0.006 | 0.873 |
| | 0.028 | 930 | 18 | 0.003 | 0.003 | 0.317 | 0.004 | 0.004 | 0.403 | 0.003 | 0.004 | 0.889 |
| | 0.028 | 930 | 36 | 0.002 | 0.003 | 0.317 | 0.002 | 0.002 | 0.697 | 0.001 | 0.002 | 0.939 |
| $\gamma_0$ 25%Q | 0.027 | 232 | 10 | −0.015 | 0.016 | 0.000 | −0.010 | 0.010 | 0.013 | −0.007 | 0.008 | 0.467 |
| | 0.027 | 232 | 18 | −0.011 | 0.011 | 0.000 | −0.006 | 0.006 | 0.391 | −0.003 | 0.005 | 0.927 |
| | 0.027 | 232 | 36 | −0.007 | 0.007 | 0.069 | −0.003 | 0.004 | 0.842 | −0.001 | 0.004 | 0.978 |
| | 0.027 | 465 | 10 | −0.015 | 0.016 | 0.000 | −0.010 | 0.010 | 0.000 | −0.007 | 0.008 | 0.176 |
| | 0.027 | 465 | 18 | −0.011 | 0.011 | 0.000 | −0.006 | 0.006 | 0.109 | −0.003 | 0.004 | 0.854 |
| | 0.027 | 465 | 36 | −0.007 | 0.007 | 0.002 | −0.003 | 0.003 | 0.747 | −0.001 | 0.003 | 0.970 |
| | 0.027 | 930 | 10 | −0.016 | 0.016 | 0.000 | −0.010 | 0.010 | 0.000 | −0.007 | 0.008 | 0.012 |
| | 0.027 | 930 | 18 | −0.011 | 0.011 | 0.000 | −0.006 | 0.006 | 0.005 | −0.003 | 0.003 | 0.734 |
| | 0.027 | 930 | 36 | −0.007 | 0.007 | 0.000 | −0.003 | 0.003 | 0.510 | −0.001 | 0.002 | 0.961 |
| $\gamma_0$ 50%Q | 0.046 | 232 | 10 | −0.022 | 0.022 | 0.000 | −0.013 | 0.013 | 0.041 | −0.009 | 0.010 | 0.626 |
| | 0.046 | 232 | 18 | −0.015 | 0.015 | 0.000 | −0.007 | 0.008 | 0.478 | −0.003 | 0.006 | 0.946 |
| | 0.046 | 232 | 36 | −0.009 | 0.010 | 0.039 | −0.003 | 0.005 | 0.857 | −0.001 | 0.005 | 0.984 |
| | 0.046 | 465 | 10 | −0.022 | 0.022 | 0.000 | −0.013 | 0.013 | 0.000 | −0.009 | 0.010 | 0.336 |
| | 0.046 | 465 | 18 | −0.015 | 0.015 | 0.000 | −0.007 | 0.008 | 0.178 | −0.003 | 0.005 | 0.910 |
| | 0.046 | 465 | 36 | −0.009 | 0.009 | 0.001 | −0.003 | 0.004 | 0.756 | −0.001 | 0.004 | 0.973 |
| | 0.046 | 930 | 10 | −0.022 | 0.022 | 0.000 | −0.013 | 0.013 | 0.000 | −0.009 | 0.010 | 0.071 |
| | 0.046 | 930 | 18 | −0.015 | 0.015 | 0.000 | −0.007 | 0.007 | 0.021 | −0.003 | 0.004 | 0.850 |
| | 0.046 | 930 | 36 | −0.009 | 0.009 | 0.000 | −0.003 | 0.004 | 0.543 | −0.001 | 0.003 | 0.960 |
| $\gamma_0$ 75%Q | 0.067 | 232 | 10 | −0.023 | 0.023 | 0.000 | −0.010 | 0.012 | 0.540 | −0.007 | 0.012 | 0.900 |
| | 0.067 | 232 | 18 | −0.015 | 0.015 | 0.026 | −0.005 | 0.007 | 0.846 | −0.001 | 0.009 | 0.976 |
| | 0.067 | 232 | 36 | −0.008 | 0.009 | 0.296 | −0.002 | 0.005 | 0.941 | 0.000 | 0.008 | 0.984 |
| | 0.067 | 465 | 10 | −0.023 | 0.023 | 0.000 | −0.010 | 0.011 | 0.271 | −0.007 | 0.010 | 0.831 |
| | 0.067 | 465 | 18 | −0.015 | 0.015 | 0.000 | −0.005 | 0.006 | 0.736 | −0.001 | 0.006 | 0.969 |
| | 0.067 | 465 | 36 | −0.008 | 0.009 | 0.069 | −0.002 | 0.004 | 0.914 | 0.000 | 0.006 | 0.975 |
| | 0.067 | 930 | 10 | −0.023 | 0.023 | 0.000 | −0.010 | 0.011 | 0.054 | −0.007 | 0.009 | 0.681 |
| | 0.067 | 930 | 18 | −0.015 | 0.015 | 0.000 | −0.005 | 0.005 | 0.551 | −0.001 | 0.005 | 0.959 |
| | 0.067 | 930 | 36 | −0.008 | 0.008 | 0.002 | −0.002 | 0.003 | 0.880 | 0.000 | 0.004 | 0.974 |

Table S14: Monte Carlo simulation results for $\rho_1$ in design 3

| | true | $N$ | $T$ | **ED** bias | rmse | cp | **HPJ** bias | rmse | cp | **TOJ** bias | rmse | cp |
|---|---|---|---|---|---|---|---|---|---|---|---|---|
| $\rho_1$ mean | 0.563 | 232 | 10 | −0.304 | 0.304 | 0.000 | −0.009 | 0.035 | 0.938 | −0.147 | 0.161 | 0.426 |
| | 0.563 | 232 | 18 | −0.167 | 0.167 | 0.000 | 0.004 | 0.024 | 0.944 | 0.014 | 0.048 | 0.940 |
| | 0.563 | 232 | 36 | −0.081 | 0.082 | 0.000 | 0.005 | 0.018 | 0.938 | 0.004 | 0.028 | 0.943 |
| | 0.563 | 465 | 10 | −0.304 | 0.304 | 0.000 | −0.009 | 0.026 | 0.929 | −0.148 | 0.156 | 0.138 |
| | 0.563 | 465 | 18 | −0.167 | 0.167 | 0.000 | 0.004 | 0.017 | 0.941 | 0.014 | 0.035 | 0.922 |
| | 0.563 | 465 | 36 | −0.081 | 0.082 | 0.000 | 0.005 | 0.013 | 0.925 | 0.004 | 0.020 | 0.944 |
| | 0.563 | 930 | 10 | −0.304 | 0.304 | 0.000 | −0.010 | 0.020 | 0.903 | −0.149 | 0.152 | 0.009 |
| | 0.563 | 930 | 18 | −0.167 | 0.167 | 0.000 | 0.004 | 0.013 | 0.937 | 0.014 | 0.027 | 0.901 |
| | 0.563 | 930 | 36 | −0.081 | 0.081 | 0.000 | 0.005 | 0.010 | 0.907 | 0.004 | 0.014 | 0.935 |
| $\rho_1$ std | 0.181 | 232 | 10 | 0.133 | 0.133 | 0.000 | 0.068 | 0.073 | 0.251 | −0.076 | 0.093 | 0.694 |
| | 0.181 | 232 | 18 | 0.078 | 0.078 | 0.000 | 0.011 | 0.023 | 0.921 | −0.029 | 0.050 | 0.883 |
| | 0.181 | 232 | 36 | 0.037 | 0.038 | 0.026 | −0.003 | 0.015 | 0.933 | −0.009 | 0.028 | 0.930 |
| | 0.181 | 465 | 10 | 0.133 | 0.133 | 0.000 | 0.068 | 0.070 | 0.039 | −0.076 | 0.085 | 0.471 |
| | 0.181 | 465 | 18 | 0.078 | 0.078 | 0.000 | 0.011 | 0.018 | 0.882 | −0.029 | 0.041 | 0.828 |
| | 0.181 | 465 | 36 | 0.037 | 0.038 | 0.000 | −0.003 | 0.011 | 0.931 | −0.009 | 0.021 | 0.921 |
| | 0.181 | 930 | 10 | 0.133 | 0.133 | 0.000 | 0.068 | 0.069 | 0.001 | −0.076 | 0.081 | 0.185 |
| | 0.181 | 930 | 18 | 0.078 | 0.078 | 0.000 | 0.011 | 0.015 | 0.805 | −0.029 | 0.035 | 0.704 |
| | 0.181 | 930 | 36 | 0.038 | 0.038 | 0.000 | −0.002 | 0.008 | 0.931 | −0.008 | 0.016 | 0.902 |
| $\rho_1$ 25%Q | 0.440 | 232 | 10 | −0.390 | 0.391 | 0.000 | −0.035 | 0.070 | 0.925 | −0.174 | 0.223 | 0.783 |
| | 0.440 | 232 | 18 | −0.213 | 0.215 | 0.000 | 0.007 | 0.046 | 0.958 | 0.031 | 0.103 | 0.963 |
| | 0.440 | 232 | 36 | −0.101 | 0.104 | 0.001 | 0.010 | 0.035 | 0.949 | 0.010 | 0.068 | 0.977 |
| | 0.440 | 465 | 10 | −0.390 | 0.391 | 0.000 | −0.036 | 0.055 | 0.877 | −0.178 | 0.203 | 0.576 |
| | 0.440 | 465 | 18 | −0.214 | 0.215 | 0.000 | 0.007 | 0.033 | 0.957 | 0.031 | 0.076 | 0.947 |
| | 0.440 | 465 | 36 | −0.102 | 0.103 | 0.000 | 0.010 | 0.026 | 0.935 | 0.009 | 0.049 | 0.972 |
| | 0.440 | 930 | 10 | −0.391 | 0.392 | 0.000 | −0.037 | 0.048 | 0.773 | −0.180 | 0.192 | 0.264 |
| | 0.440 | 930 | 18 | −0.214 | 0.214 | 0.000 | 0.007 | 0.023 | 0.948 | 0.031 | 0.057 | 0.916 |
| | 0.440 | 930 | 36 | −0.102 | 0.103 | 0.000 | 0.010 | 0.019 | 0.916 | 0.010 | 0.035 | 0.964 |
| $\rho_1$ 50%Q | 0.566 | 232 | 10 | −0.278 | 0.279 | 0.000 | 0.009 | 0.051 | 0.948 | −0.081 | 0.137 | 0.916 |
| | 0.566 | 232 | 18 | −0.146 | 0.148 | 0.000 | 0.017 | 0.041 | 0.942 | 0.024 | 0.085 | 0.962 |
| | 0.566 | 232 | 36 | −0.069 | 0.071 | 0.036 | 0.009 | 0.029 | 0.953 | 0.003 | 0.056 | 0.979 |
| | 0.566 | 465 | 10 | −0.277 | 0.278 | 0.000 | 0.010 | 0.037 | 0.942 | −0.081 | 0.114 | 0.846 |
| | 0.566 | 465 | 18 | −0.147 | 0.147 | 0.000 | 0.017 | 0.032 | 0.909 | 0.024 | 0.063 | 0.943 |
| | 0.566 | 465 | 36 | −0.068 | 0.070 | 0.000 | 0.010 | 0.022 | 0.929 | 0.004 | 0.039 | 0.973 |
| | 0.566 | 930 | 10 | −0.278 | 0.278 | 0.000 | 0.008 | 0.027 | 0.939 | −0.083 | 0.101 | 0.706 |
| | 0.566 | 930 | 18 | −0.147 | 0.147 | 0.000 | 0.017 | 0.025 | 0.863 | 0.025 | 0.048 | 0.923 |
| | 0.566 | 930 | 36 | −0.068 | 0.069 | 0.000 | 0.010 | 0.017 | 0.897 | 0.005 | 0.028 | 0.964 |
| $\rho_1$ 75%Q | 0.690 | 232 | 10 | −0.192 | 0.194 | 0.000 | 0.042 | 0.064 | 0.878 | −0.133 | 0.172 | 0.803 |
| | 0.690 | 232 | 18 | −0.101 | 0.103 | 0.001 | 0.014 | 0.039 | 0.956 | −0.012 | 0.079 | 0.970 |
| | 0.690 | 232 | 36 | −0.048 | 0.052 | 0.224 | 0.004 | 0.028 | 0.960 | −0.002 | 0.056 | 0.975 |
| | 0.690 | 465 | 10 | −0.191 | 0.192 | 0.000 | 0.041 | 0.053 | 0.793 | −0.136 | 0.156 | 0.614 |
| | 0.690 | 465 | 18 | −0.100 | 0.101 | 0.000 | 0.014 | 0.029 | 0.928 | −0.012 | 0.056 | 0.962 |
| | 0.690 | 465 | 36 | −0.047 | 0.049 | 0.040 | 0.005 | 0.021 | 0.949 | 0.000 | 0.040 | 0.968 |
| | 0.690 | 930 | 10 | −0.191 | 0.192 | 0.000 | 0.041 | 0.048 | 0.605 | −0.135 | 0.146 | 0.332 |
| | 0.690 | 930 | 18 | −0.100 | 0.101 | 0.000 | 0.015 | 0.023 | 0.889 | −0.011 | 0.040 | 0.957 |
| | 0.690 | 930 | 36 | −0.047 | 0.048 | 0.000 | 0.006 | 0.015 | 0.939 | 0.001 | 0.028 | 0.970 |

Table S15: Monte Carlo simulation results for correlations in design 3

| | true | $N$ | $T$ | **ED** bias | rmse | cp | **HPJ** bias | rmse | cp | **TOJ** bias | rmse | cp |
|---|---|---|---|---|---|---|---|---|---|---|---|---|
| $\mu$ vs $\gamma_0$ | 0.216 | 232 | 10 | −0.052 | 0.084 | 0.862 | −0.029 | 0.097 | 0.928 | −0.029 | 0.148 | 0.935 |
| | 0.216 | 232 | 18 | −0.034 | 0.073 | 0.905 | −0.016 | 0.086 | 0.937 | −0.008 | 0.123 | 0.945 |
| | 0.216 | 232 | 36 | −0.021 | 0.070 | 0.927 | −0.007 | 0.080 | 0.934 | −0.002 | 0.105 | 0.936 |
| | 0.216 | 465 | 10 | −0.051 | 0.069 | 0.794 | −0.027 | 0.070 | 0.925 | −0.029 | 0.104 | 0.941 |
| | 0.216 | 465 | 18 | −0.036 | 0.058 | 0.875 | −0.018 | 0.062 | 0.934 | −0.011 | 0.088 | 0.948 |
| | 0.216 | 465 | 36 | −0.022 | 0.050 | 0.920 | −0.008 | 0.055 | 0.944 | −0.002 | 0.072 | 0.940 |
| | 0.216 | 930 | 10 | −0.051 | 0.061 | 0.657 | −0.027 | 0.053 | 0.904 | −0.027 | 0.077 | 0.928 |
| | 0.216 | 930 | 18 | −0.036 | 0.049 | 0.786 | −0.017 | 0.047 | 0.918 | −0.010 | 0.064 | 0.940 |
| | 0.216 | 930 | 36 | −0.022 | 0.039 | 0.889 | −0.008 | 0.040 | 0.940 | −0.003 | 0.051 | 0.945 |
| $\mu$ vs $\rho_1$ | −0.221 | 232 | 10 | 0.150 | 0.164 | 0.353 | 0.111 | 0.158 | 0.820 | 0.078 | 0.225 | 0.927 |
| | −0.221 | 232 | 18 | 0.111 | 0.129 | 0.582 | 0.063 | 0.117 | 0.899 | 0.025 | 0.170 | 0.944 |
| | −0.221 | 232 | 36 | 0.065 | 0.091 | 0.828 | 0.020 | 0.088 | 0.940 | −0.005 | 0.128 | 0.943 |
| | −0.221 | 465 | 10 | 0.152 | 0.159 | 0.085 | 0.112 | 0.137 | 0.694 | 0.078 | 0.167 | 0.908 |
| | −0.221 | 465 | 18 | 0.109 | 0.119 | 0.327 | 0.060 | 0.092 | 0.867 | 0.018 | 0.119 | 0.947 |
| | −0.221 | 465 | 36 | 0.065 | 0.079 | 0.692 | 0.019 | 0.063 | 0.940 | −0.005 | 0.089 | 0.950 |
| | −0.221 | 930 | 10 | 0.153 | 0.156 | 0.003 | 0.114 | 0.127 | 0.461 | 0.081 | 0.133 | 0.874 |
| | −0.221 | 930 | 18 | 0.109 | 0.114 | 0.077 | 0.059 | 0.078 | 0.769 | 0.019 | 0.088 | 0.940 |
| | −0.221 | 930 | 36 | 0.065 | 0.072 | 0.465 | 0.019 | 0.047 | 0.924 | −0.005 | 0.064 | 0.946 |
| $\gamma_0$ vs $\rho_1$ | −0.102 | 232 | 10 | 0.278 | 0.284 | 0.015 | 0.282 | 0.301 | 0.251 | 0.198 | 0.273 | 0.824 |
| | −0.102 | 232 | 18 | 0.225 | 0.234 | 0.088 | 0.169 | 0.196 | 0.618 | 0.083 | 0.188 | 0.922 |
| | −0.102 | 232 | 36 | 0.141 | 0.157 | 0.455 | 0.057 | 0.111 | 0.905 | −0.011 | 0.144 | 0.940 |
| | −0.102 | 465 | 10 | 0.277 | 0.280 | 0.000 | 0.282 | 0.291 | 0.041 | 0.198 | 0.239 | 0.687 |
| | −0.102 | 465 | 18 | 0.227 | 0.232 | 0.003 | 0.172 | 0.187 | 0.342 | 0.087 | 0.148 | 0.885 |
| | −0.102 | 465 | 36 | 0.143 | 0.151 | 0.158 | 0.058 | 0.089 | 0.862 | −0.011 | 0.099 | 0.945 |
| | −0.102 | 930 | 10 | 0.278 | 0.280 | 0.000 | 0.285 | 0.289 | 0.000 | 0.203 | 0.223 | 0.421 |
| | −0.102 | 930 | 18 | 0.227 | 0.229 | 0.000 | 0.171 | 0.178 | 0.086 | 0.084 | 0.119 | 0.823 |
| | −0.102 | 930 | 36 | 0.142 | 0.146 | 0.014 | 0.058 | 0.075 | 0.773 | −0.010 | 0.072 | 0.944 |

# References


D. Ackerberg, C. L. Benkard, S. Berry, and A. Pakes. Econometric tools for analyzing market outcomes. *Handbook of econometrics*, 6:4171–4276, 2007.

D. Ackerberg, K. Caves, and G. Frazer. Identification properties of recent production function estimators. *Econometrica*, 83(6):2411–2451, 2015.

J. Balat, I. Brambilla, and Y. Sasaki. Heterogeneous firms: Skilled-labor productivity and the destination of exports. mimeo, 2016.

I. Botosaru and Y. Sasaki. Nonparametric heteroskedasticity in persistent panel processes: An application to earnings dynamics. *Journal of Econometrics*, 203:283–296, 2018.

M. Browning, M. Ejrnæs, and J. Alvarez. Modelling income processes with lots of heterogeneity. *Rview of Economic Studies*, 77:1353–1381, 2010.

G. Cheng and J. Huang. Bootstrap consistency for general semiparametric $m$-estimation. *Annals of Statistics*, 38:2884–2915, 2010.

V. Chernozhukov, I. Fernandez-Val, and A. Galichon. Improving point and interval estimators of monotone functions by rearrangement. *Biometrika*, 96(3):559–575, 2009.

M. J. Crucini, M. Shintani, and T. Tsuruga. Noisy information, distance and law of one price dynamics across us cities. *Journal of Monetary Economics*, 74:52–66, 2015.

G. Dhaene and K. Jochmans. Split-panel jackknife estimation of fixed effects models. *Review of Economic Studies*, 82:991–1030, 2015.

M. Ejrnæs and M. Browning. The persistent-transitory representation for earnings processes. *Quantitative Economics*, 5(3):555–581, 2014.

C. Feng, H. Wang, T. Chen, and X. M. Tu. On exact forms of Taylor's theorem for vector-valued functions. *Biometrika*, 101(4):1003–1003, 2014.

A. Gandhi, S. Navarro, and D. A. Rivers. On the identification of production functions: How heterogeneous is productivity? mimeo, 2016.

Z. Griliches and J. Mairesse. Production functions: the search for identification. *Econometrics and Economic Theory in the 20th Century: The Ragnar Frisch Centennial Symposium*, pages 169–203, 1998.

J. L. Horowitz and M. Markatou. Semiparametric estimation of regression models for panel data. *Review of Economic Studies*, 63(1):145–168, 1996.

L. Hospido. Modelling heterogeneity and dynamics in the volatility of individual wages. *Journal of Applied Econometrics*, 27:386–414, 2012.

C. Hsiao, M. H. Pesaran, and A. K. Tahmiscioglu. Bayes estimation of short-run coefficients in dynamic panel data models. In K. L. C. Hsiao, L.F. Lee and M. Pesaran, editors, *Analysis of Panels and Limited Dependent Variables Models*, pages 268–296. Cambridge University press, 1999.

A. N. Kolmogorov. Sulla determinazione empirica di una legge di distribuzione. *Giornale dell'Istituto Italiano degli Attuari*, 4:83–91, 1933.

J. Levinsohn and A. Petrin. Estimating production functions using inputs to control for unobservables. *Review of Economic Studies*, 70(2):317–341, 2003.

C. Meghir and L. Pistaferri. Income variance dynamics and heterogeneity. *Econometrica*, 72(1): 1–32, 2004.

C. Meghir and L. Pistaferri. Earnings, consumption and life cycle choices. *Handbook of Labor Economics*, 4:773–854, 2011.

R. Okui. Asymptotically unbiased estimation of autocovariances and autocorrelations with long panel data. *Econometric Theory*, 26:1263–1304, 2010.

R. Okui. Asymptotically unbiased estimation of autocovariances and autocorrelations with panel data in the presence of individual and time effects. *Journal of Time Series Econometrics*, 6(2): 129–181, 2014.

P. C. B. Phillips and H. R. Moon. Linear regression limit theory for nonstationary panel data. *Econometrica*, 67(5):1057–1111, 1999.

M. H. Quenouille. Approximate tests of correlation in time-series 3. In *Mathematical Proceedings of the Cambridge Philosophical Society*, volume 45-03, pages 483–484. Cambridge Univ Press, 1949.

M. H. Quenouille. Notes on bias in estimation. *Biometrika*, 43(3 and 4):353–360, 1956.

N. V. Smirnov. Approximate laws of distribution of random variables from empirical data. *Uspekhi Matematicheskikh Nauk*, 10:179–206, 1944.

A. W. van der Vaart. *Asymptotic Statistics.* Cambridge University Press, 1998.

R. Yokoyama. Moment bounds for stationary mixing sequences. *Zeitschrift für Wahrscheinlichkeitstheorie und verwandte Gebiete*, 52(1):45–57, 1980.
